# Supplementary material for: ALICE: An Advanced Logic for Interactive Component Engineering
Source: arXiv:1410.4381 source file (2014-10-16)
Supplement: Supplementary file 1 [file appendix.tex]

\section{Types}
Firstly, a theory introducing the necessary types is created as follows.
\begin{isabellebody}%
\isadelimtheory
\endisadelimtheory
\isatagtheory
\isacommand{theory}\isamarkupfalse%
\ ABPTypes\isanewline
\isakeyword{imports}\ ALICE\isanewline
\isakeyword{begin}%
\endisatagtheory
{\isafoldtheory}%
\isadelimtheory
\isanewline
\endisadelimtheory
\isanewline
\isacommand{typedecl}\isamarkupfalse%
\ Data\ %
\isamarkupcmt{a generic type for data%
}
\isanewline
\isacommand{types}\isamarkupfalse%
\ Bit\ {\isacharequal}\ bool%
\begin{isamarkuptext}%
By the latter type declaration in HOL, we take {\pisastyle{Bit}} as a type alias 
for the HOL type {\pisastyle{bool}}.%
\end{isamarkuptext}%
\isamarkuptrue%
\isadelimtheory
\endisadelimtheory
\isatagtheory
\isacommand{end}\isamarkupfalse%
\endisatagtheory
{\isafoldtheory}%
\isadelimtheory
\endisadelimtheory
\isanewline
\end{isabellebody}%
%%% Local Variables:
%%% mode: latex
%%% TeX-master: "root"
%%% End:

%
\section{Sender} \label{ABP_Sender}
We translate the above specification into the following \alice theory.
\begin{isabellebody}%
\isadelimtheory
\endisadelimtheory
\isatagtheory
\isacommand{theory}\isamarkupfalse%
\ Sender\isanewline
\isakeyword{imports}\ ABPTypes\isanewline
\isakeyword{begin}%
\endisatagtheory
{\isafoldtheory}%
\isadelimtheory
\isanewline
\endisadelimtheory
\isanewline
\isacommand{constdefs}\isamarkupfalse%
\isanewline
\ \ Snd\ {\isacharcolon}{\isacharcolon}\ {\isachardoublequoteopen}Data\ fstream\ {\isasymRightarrow}\ Bit\ fstream\ {\isasymRightarrow}\ {\isacharparenleft}Data\ {\isacharasterisk}\ Bit{\isacharparenright}\ fstream\ {\isasymRightarrow}\ bool{\isachardoublequoteclose}\isanewline
\ \ Snd{\isacharunderscore}def{\isacharcolon}\ \isanewline
\ \ \ \ {\isachardoublequoteopen}Snd\ i\ as\ ds\ {\isasymequiv}\ \isanewline
\ \ \ \ \ \ \ let\ \isanewline
\ \ \ \ \ \ \ \ \ \ fas\ {\isacharequal}\ fnub{\isasymcdot}as{\isacharsemicolon}\ \isanewline
\ \ \ \ \ \ \ \ \ \ fb\ {\isacharequal}\ fproj{\isadigit{2}}{\isasymcdot}{\isacharparenleft}fnub{\isasymcdot}ds{\isacharparenright}{\isacharsemicolon}\isanewline
\ \ \ \ \ \ \ \ \ \ fds\ {\isacharequal}\ fproj{\isadigit{1}}{\isasymcdot}{\isacharparenleft}fnub{\isasymcdot}ds{\isacharparenright}\ \isanewline
\ \ \ \ \ \ \ in\ \isanewline
\ \ \ \ \ \ \ \ \ \ fds\ {\isasymsqsubseteq}\ i\ {\isasymand}\ \ \isanewline
\ \ \ \ \ \ \ \ \ \ fnub{\isasymcdot}fb\ {\isacharequal}\ fb\ {\isasymand}\ \ \isanewline
\ \ \ \ \ \ \ \ \ \ {\isacharhash}fds\ {\isacharequal}\ imin\ {\isacharhash}i\ {\isacharparenleft}iSuc\ {\isacharparenleft}{\isacharhash}fas{\isacharparenright}{\isacharparenright}\ {\isasymand}\ \isanewline
\ \ \ \ \ \ \ \ \ \ {\isacharparenleft}{\isacharhash}fas\ {\isacharless}\ {\isacharhash}i\ {\isasymlongrightarrow}\ \isanewline
\ \ \ \ \ \ \ \ \ \ \ \ \ \ \ \ \ \ \ \ \ \ {\isacharhash}ds\ {\isacharequal}\ {\isasyminfinity}\ {\isasymand}\ \isanewline
\ \ \ \ \ \ \ \ \ \ \ \ \ \ \ \ \ \ \ \ \ \ {\isacharparenleft}ftake\ {\isacharparenleft}THE\ k{\isachardot}\ {\isacharhash}{\isacharparenleft}fnub{\isasymcdot}as{\isacharparenright}\ {\isacharequal}\ Fin\ k{\isacharparenright}{\isasymcdot}fb\ {\isacharequal}\ fas{\isacharparenright}{\isacharparenright}{\isachardoublequoteclose}\isanewline
\isanewline
\isacommand{lemma}\isamarkupfalse%
\ SndD{\isadigit{1}}{\isacharcolon}\ \isanewline
\ \ {\isachardoublequoteopen}Snd\ i\ as\ ds\ {\isasymLongrightarrow}\ fproj{\isadigit{1}}{\isasymcdot}{\isacharparenleft}fnub{\isasymcdot}ds{\isacharparenright}\ {\isasymsqsubseteq}\ i{\isachardoublequoteclose}\isanewline
\isadelimproof
\endisadelimproof
\isatagproof
\isacommand{by}\isamarkupfalse%
\ {\isacharparenleft}simp\ add{\isacharcolon}\ Snd{\isacharunderscore}def\ Let{\isacharunderscore}def{\isacharparenright}%
\endisatagproof
{\isafoldproof}%
\isadelimproof
\isanewline
\endisadelimproof
\isanewline
\isacommand{lemma}\isamarkupfalse%
\ SndD{\isadigit{2}}{\isacharcolon}\ \isanewline
\ \ {\isachardoublequoteopen}Snd\ i\ as\ ds\ {\isasymLongrightarrow}\ {\isacharhash}{\isacharparenleft}fproj{\isadigit{1}}{\isasymcdot}{\isacharparenleft}fnub{\isasymcdot}ds{\isacharparenright}{\isacharparenright}\ {\isacharequal}\ imin\ {\isacharhash}i\ {\isacharparenleft}iSuc\ {\isacharhash}{\isacharparenleft}fnub{\isasymcdot}as{\isacharparenright}{\isacharparenright}{\isachardoublequoteclose}\isanewline
\isadelimproof
\endisadelimproof
\isatagproof
\isacommand{by}\isamarkupfalse%
\ {\isacharparenleft}simp\ add{\isacharcolon}\ Snd{\isacharunderscore}def\ Let{\isacharunderscore}def{\isacharparenright}%
\endisatagproof
{\isafoldproof}%
\isadelimproof
\isanewline
\endisadelimproof
\isanewline
\isacommand{lemma}\isamarkupfalse%
\ Snd{\isacharunderscore}epsilon{\isacharunderscore}all{\isacharbrackleft}simp{\isacharbrackright}{\isacharcolon}\ \isanewline
\ \ {\isachardoublequoteopen}Snd\ {\isasymepsilon}\ {\isasymepsilon}\ {\isasymepsilon}{\isachardoublequoteclose}\isanewline
\isadelimproof
\endisadelimproof
\isatagproof
\isacommand{by}\isamarkupfalse%
\ {\isacharparenleft}auto\ simp\ add{\isacharcolon}\ Snd{\isacharunderscore}def\ Let{\isacharunderscore}def{\isacharparenright}%
\endisatagproof
{\isafoldproof}%
\isadelimproof
\isanewline
\endisadelimproof
\isanewline
\isacommand{lemma}\isamarkupfalse%
\ mixed{\isacharunderscore}fnub{\isacharunderscore}fproj{\isadigit{2}}{\isacharbrackleft}simp{\isacharbrackright}{\isacharcolon}\ \isanewline
\ \ {\isachardoublequoteopen}fnub{\isasymcdot}{\isacharparenleft}fproj{\isadigit{2}}{\isasymcdot}{\isacharparenleft}fnub{\isasymcdot}x{\isacharparenright}{\isacharparenright}\ {\isacharequal}\ fnub{\isasymcdot}{\isacharparenleft}fproj{\isadigit{2}}{\isasymcdot}x{\isacharparenright}{\isachardoublequoteclose}\isanewline
\isadelimproof
\endisadelimproof
\isatagproof
\isacommand{apply}\isamarkupfalse%
\ {\isacharparenleft}rule\ fstream{\isacharunderscore}ind{\isadigit{1}}\ {\isacharbrackleft}of\ {\isacharunderscore}\ {\isachardoublequoteopen}x{\isachardoublequoteclose}{\isacharbrackright}{\isacharcomma}\ auto{\isacharparenright}\isanewline
\isacommand{apply}\isamarkupfalse%
\ {\isacharparenleft}case{\isacharunderscore}tac\ {\isachardoublequoteopen}s\ {\isacharequal}\ {\isasymepsilon}{\isachardoublequoteclose}{\isacharcomma}\ auto{\isacharparenright}\isanewline
\isacommand{apply}\isamarkupfalse%
\ {\isacharparenleft}drule\ fscase{\isadigit{2}}{\isacharcomma}\ auto{\isacharparenright}\isanewline
\isacommand{apply}\isamarkupfalse%
\ {\isacharparenleft}case{\isacharunderscore}tac\ {\isachardoublequoteopen}{\isacharparenleft}a{\isacharcomma}b{\isacharparenright}\ {\isacharequal}\ {\isacharparenleft}aa{\isacharcomma}ba{\isacharparenright}{\isachardoublequoteclose}{\isacharcomma}\ auto{\isacharparenright}\isanewline
\isacommand{apply}\isamarkupfalse%
\ {\isacharparenleft}insert\ fnub{\isacharunderscore}exhaust{\isacharcomma}\ atomize{\isacharparenright}\isanewline
\isacommand{apply}\isamarkupfalse%
\ {\isacharparenleft}erule{\isacharunderscore}tac\ x{\isacharequal}{\isachardoublequoteopen}{\isacharparenleft}aa{\isacharcomma}ba{\isacharparenright}{\isachardoublequoteclose}\isakeyword{in}\ allE{\isacharparenright}\isanewline
\isacommand{apply}\isamarkupfalse%
\ {\isacharparenleft}erule{\isacharunderscore}tac\ x{\isacharequal}{\isachardoublequoteopen}rs{\isachardoublequoteclose}\ \isakeyword{in}\ allE{\isacharcomma}\ auto{\isacharparenright}\isanewline
\isacommand{apply}\isamarkupfalse%
\ {\isacharparenleft}case{\isacharunderscore}tac\ {\isachardoublequoteopen}b{\isacharequal}ba{\isachardoublequoteclose}{\isacharcomma}\ auto{\isacharparenright}\isanewline
\isacommand{apply}\isamarkupfalse%
\ atomize\isanewline
\isacommand{apply}\isamarkupfalse%
\ {\isacharparenleft}erule{\isacharunderscore}tac\ x{\isacharequal}{\isachardoublequoteopen}{\isacharparenleft}aa{\isacharcomma}ba{\isacharparenright}{\isachardoublequoteclose}\ \isakeyword{in}\ allE{\isacharparenright}\isanewline
\isacommand{by}\isamarkupfalse%
\ {\isacharparenleft}erule{\isacharunderscore}tac\ x{\isacharequal}{\isachardoublequoteopen}rs{\isachardoublequoteclose}\ \isakeyword{in}\ allE{\isacharcomma}\ auto{\isacharparenright}%
\endisatagproof
{\isafoldproof}%
\isadelimproof
\isanewline
\endisadelimproof
\isanewline
\isacommand{lemma}\isamarkupfalse%
\ alt{\isacharunderscore}Snd{\isacharunderscore}lemma{\isacharcolon}\ \isanewline
\ \ {\isachardoublequoteopen}Snd\ i\ as\ ds\ {\isasymLongrightarrow}\ fproj{\isadigit{2}}{\isasymcdot}{\isacharparenleft}fnub{\isasymcdot}ds{\isacharparenright}\ {\isacharequal}\ fnub{\isasymcdot}{\isacharparenleft}fproj{\isadigit{2}}{\isasymcdot}ds{\isacharparenright}{\isachardoublequoteclose}\isanewline
\isadelimproof
\endisadelimproof
\isatagproof
\isacommand{by}\isamarkupfalse%
\ {\isacharparenleft}simp\ add{\isacharcolon}\ Snd{\isacharunderscore}def\ Let{\isacharunderscore}def{\isacharparenright}%
\endisatagproof
{\isafoldproof}%
\isadelimproof
\isanewline
\endisadelimproof
\isanewline
\isacommand{lemma}\isamarkupfalse%
\ send{\isacharunderscore}Snd{\isacharunderscore}lemma{\isacharcolon}\ \isanewline
\ \ {\isachardoublequoteopen}Snd\ i\ as\ ds\ {\isasymLongrightarrow}\ {\isacharhash}{\isacharparenleft}fnub{\isasymcdot}ds{\isacharparenright}\ {\isasymle}\ {\isacharhash}i{\isachardoublequoteclose}\isanewline
\isadelimproof
\endisadelimproof
\isatagproof
\isacommand{apply}\isamarkupfalse%
\ {\isacharparenleft}drule\ SndD{\isadigit{1}}{\isacharcomma}\ drule\ fslen{\isacharunderscore}mono{\isacharparenright}\isanewline
\isacommand{by}\isamarkupfalse%
\ {\isacharparenleft}simp\ add{\isacharcolon}\ fproj{\isadigit{1}}{\isacharunderscore}fslen{\isacharparenright}%
\endisatagproof
{\isafoldproof}%
\isadelimproof
\isanewline
\endisadelimproof
\isanewline
\isacommand{lemma}\isamarkupfalse%
\ ack{\isacharunderscore}Snd{\isacharunderscore}lemma{\isacharcolon}\ \isanewline
\ \ {\isachardoublequoteopen}Snd\ i\ as\ ds\ {\isasymLongrightarrow}\ {\isacharparenleft}{\isacharhash}{\isacharparenleft}fnub{\isasymcdot}as{\isacharparenright}\ {\isacharless}\ {\isacharhash}i{\isacharparenright}\ {\isasymor}\ {\isacharparenleft}{\isacharhash}{\isacharparenleft}fnub{\isasymcdot}ds{\isacharparenright}\ {\isacharequal}\ {\isacharhash}i{\isacharparenright}{\isachardoublequoteclose}\isanewline
\isadelimproof
\endisadelimproof
\isatagproof
\isacommand{apply}\isamarkupfalse%
\ {\isacharparenleft}frule\ SndD{\isadigit{2}}{\isacharcomma}\ auto{\isacharparenright}\isanewline
\isacommand{apply}\isamarkupfalse%
\ {\isacharparenleft}drule\ send{\isacharunderscore}Snd{\isacharunderscore}lemma{\isacharparenright}\isanewline
\isacommand{apply}\isamarkupfalse%
\ {\isacharparenleft}simp\ add{\isacharcolon}\ fproj{\isadigit{1}}{\isacharunderscore}fslen{\isacharparenright}\isanewline
\isacommand{by}\isamarkupfalse%
\ {\isacharparenleft}simp\ add{\isacharcolon}\ imin{\isacharunderscore}def\ inat{\isacharunderscore}defs\ split{\isacharcolon}\ inat{\isacharunderscore}splits{\isacharcomma}\ arith{\isacharquery}{\isacharparenright}%
\endisatagproof
{\isafoldproof}%
\isadelimproof
\isanewline
\endisadelimproof
\isadelimtheory
\isanewline
\endisadelimtheory
\isatagtheory
\isacommand{end}\isamarkupfalse%
\endisatagtheory
{\isafoldtheory}%
\isadelimtheory
\isanewline
\endisadelimtheory
\isanewline
\end{isabellebody}%
%%% Local Variables:
%%% mode: latex
%%% TeX-master: "root"
%%% End:

%
\section{Media} \label{ABP_Media}
\begin{isabellebody}%
\isadelimtheory
\endisadelimtheory
\isatagtheory
\isacommand{theory}\isamarkupfalse%
\ Medium\isanewline
\isakeyword{imports}\ ABPTypes\isanewline
\isakeyword{begin}%
\endisatagtheory
{\isafoldtheory}%
\isadelimtheory
\isanewline
\endisadelimtheory
\isanewline
\isacommand{constdefs}\isamarkupfalse%
\isanewline
\ \ Med\ {\isacharcolon}{\isacharcolon}\ {\isachardoublequoteopen}{\isacharprime}t\ fstream\ {\isasymRightarrow}\ {\isacharprime}t\ fstream\ {\isasymRightarrow}\ bool{\isachardoublequoteclose}\isanewline
\ \ Med{\isacharunderscore}def{\isacharcolon}\ \ \isanewline
\ \ \ \ {\isachardoublequoteopen}Med\ s\ r\ {\isasymequiv}\ \isanewline
\ \ \ \ \ \ \ {\isasymexists}p{\isachardot}\ {\isacharhash}{\isacharparenleft}ffilter\ {\isacharbraceleft}True{\isacharbraceright}{\isasymcdot}p{\isacharparenright}\ {\isacharequal}\ {\isasyminfinity}\ {\isasymand}\ \isanewline
\ \ \ \ \ \ \ \ \ \ \ r\ {\isacharequal}\ fproj{\isadigit{1}}{\isasymcdot}{\isacharparenleft}ffilter\ {\isacharbraceleft}a{\isachardot}\ {\isasymexists}b{\isachardot}\ a\ {\isacharequal}\ {\isacharparenleft}b{\isacharcomma}\ True{\isacharparenright}{\isacharbraceright}{\isasymcdot}{\isacharparenleft}fzip{\isasymcdot}s{\isasymcdot}p{\isacharparenright}{\isacharparenright}{\isachardoublequoteclose}\ \isanewline
\isanewline
\isacommand{lemma}\isamarkupfalse%
\ ffilter{\isacharunderscore}fzip{\isacharunderscore}lemma{\isacharcolon}\ \isanewline
\ \ {\isachardoublequoteopen}{\isasymforall}ds{\isachardot}\ {\isacharhash}ds\ {\isacharequal}\ {\isasyminfinity}\ {\isasymlongrightarrow}\ \isanewline
\ \ \ \ \ \ \ \ fproj{\isadigit{2}}{\isasymcdot}{\isacharparenleft}ffilter\ {\isacharbraceleft}a{\isachardot}\ {\isasymexists}h{\isachardot}\ a\ {\isacharequal}\ {\isacharparenleft}h{\isacharcomma}z{\isacharparenright}{\isacharbraceright}{\isasymcdot}{\isacharparenleft}fzip{\isasymcdot}ds{\isasymcdot}p{\isacharparenright}{\isacharparenright}\ {\isacharequal}\ ffilter\ {\isacharbraceleft}z{\isacharbraceright}{\isasymcdot}p{\isachardoublequoteclose}\ \isanewline
\isadelimproof
\endisadelimproof
\isatagproof
\isacommand{apply}\isamarkupfalse%
\ {\isacharparenleft}rule\ fstream{\isacharunderscore}ind{\isadigit{1}}\ {\isacharbrackleft}of\ {\isacharunderscore}\ {\isachardoublequoteopen}p{\isachardoublequoteclose}{\isacharbrackright}{\isacharcomma}\ auto{\isacharparenright}\isanewline
\isacommand{apply}\isamarkupfalse%
\ {\isacharparenleft}case{\isacharunderscore}tac\ {\isachardoublequoteopen}ds{\isacharequal}{\isasymepsilon}{\isachardoublequoteclose}{\isacharcomma}\ auto{\isacharparenright}\isanewline
\isacommand{apply}\isamarkupfalse%
\ {\isacharparenleft}drule\ fscase{\isadigit{2}}{\isacharcomma}\ auto{\isacharparenright}\isanewline
\isacommand{apply}\isamarkupfalse%
\ {\isacharparenleft}case{\isacharunderscore}tac\ {\isachardoublequoteopen}z{\isacharequal}a{\isachardoublequoteclose}{\isacharcomma}\ auto{\isacharparenright}\isanewline
\isacommand{apply}\isamarkupfalse%
\ {\isacharparenleft}drule\ iSuc{\isadigit{2}}Inf{\isacharparenright}\isanewline
\isacommand{apply}\isamarkupfalse%
\ {\isacharparenleft}erule{\isacharunderscore}tac\ x{\isacharequal}{\isachardoublequoteopen}rs{\isachardoublequoteclose}\ \isakeyword{in}\ allE{\isacharcomma}\ simp{\isacharparenright}\isanewline
\isacommand{apply}\isamarkupfalse%
\ {\isacharparenleft}case{\isacharunderscore}tac\ {\isachardoublequoteopen}{\isacharparenleft}aa{\isacharcomma}\ a{\isacharparenright}\ {\isasymin}\ {\isacharbraceleft}a{\isachardot}\ {\isasymexists}h{\isachardot}\ a\ {\isacharequal}\ {\isacharparenleft}h{\isacharcomma}\ z{\isacharparenright}{\isacharbraceright}{\isachardoublequoteclose}{\isacharcomma}\ auto{\isacharparenright}\isanewline
\isacommand{by}\isamarkupfalse%
\ {\isacharparenleft}drule\ iSuc{\isadigit{2}}Inf{\isacharcomma}\ simp{\isacharparenright}%
\endisatagproof
{\isafoldproof}%
\isadelimproof
\endisadelimproof
\begin{isamarkuptext}%
In the following lemma the fairness property of $Medium$ is proved.%
\end{isamarkuptext}%
\isamarkuptrue%
\isacommand{lemma}\isamarkupfalse%
\ fair{\isacharunderscore}Med{\isacharcolon}\ \isanewline
\ \ {\isachardoublequoteopen}{\isasymlbrakk}{\isacharhash}ds\ {\isacharequal}\ {\isasyminfinity}{\isacharsemicolon}\ Med\ ds\ dr{\isasymrbrakk}\ {\isasymLongrightarrow}\ {\isacharhash}dr\ {\isacharequal}\ {\isasyminfinity}{\isachardoublequoteclose}\isanewline
\isadelimproof
\endisadelimproof
\isatagproof
\isacommand{apply}\isamarkupfalse%
\ {\isacharparenleft}auto\ simp\ add{\isacharcolon}\ Med{\isacharunderscore}def{\isacharparenright}\isanewline
\isacommand{apply}\isamarkupfalse%
\ {\isacharparenleft}insert\ ffilter{\isacharunderscore}fzip{\isacharunderscore}lemma\ \isanewline
\ \ \ \ \ \ \ \ \ {\isacharbrackleft}rule{\isacharunderscore}format{\isacharcomma}\ THEN\ sym{\isacharcomma}\ of\ {\isachardoublequoteopen}ds{\isachardoublequoteclose}\ {\isachardoublequoteopen}True{\isachardoublequoteclose}{\isacharbrackright}{\isacharcomma}\ atomize{\isacharparenright}\isanewline
\isacommand{apply}\isamarkupfalse%
\ {\isacharparenleft}erule{\isacharunderscore}tac\ x{\isacharequal}{\isachardoublequoteopen}p{\isachardoublequoteclose}\ \isakeyword{in}\ allE{\isacharcomma}\ auto{\isacharparenright}\isanewline
\isacommand{apply}\isamarkupfalse%
\ {\isacharparenleft}drule\ fslen{\isacharunderscore}arg{\isacharunderscore}cong{\isacharparenright}\isanewline
\isacommand{by}\isamarkupfalse%
\ {\isacharparenleft}auto\ simp\ add{\isacharcolon}\ fslen{\isacharunderscore}fprojs{\isacharunderscore}eq{\isacharparenright}%
\endisatagproof
{\isafoldproof}%
\isadelimproof
\isanewline
\endisadelimproof
\isanewline
\isacommand{lemma}\isamarkupfalse%
\ strict{\isacharunderscore}rev{\isacharunderscore}Med{\isacharcolon}\ \isanewline
\ \ {\isachardoublequoteopen}Med\ {\isasymepsilon}\ y\ {\isasymLongrightarrow}\ y\ {\isacharequal}\ {\isasymepsilon}{\isachardoublequoteclose}\isanewline
\isadelimproof
\endisadelimproof
\isatagproof
\isacommand{by}\isamarkupfalse%
\ {\isacharparenleft}simp\ add{\isacharcolon}\ Med{\isacharunderscore}def{\isacharparenright}%
\endisatagproof
{\isafoldproof}%
\isadelimproof
\isanewline
\endisadelimproof
\isanewline
\isacommand{lemma}\isamarkupfalse%
\ Med{\isacharunderscore}eps{\isacharunderscore}eps{\isacharbrackleft}simp{\isacharbrackright}{\isacharcolon}\ \isanewline
\ \ {\isachardoublequoteopen}Med\ {\isasymepsilon}\ {\isasymepsilon}{\isachardoublequoteclose}\isanewline
\isadelimproof
\endisadelimproof
\isatagproof
\isacommand{apply}\isamarkupfalse%
\ {\isacharparenleft}simp\ add{\isacharcolon}\ Med{\isacharunderscore}def{\isacharparenright}\isanewline
\isacommand{by}\isamarkupfalse%
\ {\isacharparenleft}rule{\isacharunderscore}tac\ x{\isacharequal}{\isachardoublequoteopen}ficycle\ {\isacharless}True{\isachargreater}{\isachardoublequoteclose}\ \isakeyword{in}\ exI{\isacharcomma}\ simp{\isacharparenright}%
\endisatagproof
{\isafoldproof}%
\isadelimproof
\endisadelimproof
\begin{isamarkuptext}%
To show that {\pisastyle{Med}} is transitive, we introduce the following 
\Focus function on the corresponding oracles.
\input{./focus-specs/ABP/tOrac}
\end{isamarkuptext}%
\isamarkuptrue%
\isacommand{constdefs}\isamarkupfalse%
\isanewline
\ \ tOrac\ {\isacharcolon}{\isacharcolon}\ {\isachardoublequoteopen}bool\ fstream\ {\isasymrightarrow}\ bool\ fstream\ {\isasymrightarrow}\ bool\ fstream{\isachardoublequoteclose}\isanewline
\ \ tOrac{\isacharunderscore}def{\isacharcolon}\isanewline
\ \ \ \ {\isachardoublequoteopen}tOrac\ {\isasymequiv}\ fix{\isasymcdot}{\isacharparenleft}{\isasymLambda}\ h\ p{\isadigit{1}}\ p{\isadigit{2}}{\isachardot}\ lookahead{\isasymcdot}p{\isadigit{1}}{\isasymcdot}{\isacharparenleft}{\isasymlambda}a{\isachardot}\ lookahead{\isasymcdot}p{\isadigit{2}}{\isasymcdot}{\isacharparenleft}{\isasymlambda}b{\isachardot}\ \isanewline
\ \ \ \ \ \ \ \ \ \ \ \ \ \ \ \ \ \ \ \ \ \ if\ a\ then\ \isanewline
\ \ \ \ \ \ \ \ \ \ \ \ \ \ \ \ \ \ \ \ \ \ \ \ \ if\ b\ then\ {\isacharless}True{\isachargreater}\ {\isasymfrown}\ h{\isasymcdot}{\isacharparenleft}frt{\isasymcdot}p{\isadigit{1}}{\isacharparenright}{\isasymcdot}{\isacharparenleft}frt{\isasymcdot}p{\isadigit{2}}{\isacharparenright}\ \isanewline
\ \ \ \ \ \ \ \ \ \ \ \ \ \ \ \ \ \ \ \ \ \ \ \ \ \ \ \ \ \ else\ {\isacharless}False{\isachargreater}\ {\isasymfrown}\ h{\isasymcdot}{\isacharparenleft}frt{\isasymcdot}p{\isadigit{1}}{\isacharparenright}{\isasymcdot}{\isacharparenleft}frt{\isasymcdot}p{\isadigit{2}}{\isacharparenright}\isanewline
\ \ \ \ \ \ \ \ \ \ \ \ \ \ \ \ \ \ \ \ \ \ \ \ \ else\ if\ b\ then\ {\isacharless}False{\isachargreater}\ {\isasymfrown}\ h{\isasymcdot}{\isacharparenleft}frt{\isasymcdot}p{\isadigit{1}}{\isacharparenright}{\isasymcdot}p{\isadigit{2}}\ \isanewline
\ \ \ \ \ \ \ \ \ \ \ \ \ \ \ \ \ \ \ \ \ \ \ \ \ \ \ \ \ \ \ \ \ \ \ else\ {\isacharless}False{\isachargreater}\ {\isasymfrown}\ h{\isasymcdot}{\isacharparenleft}frt{\isasymcdot}p{\isadigit{1}}{\isacharparenright}{\isasymcdot}p{\isadigit{2}}{\isacharparenright}{\isacharparenright}{\isacharparenright}{\isachardoublequoteclose}\isanewline
\isanewline
\isacommand{lemma}\isamarkupfalse%
\ tOrac{\isacharunderscore}unfold{\isadigit{1}}{\isacharbrackleft}simp{\isacharbrackright}{\isacharcolon}\ \isanewline
\ \ {\isachardoublequoteopen}tOrac{\isasymcdot}{\isasymepsilon}{\isasymcdot}p\ {\isacharequal}\ {\isasymepsilon}{\isachardoublequoteclose}\isanewline
\isadelimproof
\endisadelimproof
\isatagproof
\isacommand{by}\isamarkupfalse%
\ {\isacharparenleft}subst\ tOrac{\isacharunderscore}def\ {\isacharbrackleft}THEN\ fix{\isacharunderscore}eq{\isadigit{2}}{\isacharbrackright}{\isacharcomma}\ simp{\isacharparenright}%
\endisatagproof
{\isafoldproof}%
\isadelimproof
\isanewline
\endisadelimproof
\isanewline
\isacommand{lemma}\isamarkupfalse%
\ tOrac{\isacharunderscore}unfold{\isadigit{2}}{\isacharbrackleft}simp{\isacharbrackright}{\isacharcolon}\ \isanewline
\ \ {\isachardoublequoteopen}tOrac{\isasymcdot}p{\isasymcdot}{\isasymepsilon}\ {\isacharequal}\ {\isasymepsilon}{\isachardoublequoteclose}\isanewline
\isadelimproof
\endisadelimproof
\isatagproof
\isacommand{apply}\isamarkupfalse%
\ {\isacharparenleft}subst\ tOrac{\isacharunderscore}def\ {\isacharbrackleft}THEN\ fix{\isacharunderscore}eq{\isadigit{2}}{\isacharbrackright}{\isacharparenright}\isanewline
\isacommand{by}\isamarkupfalse%
\ {\isacharparenleft}case{\isacharunderscore}tac\ {\isachardoublequoteopen}p{\isacharequal}{\isasymepsilon}{\isachardoublequoteclose}{\isacharcomma}\ auto{\isacharparenright}%
\endisatagproof
{\isafoldproof}%
\isadelimproof
\isanewline
\endisadelimproof
\isanewline
\isacommand{lemma}\isamarkupfalse%
\ tOrac{\isacharunderscore}unfold{\isadigit{3}}{\isacharbrackleft}simp{\isacharbrackright}{\isacharcolon}\ \isanewline
\ \ {\isachardoublequoteopen}tOrac{\isasymcdot}{\isacharparenleft}{\isacharless}True{\isachargreater}\ {\isasymfrown}\ p{\isadigit{1}}{\isacharparenright}{\isasymcdot}{\isacharparenleft}{\isacharless}True{\isachargreater}\ {\isasymfrown}\ p{\isadigit{2}}{\isacharparenright}\ {\isacharequal}\ \isanewline
\ \ \ {\isacharless}True{\isachargreater}\ {\isasymfrown}\ tOrac{\isasymcdot}p{\isadigit{1}}{\isasymcdot}p{\isadigit{2}}{\isachardoublequoteclose}\isanewline
\isadelimproof
\endisadelimproof
\isatagproof
\isacommand{by}\isamarkupfalse%
\ {\isacharparenleft}subst\ tOrac{\isacharunderscore}def\ {\isacharbrackleft}THEN\ fix{\isacharunderscore}eq{\isadigit{2}}{\isacharbrackright}{\isacharcomma}\ simp{\isacharparenright}%
\endisatagproof
{\isafoldproof}%
\isadelimproof
\isanewline
\endisadelimproof
\isanewline
\isacommand{lemma}\isamarkupfalse%
\ tOrac{\isacharunderscore}unfold{\isadigit{4}}{\isacharbrackleft}simp{\isacharbrackright}{\isacharcolon}\ \isanewline
\ \ {\isachardoublequoteopen}tOrac{\isasymcdot}{\isacharparenleft}{\isacharless}True{\isachargreater}\ {\isasymfrown}\ p{\isadigit{1}}{\isacharparenright}{\isasymcdot}{\isacharparenleft}{\isacharless}False{\isachargreater}\ {\isasymfrown}\ p{\isadigit{2}}{\isacharparenright}\ {\isacharequal}\ \isanewline
\ \ \ {\isacharless}False{\isachargreater}\ {\isasymfrown}\ tOrac{\isasymcdot}p{\isadigit{1}}{\isasymcdot}p{\isadigit{2}}{\isachardoublequoteclose}\isanewline
\isadelimproof
\endisadelimproof
\isatagproof
\isacommand{by}\isamarkupfalse%
\ {\isacharparenleft}subst\ tOrac{\isacharunderscore}def\ {\isacharbrackleft}THEN\ fix{\isacharunderscore}eq{\isadigit{2}}{\isacharbrackright}{\isacharcomma}\ simp{\isacharparenright}%
\endisatagproof
{\isafoldproof}%
\isadelimproof
\isanewline
\endisadelimproof
\isanewline
\isacommand{lemma}\isamarkupfalse%
\ tOrac{\isacharunderscore}unfold{\isadigit{5}}{\isacharbrackleft}simp{\isacharbrackright}{\isacharcolon}\ \isanewline
\ \ {\isachardoublequoteopen}tOrac{\isasymcdot}{\isacharparenleft}{\isacharless}False{\isachargreater}\ {\isasymfrown}\ p{\isadigit{1}}{\isacharparenright}{\isasymcdot}{\isacharparenleft}{\isacharless}True{\isachargreater}\ {\isasymfrown}\ p{\isadigit{2}}{\isacharparenright}\ {\isacharequal}\ \isanewline
\ \ \ {\isacharless}False{\isachargreater}\ {\isasymfrown}\ tOrac{\isasymcdot}p{\isadigit{1}}{\isasymcdot}{\isacharparenleft}{\isacharless}True{\isachargreater}\ {\isasymfrown}\ p{\isadigit{2}}{\isacharparenright}{\isachardoublequoteclose}\isanewline
\isadelimproof
\endisadelimproof
\isatagproof
\isacommand{by}\isamarkupfalse%
\ {\isacharparenleft}subst\ tOrac{\isacharunderscore}def\ {\isacharbrackleft}THEN\ fix{\isacharunderscore}eq{\isadigit{2}}{\isacharbrackright}{\isacharcomma}\ simp{\isacharparenright}%
\endisatagproof
{\isafoldproof}%
\isadelimproof
\isanewline
\endisadelimproof
\isanewline
\isacommand{lemma}\isamarkupfalse%
\ tOrac{\isacharunderscore}unfold{\isadigit{6}}{\isacharbrackleft}simp{\isacharbrackright}{\isacharcolon}\ \isanewline
\ \ {\isachardoublequoteopen}tOrac{\isasymcdot}{\isacharparenleft}{\isacharless}False{\isachargreater}\ {\isasymfrown}\ p{\isadigit{1}}{\isacharparenright}{\isasymcdot}{\isacharparenleft}{\isacharless}False{\isachargreater}\ {\isasymfrown}\ p{\isadigit{2}}{\isacharparenright}\ {\isacharequal}\ \isanewline
\ \ \ {\isacharless}False{\isachargreater}\ {\isasymfrown}\ tOrac{\isasymcdot}p{\isadigit{1}}{\isasymcdot}{\isacharparenleft}{\isacharless}False{\isachargreater}\ {\isasymfrown}\ p{\isadigit{2}}{\isacharparenright}{\isachardoublequoteclose}\isanewline
\isadelimproof
\endisadelimproof
\isatagproof
\isacommand{by}\isamarkupfalse%
\ {\isacharparenleft}subst\ tOrac{\isacharunderscore}def\ {\isacharbrackleft}THEN\ fix{\isacharunderscore}eq{\isadigit{2}}{\isacharbrackright}{\isacharcomma}\ simp{\isacharparenright}%
\endisatagproof
{\isafoldproof}%
\isadelimproof
\isanewline
\endisadelimproof
\isanewline
\isacommand{lemma}\isamarkupfalse%
\ tOrac{\isacharunderscore}Med{\isacharbrackleft}rule{\isacharunderscore}format{\isacharbrackright}{\isacharcolon}\ \isanewline
\ \ {\isachardoublequoteopen}{\isasymforall}p\ pa{\isachardot}\ fproj{\isadigit{1}}{\isasymcdot}{\isacharparenleft}ffilter\ {\isacharbraceleft}a{\isachardot}\ {\isasymexists}b{\isachardot}\ a\ {\isacharequal}\ {\isacharparenleft}b{\isacharcomma}\ True{\isacharparenright}{\isacharbraceright}{\isasymcdot}\isanewline
\ \ \ \ \ \ \ \ \ \ \ \ {\isacharparenleft}fzip{\isasymcdot}{\isacharparenleft}fproj{\isadigit{1}}{\isasymcdot}{\isacharparenleft}ffilter\ {\isacharbraceleft}a{\isachardot}\ {\isasymexists}b{\isachardot}\ a\ {\isacharequal}\ {\isacharparenleft}b{\isacharcomma}\ True{\isacharparenright}{\isacharbraceright}{\isasymcdot}{\isacharparenleft}fzip{\isasymcdot}x{\isasymcdot}p{\isacharparenright}{\isacharparenright}{\isacharparenright}{\isasymcdot}pa{\isacharparenright}{\isacharparenright}\ {\isacharequal}\isanewline
\ \ \ \ \ \ \ \ \ \ fproj{\isadigit{1}}{\isasymcdot}{\isacharparenleft}ffilter\ {\isacharbraceleft}a{\isachardot}\ {\isasymexists}b{\isachardot}\ a\ {\isacharequal}\ {\isacharparenleft}b{\isacharcomma}\ True{\isacharparenright}{\isacharbraceright}{\isasymcdot}{\isacharparenleft}fzip{\isasymcdot}x{\isasymcdot}{\isacharparenleft}tOrac{\isasymcdot}p{\isasymcdot}pa{\isacharparenright}{\isacharparenright}{\isacharparenright}{\isachardoublequoteclose}\isanewline
\isadelimproof
\endisadelimproof
\isatagproof
\isacommand{apply}\isamarkupfalse%
\ {\isacharparenleft}rule\ fstream{\isacharunderscore}ind{\isadigit{1}}\ {\isacharbrackleft}of\ {\isacharunderscore}\ x{\isacharbrackright}{\isacharcomma}\ auto{\isacharparenright}\isanewline
\isacommand{apply}\isamarkupfalse%
\ {\isacharparenleft}case{\isacharunderscore}tac\ {\isachardoublequoteopen}p{\isacharequal}{\isasymepsilon}{\isachardoublequoteclose}{\isacharcomma}\ auto{\isacharparenright}\isanewline
\isacommand{apply}\isamarkupfalse%
\ {\isacharparenleft}case{\isacharunderscore}tac\ {\isachardoublequoteopen}pa{\isacharequal}{\isasymepsilon}{\isachardoublequoteclose}{\isacharcomma}\ auto{\isacharparenright}\isanewline
\isacommand{apply}\isamarkupfalse%
\ {\isacharparenleft}drule\ fscase{\isadigit{2}}{\isacharcomma}\ auto{\isacharparenright}{\isacharplus}\isanewline
\isacommand{apply}\isamarkupfalse%
\ {\isacharparenleft}case{\isacharunderscore}tac\ {\isachardoublequoteopen}aa{\isachardoublequoteclose}{\isacharcomma}\ auto{\isacharparenright}\isanewline
\isacommand{apply}\isamarkupfalse%
\ {\isacharparenleft}case{\isacharunderscore}tac\ {\isachardoublequoteopen}ab{\isachardoublequoteclose}{\isacharcomma}\ auto{\isacharparenright}\isanewline
\isacommand{by}\isamarkupfalse%
\ {\isacharparenleft}case{\isacharunderscore}tac\ {\isachardoublequoteopen}ab{\isachardoublequoteclose}{\isacharcomma}\ auto{\isacharparenright}%
\endisatagproof
{\isafoldproof}%
\isadelimproof
\isanewline
\endisadelimproof
\isanewline
\isacommand{lemma}\isamarkupfalse%
\ fair{\isacharunderscore}trans{\isacharunderscore}Med{\isacharunderscore}lemma{\isacharcolon}\ \isanewline
\ \ {\isachardoublequoteopen}{\isasymforall}x{\isachardot}\ {\isacharhash}x\ {\isacharequal}\ {\isasyminfinity}\ {\isasymlongrightarrow}\ {\isacharhash}{\isacharparenleft}ffilter\ {\isacharbraceleft}b{\isacharbraceright}{\isasymcdot}p{\isacharparenright}\ {\isacharequal}\ {\isacharhash}{\isacharparenleft}ffilter\ {\isacharbraceleft}x{\isachardot}\ {\isasymexists}a{\isachardot}\ x\ {\isacharequal}\ {\isacharparenleft}a{\isacharcomma}\ b{\isacharparenright}{\isacharbraceright}{\isasymcdot}{\isacharparenleft}fzip{\isasymcdot}x{\isasymcdot}p{\isacharparenright}{\isacharparenright}{\isachardoublequoteclose}\ \isanewline
\isadelimproof
\endisadelimproof
\isatagproof
\isacommand{apply}\isamarkupfalse%
\ {\isacharparenleft}rule\ fstream{\isacharunderscore}ind{\isadigit{1}}\ {\isacharbrackleft}of\ {\isacharunderscore}\ p{\isacharbrackright}{\isacharcomma}\ auto{\isacharparenright}\isanewline
\isacommand{apply}\isamarkupfalse%
\ {\isacharparenleft}case{\isacharunderscore}tac\ {\isachardoublequoteopen}x{\isacharequal}{\isasymepsilon}{\isachardoublequoteclose}{\isacharcomma}\ auto{\isacharparenright}\isanewline
\isacommand{apply}\isamarkupfalse%
\ {\isacharparenleft}drule\ fscase{\isadigit{2}}{\isacharcomma}\ auto{\isacharparenright}\isanewline
\isacommand{apply}\isamarkupfalse%
\ {\isacharparenleft}case{\isacharunderscore}tac\ {\isachardoublequoteopen}a\ {\isacharequal}\ b{\isachardoublequoteclose}{\isacharcomma}\ auto{\isacharparenright}\isanewline
\isacommand{by}\isamarkupfalse%
\ {\isacharparenleft}simp\ add{\isacharcolon}\ inat{\isacharunderscore}defs\ split{\isacharcolon}\ inat{\isacharunderscore}splits{\isacharparenright}{\isacharplus}%
\endisatagproof
{\isafoldproof}%
\isadelimproof
\isanewline
\endisadelimproof
\isanewline
\isacommand{lemma}\isamarkupfalse%
\ fin{\isacharunderscore}tOrac{\isacharunderscore}lemma\ {\isacharbrackleft}rule{\isacharunderscore}format{\isacharbrackright}{\isacharcolon}\isanewline
\ \ {\isachardoublequoteopen}{\isasymforall}x\ p\ pa\ pb{\isachardot}\ \isanewline
\ \ \ \ \ \ {\isacharhash}x\ {\isacharequal}\ Fin\ n\ {\isasymand}\ {\isacharhash}{\isacharparenleft}ffilter\ {\isacharbraceleft}True{\isacharbraceright}{\isasymcdot}p{\isacharparenright}\ {\isacharequal}\ {\isasyminfinity}\ {\isasymand}\ \isanewline
\ \ \ \ \ \ {\isacharhash}{\isacharparenleft}ffilter\ {\isacharbraceleft}True{\isacharbraceright}{\isasymcdot}pa{\isacharparenright}\ {\isacharequal}\ {\isasyminfinity}\ {\isasymlongrightarrow}\ \isanewline
\ \ \ \ \ \ \ \ {\isacharparenleft}{\isasymexists}pb{\isachardot}\ {\isacharhash}{\isacharparenleft}ffilter\ {\isacharbraceleft}True{\isacharbraceright}{\isasymcdot}pb{\isacharparenright}\ {\isacharequal}\ {\isasyminfinity}\ {\isasymand}\isanewline
\ \ \ \ \ \ \ \ \ \ \ \ \ \ fproj{\isadigit{1}}{\isasymcdot}{\isacharparenleft}ffilter\ {\isacharbraceleft}a{\isachardot}\ {\isasymexists}b{\isachardot}\ a\ {\isacharequal}\ {\isacharparenleft}b{\isacharcomma}\ True{\isacharparenright}{\isacharbraceright}{\isasymcdot}\isanewline
\ \ \ \ \ \ \ \ \ \ \ \ \ \ \ \ {\isacharparenleft}fzip{\isasymcdot}{\isacharparenleft}fproj{\isadigit{1}}{\isasymcdot}{\isacharparenleft}ffilter\ {\isacharbraceleft}a{\isachardot}\ {\isasymexists}b{\isachardot}\ a\ {\isacharequal}\ {\isacharparenleft}b{\isacharcomma}\ True{\isacharparenright}{\isacharbraceright}{\isasymcdot}{\isacharparenleft}fzip{\isasymcdot}x{\isasymcdot}p{\isacharparenright}{\isacharparenright}{\isacharparenright}{\isasymcdot}pa{\isacharparenright}{\isacharparenright}\ {\isacharequal}\isanewline
\ \ \ \ \ \ \ \ \ \ \ \ \ \ \ \ \ \ \ fproj{\isadigit{1}}{\isasymcdot}{\isacharparenleft}ffilter\ {\isacharbraceleft}a{\isachardot}\ {\isasymexists}b{\isachardot}\ a\ {\isacharequal}\ {\isacharparenleft}b{\isacharcomma}\ True{\isacharparenright}{\isacharbraceright}{\isasymcdot}{\isacharparenleft}fzip{\isasymcdot}x{\isasymcdot}pb{\isacharparenright}{\isacharparenright}{\isacharparenright}{\isachardoublequoteclose}\isanewline
\isadelimproof
\endisadelimproof
\isatagproof
\isacommand{apply}\isamarkupfalse%
\ {\isacharparenleft}induct{\isacharunderscore}tac\ n{\isacharcomma}\ auto{\isacharparenright}\isanewline
\isacommand{apply}\isamarkupfalse%
\ {\isacharparenleft}simp\ add{\isacharcolon}\ Fin{\isacharunderscore}{\isadigit{0}}{\isacharparenright}\isanewline
\isacommand{apply}\isamarkupfalse%
\ {\isacharparenleft}rule{\isacharunderscore}tac\ x{\isacharequal}{\isachardoublequoteopen}ficycle\ {\isacharless}True{\isachargreater}{\isachardoublequoteclose}\ \isakeyword{in}\ exI{\isacharcomma}\ auto{\isacharparenright}\isanewline
\isacommand{apply}\isamarkupfalse%
\ {\isacharparenleft}case{\isacharunderscore}tac\ {\isachardoublequoteopen}x{\isacharequal}{\isasymepsilon}{\isachardoublequoteclose}{\isacharcomma}\ auto{\isacharparenright}\isanewline
\isacommand{apply}\isamarkupfalse%
\ {\isacharparenleft}drule\ fscase{\isadigit{2}}{\isacharcomma}\ auto{\isacharparenright}\isanewline
\isacommand{apply}\isamarkupfalse%
\ {\isacharparenleft}erule{\isacharunderscore}tac\ x{\isacharequal}{\isachardoublequoteopen}rs{\isachardoublequoteclose}\ \isakeyword{in}\ allE{\isacharparenright}\isanewline
\isacommand{apply}\isamarkupfalse%
\ {\isacharparenleft}erule{\isacharunderscore}tac\ x{\isacharequal}{\isachardoublequoteopen}frt{\isasymcdot}p{\isachardoublequoteclose}\ \isakeyword{in}\ allE{\isacharparenright}\isanewline
\isacommand{apply}\isamarkupfalse%
\ {\isacharparenleft}case{\isacharunderscore}tac\ {\isachardoublequoteopen}p{\isacharequal}{\isasymepsilon}{\isachardoublequoteclose}{\isacharcomma}\ auto{\isacharparenright}\isanewline
\isacommand{apply}\isamarkupfalse%
\ {\isacharparenleft}drule\ fscase{\isadigit{2}}{\isacharcomma}\ auto{\isacharparenright}\isanewline
\isacommand{apply}\isamarkupfalse%
\ {\isacharparenleft}case{\isacharunderscore}tac\ {\isachardoublequoteopen}aa{\isachardoublequoteclose}{\isacharcomma}\ auto{\isacharparenright}\isanewline
\isacommand{apply}\isamarkupfalse%
\ {\isacharparenleft}case{\isacharunderscore}tac\ {\isachardoublequoteopen}pa\ {\isacharequal}\ {\isasymepsilon}{\isachardoublequoteclose}{\isacharcomma}\ auto{\isacharparenright}\isanewline
\isacommand{apply}\isamarkupfalse%
\ {\isacharparenleft}drule\ fscase{\isadigit{2}}{\isacharcomma}\ auto{\isacharparenright}\isanewline
\isacommand{apply}\isamarkupfalse%
\ {\isacharparenleft}case{\isacharunderscore}tac\ {\isachardoublequoteopen}ab{\isachardoublequoteclose}{\isacharcomma}\ auto{\isacharparenright}\isanewline
\isacommand{apply}\isamarkupfalse%
\ {\isacharparenleft}erule{\isacharunderscore}tac\ x{\isacharequal}{\isachardoublequoteopen}rsb{\isachardoublequoteclose}\ \isakeyword{in}\ allE{\isacharcomma}\ auto{\isacharparenright}\ \isacommand{prefer}\isamarkupfalse%
\ {\isadigit{4}}\isanewline
\isacommand{apply}\isamarkupfalse%
\ {\isacharparenleft}rule{\isacharunderscore}tac\ x{\isacharequal}{\isachardoublequoteopen}{\isacharless}True{\isachargreater}\ {\isasymfrown}\ pb{\isachardoublequoteclose}\ \isakeyword{in}\ exI{\isacharcomma}\ simp{\isacharparenright}\isanewline
\isacommand{apply}\isamarkupfalse%
\ {\isacharparenleft}simp\ add{\isacharcolon}\ inat{\isacharunderscore}defs\ split{\isacharcolon}\ inat{\isacharunderscore}splits{\isacharparenright}{\isacharplus}\isanewline
\isacommand{apply}\isamarkupfalse%
\ {\isacharparenleft}erule{\isacharunderscore}tac\ x{\isacharequal}{\isachardoublequoteopen}rsb{\isachardoublequoteclose}\ \isakeyword{in}\ allE{\isacharcomma}\ auto{\isacharparenright}\isanewline
\isacommand{apply}\isamarkupfalse%
\ {\isacharparenleft}rule{\isacharunderscore}tac\ x{\isacharequal}{\isachardoublequoteopen}{\isacharless}False{\isachargreater}\ {\isasymfrown}\ pb{\isachardoublequoteclose}\ \isakeyword{in}\ exI{\isacharcomma}\ simp{\isacharparenright}\isanewline
\isacommand{apply}\isamarkupfalse%
\ {\isacharparenleft}erule{\isacharunderscore}tac\ x{\isacharequal}{\isachardoublequoteopen}pa{\isachardoublequoteclose}\ \isakeyword{in}\ allE{\isacharcomma}\ auto{\isacharparenright}\isanewline
\isacommand{apply}\isamarkupfalse%
\ {\isacharparenleft}simp\ add{\isacharcolon}\ inat{\isacharunderscore}defs\ split{\isacharcolon}\ inat{\isacharunderscore}splits{\isacharparenright}\isanewline
\isacommand{by}\isamarkupfalse%
\ {\isacharparenleft}rule{\isacharunderscore}tac\ x{\isacharequal}{\isachardoublequoteopen}{\isacharless}False{\isachargreater}\ {\isasymfrown}\ pb{\isachardoublequoteclose}\ \isakeyword{in}\ exI{\isacharcomma}\ auto{\isacharparenright}%
\endisatagproof
{\isafoldproof}%
\isadelimproof
\endisadelimproof
\begin{isamarkuptext}%
The following lemma plays a key role in our proof of the correctness of the protocol
in the last section of this chapter (Section~\ref{ABP_sys}), 
since it allows us to short-circuit both of the involved media by taking
care of their interfaces (see Figure~\ref{fig_abp}).%
\end{isamarkuptext}%
\isamarkuptrue%
\isacommand{lemma}\isamarkupfalse%
\ trans{\isacharunderscore}Med{\isacharcolon}\ {\isachardoublequoteopen}{\isasymlbrakk}Med\ x\ y{\isacharsemicolon}\ Med\ y\ z{\isasymrbrakk}\ {\isasymLongrightarrow}\ Med\ x\ z{\isachardoublequoteclose}\ \isanewline
\isadelimproof
\endisadelimproof
\isatagproof
\isacommand{apply}\isamarkupfalse%
\ {\isacharparenleft}case{\isacharunderscore}tac\ {\isachardoublequoteopen}{\isacharhash}x{\isachardoublequoteclose}{\isacharparenright}\isanewline
\isacommand{apply}\isamarkupfalse%
\ {\isacharparenleft}simp\ add{\isacharcolon}\ Med{\isacharunderscore}def{\isacharcomma}\ auto{\isacharparenright}\isanewline
\isacommand{apply}\isamarkupfalse%
\ {\isacharparenleft}rule\ fin{\isacharunderscore}tOrac{\isacharunderscore}lemma{\isacharcomma}\ auto{\isacharparenright}\isanewline
\isacommand{apply}\isamarkupfalse%
\ {\isacharparenleft}frule\ fair{\isacharunderscore}Med{\isacharcomma}\ auto{\isacharparenright}\isanewline
\isacommand{apply}\isamarkupfalse%
\ {\isacharparenleft}frule\ fair{\isacharunderscore}Med\ {\isacharbrackleft}of\ y\ z{\isacharbrackright}{\isacharcomma}\ auto{\isacharparenright}\isanewline
\isacommand{apply}\isamarkupfalse%
\ {\isacharparenleft}auto\ simp\ add{\isacharcolon}\ Med{\isacharunderscore}def{\isacharparenright}\isanewline
\isacommand{apply}\isamarkupfalse%
\ {\isacharparenleft}rule{\isacharunderscore}tac\ x{\isacharequal}{\isachardoublequoteopen}tOrac{\isasymcdot}p{\isasymcdot}pa{\isachardoublequoteclose}\ \isakeyword{in}\ exI{\isacharparenright}\isanewline
\isacommand{apply}\isamarkupfalse%
\ {\isacharparenleft}simp\ add{\isacharcolon}\ tOrac{\isacharunderscore}Med{\isacharparenright}\isanewline
\isacommand{apply}\isamarkupfalse%
\ {\isacharparenleft}simp\ add{\isacharcolon}\ fproj{\isadigit{1}}{\isacharunderscore}fslen{\isacharparenright}\isanewline
\isacommand{by}\isamarkupfalse%
\ {\isacharparenleft}simp\ add{\isacharcolon}\ fair{\isacharunderscore}trans{\isacharunderscore}Med{\isacharunderscore}lemma\ {\isacharbrackleft}rule{\isacharunderscore}format{\isacharbrackright}{\isacharparenright}%
\endisatagproof
{\isafoldproof}%
\isadelimproof
\isanewline
\endisadelimproof
\isanewline
\isacommand{lemma}\isamarkupfalse%
\ triv{\isacharunderscore}oracle{\isacharunderscore}lemma{\isadigit{1}}{\isacharbrackleft}simp{\isacharbrackright}{\isacharcolon}\ \isanewline
\ \ {\isachardoublequoteopen}fproj{\isadigit{1}}{\isasymcdot}{\isacharparenleft}ffilter\ {\isacharbraceleft}a{\isachardot}\ {\isasymexists}b{\isachardot}\ a\ {\isacharequal}\ {\isacharparenleft}b{\isacharcomma}\ True{\isacharparenright}{\isacharbraceright}{\isasymcdot}{\isacharparenleft}fzip{\isasymcdot}x{\isasymcdot}{\isacharparenleft}ficycle\ {\isacharless}True{\isachargreater}{\isacharparenright}{\isacharparenright}{\isacharparenright}\ {\isacharequal}\ x{\isachardoublequoteclose}\isanewline
\isadelimproof
\endisadelimproof
\isatagproof
\isacommand{apply}\isamarkupfalse%
\ {\isacharparenleft}rule\ fstream{\isacharunderscore}ind{\isadigit{1}}\ {\isacharbrackleft}of\ {\isacharunderscore}\ x{\isacharbrackright}{\isacharcomma}\ auto{\isacharparenright}\isanewline
\isacommand{apply}\isamarkupfalse%
\ {\isacharparenleft}case{\isacharunderscore}tac\ {\isachardoublequoteopen}s{\isacharequal}{\isasymepsilon}{\isachardoublequoteclose}{\isacharcomma}\ auto{\isacharparenright}\isanewline
\isacommand{apply}\isamarkupfalse%
\ {\isacharparenleft}subst\ ficycle{\isacharunderscore}unfold{\isacharcomma}\ simp{\isacharparenright}\isanewline
\isacommand{apply}\isamarkupfalse%
\ {\isacharparenleft}drule\ fscase{\isadigit{2}}{\isacharcomma}\ auto{\isacharparenright}\isanewline
\isacommand{by}\isamarkupfalse%
\ {\isacharparenleft}subst\ ficycle{\isacharunderscore}unfold{\isacharcomma}\ simp{\isacharparenright}%
\endisatagproof
{\isafoldproof}%
\isadelimproof
\endisadelimproof
\begin{isamarkuptext}%
In the following we prove a number of various unfolding properties for 
the predicate {\pisastyle{Med}}.%
\end{isamarkuptext}%
\isamarkuptrue%
\isacommand{lemma}\isamarkupfalse%
\ Med{\isacharunderscore}frt{\isacharunderscore}lemma{\isacharcolon}\ {\isachardoublequoteopen}Med\ x\ {\isacharparenleft}frt{\isasymcdot}x{\isacharparenright}{\isachardoublequoteclose}\isanewline
\isadelimproof
\endisadelimproof
\isatagproof
\isacommand{apply}\isamarkupfalse%
\ {\isacharparenleft}auto\ simp\ add{\isacharcolon}\ Med{\isacharunderscore}def{\isacharparenright}\isanewline
\isacommand{apply}\isamarkupfalse%
\ {\isacharparenleft}rule{\isacharunderscore}tac\ x{\isacharequal}{\isachardoublequoteopen}{\isacharless}False{\isachargreater}\ {\isasymfrown}\ {\isacharparenleft}ficycle\ {\isacharless}True{\isachargreater}{\isacharparenright}{\isachardoublequoteclose}\ \isakeyword{in}\ exI{\isacharcomma}\ auto{\isacharparenright}\ \isanewline
\isacommand{apply}\isamarkupfalse%
\ {\isacharparenleft}case{\isacharunderscore}tac\ {\isachardoublequoteopen}x{\isacharequal}{\isasymepsilon}{\isachardoublequoteclose}{\isacharcomma}\ auto{\isacharparenright}\isanewline
\isacommand{by}\isamarkupfalse%
\ {\isacharparenleft}drule\ fscase{\isadigit{2}}{\isacharcomma}\ auto{\isacharparenright}%
\endisatagproof
{\isafoldproof}%
\isadelimproof
\isanewline
\endisadelimproof
\isanewline
\isacommand{lemma}\isamarkupfalse%
\ Med{\isacharunderscore}frt{\isadigit{2}}{\isacharcolon}\ \isanewline
\ \ {\isachardoublequoteopen}Med\ x\ y\ {\isasymLongrightarrow}\ Med\ x\ {\isacharparenleft}frt{\isasymcdot}y{\isacharparenright}{\isachardoublequoteclose}\isanewline
\isadelimproof
\endisadelimproof
\isatagproof
\isacommand{apply}\isamarkupfalse%
\ {\isacharparenleft}insert\ Med{\isacharunderscore}frt{\isacharunderscore}lemma\ {\isacharbrackleft}of\ y{\isacharbrackright}{\isacharparenright}\isanewline
\isacommand{by}\isamarkupfalse%
\ {\isacharparenleft}rule\ trans{\isacharunderscore}Med{\isacharcomma}\ auto{\isacharparenright}%
\endisatagproof
{\isafoldproof}%
\isadelimproof
\isanewline
\endisadelimproof
\isanewline
\isacommand{lemma}\isamarkupfalse%
\ Med{\isacharunderscore}fdrop{\isadigit{2}}{\isacharcolon}\ \isanewline
\ \ {\isachardoublequoteopen}Med\ x\ y\ {\isasymlongrightarrow}\ Med\ x\ {\isacharparenleft}fdrop\ n{\isasymcdot}y{\isacharparenright}{\isachardoublequoteclose}\isanewline
\isadelimproof
\endisadelimproof
\isatagproof
\isacommand{apply}\isamarkupfalse%
\ {\isacharparenleft}induct{\isacharunderscore}tac\ n{\isacharcomma}\ auto{\isacharparenright}\isanewline
\isacommand{by}\isamarkupfalse%
\ {\isacharparenleft}subst\ fdrop{\isacharunderscore}unfold{\isadigit{2}}{\isacharcomma}\ rule\ Med{\isacharunderscore}frt{\isadigit{2}}{\isacharparenright}%
\endisatagproof
{\isafoldproof}%
\isadelimproof
\endisadelimproof
\begin{isamarkuptext}%
Additionally, we introduce a help function {\pisastyle{rOrac}} to show 
further unfolding properties for {\pisastyle{Med}} in the remaining theory.
{\pisastyle{rOrac}} converts the first 1-valued bit to 0 in an arbitrary oracle.
Firstly, we give a \Focus specification of {\pisastyle{rOrac}} in the following.  
\input{./focus-specs/ABP/rOrac}
\end{isamarkuptext}%
\isamarkuptrue%
\isacommand{constdefs}\isamarkupfalse%
\isanewline
\ \ rOrac\ {\isacharcolon}{\isacharcolon}\ \ \ {\isachardoublequoteopen}bool\ fstream\ {\isasymrightarrow}\ bool\ fstream{\isachardoublequoteclose}\isanewline
\ \ rOrac{\isacharunderscore}def{\isacharcolon}\ \isanewline
\ \ \ \ {\isachardoublequoteopen}rOrac\ {\isasymequiv}\ fix{\isasymcdot}{\isacharparenleft}{\isasymLambda}\ h\ p{\isachardot}\ lookahead{\isasymcdot}p{\isasymcdot}{\isacharparenleft}{\isasymlambda}\ b{\isachardot}\ \isanewline
\ \ \ \ \ \ \ \ \ \ \ \ \ \ \ if\ b\ then\ {\isacharless}False{\isachargreater}\ {\isasymfrown}\ frt{\isasymcdot}p\ else\ {\isacharless}b{\isachargreater}\ {\isasymfrown}\ h{\isasymcdot}{\isacharparenleft}frt{\isasymcdot}p{\isacharparenright}{\isacharparenright}{\isacharparenright}{\isachardoublequoteclose}\isanewline
\isanewline
\isacommand{lemma}\isamarkupfalse%
\ rOrac{\isacharunderscore}empty{\isacharbrackleft}simp{\isacharbrackright}{\isacharcolon}\ \isanewline
\ \ {\isachardoublequoteopen}rOrac{\isasymcdot}{\isasymepsilon}\ {\isacharequal}\ {\isasymepsilon}{\isachardoublequoteclose}\isanewline
\isadelimproof
\endisadelimproof
\isatagproof
\isacommand{by}\isamarkupfalse%
\ {\isacharparenleft}subst\ rOrac{\isacharunderscore}def\ {\isacharbrackleft}THEN\ fix{\isacharunderscore}eq{\isadigit{2}}{\isacharbrackright}{\isacharcomma}\ simp{\isacharparenright}%
\endisatagproof
{\isafoldproof}%
\isadelimproof
\isanewline
\endisadelimproof
\isanewline
\isacommand{lemma}\isamarkupfalse%
\ rOrac{\isacharunderscore}unfold{\isadigit{1}}{\isacharbrackleft}simp{\isacharbrackright}{\isacharcolon}\ \isanewline
\ \ {\isachardoublequoteopen}rOrac{\isasymcdot}{\isacharparenleft}{\isacharless}False{\isachargreater}\ {\isasymfrown}\ p{\isacharparenright}\ {\isacharequal}\ {\isacharless}False{\isachargreater}\ {\isasymfrown}\ rOrac{\isasymcdot}p{\isachardoublequoteclose}\isanewline
\isadelimproof
\endisadelimproof
\isatagproof
\isacommand{by}\isamarkupfalse%
\ {\isacharparenleft}subst\ rOrac{\isacharunderscore}def\ {\isacharbrackleft}THEN\ fix{\isacharunderscore}eq{\isadigit{2}}{\isacharbrackright}{\isacharcomma}\ simp{\isacharparenright}%
\endisatagproof
{\isafoldproof}%
\isadelimproof
\isanewline
\endisadelimproof
\isanewline
\isacommand{lemma}\isamarkupfalse%
\ rOrac{\isacharunderscore}unfold{\isadigit{2}}{\isacharbrackleft}simp{\isacharbrackright}{\isacharcolon}\ \isanewline
\ \ {\isachardoublequoteopen}rOrac{\isasymcdot}{\isacharparenleft}{\isacharless}True{\isachargreater}\ {\isasymfrown}\ p{\isacharparenright}\ {\isacharequal}\ {\isacharless}False{\isachargreater}\ {\isasymfrown}\ p{\isachardoublequoteclose}\isanewline
\isadelimproof
\endisadelimproof
\isatagproof
\isacommand{by}\isamarkupfalse%
\ {\isacharparenleft}subst\ rOrac{\isacharunderscore}def\ {\isacharbrackleft}THEN\ fix{\isacharunderscore}eq{\isadigit{2}}{\isacharbrackright}{\isacharcomma}\ simp{\isacharparenright}%
\endisatagproof
{\isafoldproof}%
\isadelimproof
\isanewline
\endisadelimproof
\isanewline
\isacommand{lemma}\isamarkupfalse%
\ rOrac{\isacharunderscore}lone{\isadigit{1}}{\isacharbrackleft}simp{\isacharbrackright}{\isacharcolon}\ \isanewline
\ \ {\isachardoublequoteopen}rOrac{\isasymcdot}{\isacharparenleft}{\isacharless}True{\isachargreater}{\isacharparenright}\ {\isacharequal}\ {\isacharless}False{\isachargreater}{\isachardoublequoteclose}\isanewline
\isadelimproof
\endisadelimproof
\isatagproof
\isacommand{by}\isamarkupfalse%
\ {\isacharparenleft}subst\ lone{\isacharunderscore}conv{\isacharcomma}\ subst\ rOrac{\isacharunderscore}unfold{\isadigit{2}}{\isacharcomma}\ simp{\isacharparenright}%
\endisatagproof
{\isafoldproof}%
\isadelimproof
\isanewline
\endisadelimproof
\isanewline
\isacommand{lemma}\isamarkupfalse%
\ rOrac{\isacharunderscore}lone{\isadigit{2}}{\isacharbrackleft}simp{\isacharbrackright}{\isacharcolon}\ \isanewline
\ \ {\isachardoublequoteopen}rOrac{\isasymcdot}{\isacharparenleft}{\isacharless}False{\isachargreater}{\isacharparenright}\ {\isacharequal}\ {\isacharless}False{\isachargreater}{\isachardoublequoteclose}\isanewline
\isadelimproof
\endisadelimproof
\isatagproof
\isacommand{by}\isamarkupfalse%
\ {\isacharparenleft}subst\ lone{\isacharunderscore}conv{\isacharcomma}\ subst\ rOrac{\isacharunderscore}unfold{\isadigit{1}}{\isacharcomma}\ simp{\isacharparenright}%
\endisatagproof
{\isafoldproof}%
\isadelimproof
\isanewline
\endisadelimproof
\isanewline
\isacommand{lemma}\isamarkupfalse%
\ rOrac{\isacharunderscore}lemma{\isadigit{1}}{\isacharbrackleft}rule{\isacharunderscore}format{\isacharbrackright}{\isacharcolon}\ \isanewline
\ \ {\isachardoublequoteopen}{\isasymforall}x{\isachardot}\ frt{\isasymcdot}{\isacharparenleft}fproj{\isadigit{1}}{\isasymcdot}{\isacharparenleft}ffilter\ {\isacharbraceleft}a{\isachardot}\ {\isasymexists}b{\isachardot}\ a\ {\isacharequal}\ {\isacharparenleft}b{\isacharcomma}\ True{\isacharparenright}{\isacharbraceright}{\isasymcdot}{\isacharparenleft}fzip{\isasymcdot}x{\isasymcdot}y{\isacharparenright}{\isacharparenright}{\isacharparenright}\ {\isacharequal}\isanewline
\ \ \ \ \ \ \ fproj{\isadigit{1}}{\isasymcdot}{\isacharparenleft}ffilter\ {\isacharbraceleft}a{\isachardot}\ {\isasymexists}b{\isachardot}\ a\ {\isacharequal}\ {\isacharparenleft}b{\isacharcomma}\ True{\isacharparenright}{\isacharbraceright}{\isasymcdot}{\isacharparenleft}fzip{\isasymcdot}x{\isasymcdot}{\isacharparenleft}rOrac{\isasymcdot}y{\isacharparenright}{\isacharparenright}{\isacharparenright}{\isachardoublequoteclose}\isanewline
\isadelimproof
\endisadelimproof
\isatagproof
\isacommand{apply}\isamarkupfalse%
\ {\isacharparenleft}rule\ fstream{\isacharunderscore}ind{\isadigit{1}}\ {\isacharbrackleft}of\ {\isacharunderscore}\ y{\isacharbrackright}{\isacharcomma}\ auto{\isacharparenright}\isanewline
\isacommand{apply}\isamarkupfalse%
\ {\isacharparenleft}case{\isacharunderscore}tac\ {\isachardoublequoteopen}x{\isacharequal}{\isasymepsilon}{\isachardoublequoteclose}{\isacharcomma}\ auto{\isacharparenright}\isanewline
\isacommand{apply}\isamarkupfalse%
\ {\isacharparenleft}drule\ fscase{\isadigit{2}}{\isacharcomma}\ auto{\isacharparenright}\isanewline
\isacommand{by}\isamarkupfalse%
\ {\isacharparenleft}case{\isacharunderscore}tac\ {\isachardoublequoteopen}a{\isacharequal}True{\isachardoublequoteclose}{\isacharcomma}\ auto{\isacharparenright}%
\endisatagproof
{\isafoldproof}%
\isadelimproof
\isanewline
\endisadelimproof
\isanewline
\isacommand{lemma}\isamarkupfalse%
\ rOrac{\isacharunderscore}lemma{\isadigit{2}}{\isacharcolon}\ \isanewline
\ \ {\isachardoublequoteopen}{\isasymforall}p{\isachardot}\ fft\ {\isacharparenleft}fdrop\ n{\isasymcdot}p{\isacharparenright}\ {\isasymlongrightarrow}\ fdrop\ {\isacharparenleft}Suc\ n{\isacharparenright}{\isasymcdot}{\isacharparenleft}rOrac{\isasymcdot}p{\isacharparenright}\ {\isacharequal}\ fdrop\ {\isacharparenleft}Suc\ n{\isacharparenright}{\isasymcdot}p{\isachardoublequoteclose}\ \isanewline
\isadelimproof
\endisadelimproof
\isatagproof
\isacommand{apply}\isamarkupfalse%
\ {\isacharparenleft}induct{\isacharunderscore}tac\ n{\isacharcomma}\ auto{\isacharparenright}\isanewline
\isacommand{apply}\isamarkupfalse%
\ {\isacharparenleft}case{\isacharunderscore}tac\ {\isachardoublequoteopen}p{\isacharequal}{\isasymepsilon}{\isachardoublequoteclose}{\isacharcomma}\ auto{\isacharparenright}\isanewline
\isacommand{apply}\isamarkupfalse%
\ {\isacharparenleft}drule\ fscase{\isadigit{2}}{\isacharcomma}\ auto{\isacharparenright}\isanewline
\isacommand{apply}\isamarkupfalse%
\ {\isacharparenleft}case{\isacharunderscore}tac\ {\isachardoublequoteopen}p{\isacharequal}{\isasymepsilon}{\isachardoublequoteclose}{\isacharcomma}\ auto{\isacharparenright}\isanewline
\isacommand{apply}\isamarkupfalse%
\ {\isacharparenleft}drule\ fscase{\isadigit{2}}{\isacharcomma}\ auto{\isacharparenright}\isanewline
\isacommand{by}\isamarkupfalse%
\ {\isacharparenleft}case{\isacharunderscore}tac\ a{\isacharcomma}\ auto{\isacharparenright}%
\endisatagproof
{\isafoldproof}%
\isadelimproof
\isanewline
\endisadelimproof
\isanewline
\isacommand{lemma}\isamarkupfalse%
\ rOrac{\isacharunderscore}lemma{\isadigit{3}}{\isacharcolon}\ \isanewline
\ \ {\isachardoublequoteopen}{\isacharhash}{\isacharparenleft}ffilter\ {\isacharbraceleft}True{\isacharbraceright}{\isasymcdot}p{\isacharparenright}\ {\isacharequal}\ {\isasyminfinity}\ {\isasymLongrightarrow}\ {\isacharhash}{\isacharparenleft}ffilter\ {\isacharbraceleft}True{\isacharbraceright}{\isasymcdot}{\isacharparenleft}rOrac{\isasymcdot}p{\isacharparenright}{\isacharparenright}\ {\isacharequal}\ {\isasyminfinity}{\isachardoublequoteclose}\isanewline
\isadelimproof
\endisadelimproof
\isatagproof
\isacommand{apply}\isamarkupfalse%
\ {\isacharparenleft}case{\isacharunderscore}tac\ {\isachardoublequoteopen}ffilter\ {\isacharbraceleft}True{\isacharbraceright}{\isasymcdot}p\ {\isacharequal}\ {\isasymepsilon}{\isachardoublequoteclose}{\isacharcomma}\ auto{\isacharparenright}\isanewline
\isacommand{apply}\isamarkupfalse%
\ {\isacharparenleft}drule\ ffilter{\isacharunderscore}lemma{\isadigit{3}}{\isacharcomma}\ erule\ exE{\isacharcomma}\ simp{\isacharparenright}\isanewline
\isacommand{apply}\isamarkupfalse%
\ {\isacharparenleft}drule\ rOrac{\isacharunderscore}lemma{\isadigit{2}}\ {\isacharbrackleft}rule{\isacharunderscore}format{\isacharbrackright}{\isacharparenright}\isanewline
\isacommand{apply}\isamarkupfalse%
\ {\isacharparenleft}insert\ fslen{\isacharunderscore}ffilter{\isacharunderscore}fdrop\ {\isacharbrackleft}of{\isacharbrackright}{\isacharcomma}\ atomize{\isacharparenright}\isanewline
\isacommand{apply}\isamarkupfalse%
\ {\isacharparenleft}erule{\isacharunderscore}tac\ x{\isacharequal}{\isachardoublequoteopen}Suc\ n{\isachardoublequoteclose}\ \isakeyword{in}\ allE{\isacharparenright}\isanewline
\isacommand{apply}\isamarkupfalse%
\ {\isacharparenleft}erule{\isacharunderscore}tac\ x{\isacharequal}{\isachardoublequoteopen}p{\isachardoublequoteclose}\ \isakeyword{in}\ allE{\isacharparenright}\isanewline
\isacommand{apply}\isamarkupfalse%
\ {\isacharparenleft}erule{\isacharunderscore}tac\ x{\isacharequal}{\isachardoublequoteopen}{\isacharbraceleft}True{\isacharbraceright}{\isachardoublequoteclose}\ \isakeyword{in}\ allE{\isacharcomma}\ simp{\isacharparenright}\isanewline
\isacommand{apply}\isamarkupfalse%
\ {\isacharparenleft}insert\ fslen{\isacharunderscore}ffilter{\isacharunderscore}fdrop{\isacharunderscore}rev\ \isanewline
\ \ \ \ \ \ \ \ \ {\isacharbrackleft}rule{\isacharunderscore}format{\isacharcomma}\ of\ {\isachardoublequoteopen}{\isacharbraceleft}True{\isacharbraceright}{\isachardoublequoteclose}\ {\isacharunderscore}\ {\isachardoublequoteopen}rOrac{\isasymcdot}p{\isachardoublequoteclose}{\isacharbrackright}{\isacharcomma}\ atomize{\isacharparenright}\isanewline
\isacommand{by}\isamarkupfalse%
\ {\isacharparenleft}erule{\isacharunderscore}tac\ x{\isacharequal}{\isachardoublequoteopen}Suc\ n{\isachardoublequoteclose}\ \isakeyword{in}\ allE{\isacharcomma}\ auto{\isacharparenright}%
\endisatagproof
{\isafoldproof}%
\isadelimproof
\isanewline
\endisadelimproof
\isanewline
\isacommand{lemma}\isamarkupfalse%
\ Med{\isacharunderscore}frt{\isacharunderscore}both{\isacharcolon}\ \isanewline
\ \ {\isachardoublequoteopen}Med\ x\ y\ {\isasymLongrightarrow}\ Med\ {\isacharparenleft}frt{\isasymcdot}x{\isacharparenright}\ {\isacharparenleft}frt{\isasymcdot}y{\isacharparenright}{\isachardoublequoteclose}\isanewline
\isadelimproof
\endisadelimproof
\isatagproof
\isacommand{apply}\isamarkupfalse%
\ {\isacharparenleft}auto\ simp\ add{\isacharcolon}\ Med{\isacharunderscore}def{\isacharparenright}\isanewline
\isacommand{apply}\isamarkupfalse%
\ {\isacharparenleft}case{\isacharunderscore}tac\ {\isachardoublequoteopen}p{\isacharequal}{\isasymepsilon}{\isachardoublequoteclose}{\isacharcomma}\ auto{\isacharparenright}\isanewline
\isacommand{apply}\isamarkupfalse%
\ {\isacharparenleft}drule\ fscase{\isadigit{2}}{\isacharcomma}\ auto{\isacharparenright}\isanewline
\isacommand{apply}\isamarkupfalse%
\ {\isacharparenleft}case{\isacharunderscore}tac\ {\isachardoublequoteopen}x{\isacharequal}{\isasymepsilon}{\isachardoublequoteclose}{\isacharcomma}\ auto{\isacharparenright}\isanewline
\isacommand{apply}\isamarkupfalse%
\ {\isacharparenleft}drule\ fscase{\isadigit{2}}{\isacharcomma}\ auto{\isacharparenright}\isanewline
\isacommand{apply}\isamarkupfalse%
\ {\isacharparenleft}case{\isacharunderscore}tac\ a{\isacharcomma}\ auto{\isacharparenright}\isanewline
\isacommand{apply}\isamarkupfalse%
\ {\isacharparenleft}rule{\isacharunderscore}tac\ x{\isacharequal}{\isachardoublequoteopen}rs{\isachardoublequoteclose}\ \isakeyword{in}\ exI{\isacharcomma}\ simp{\isacharparenright}\isanewline
\isacommand{apply}\isamarkupfalse%
\ {\isacharparenleft}simp\ add{\isacharcolon}\ inat{\isacharunderscore}defs\ split{\isacharcolon}\ inat{\isacharunderscore}splits{\isacharparenright}\isanewline
\isacommand{apply}\isamarkupfalse%
\ {\isacharparenleft}rule{\isacharunderscore}tac\ x{\isacharequal}{\isachardoublequoteopen}rOrac{\isasymcdot}rs{\isachardoublequoteclose}\ \isakeyword{in}\ exI{\isacharparenright}\isanewline
\isacommand{by}\isamarkupfalse%
\ {\isacharparenleft}auto\ simp\ add{\isacharcolon}\ rOrac{\isacharunderscore}lemma{\isadigit{1}}\ rOrac{\isacharunderscore}lemma{\isadigit{3}}{\isacharparenright}%
\endisatagproof
{\isafoldproof}%
\isadelimproof
\isanewline
\endisadelimproof
\isanewline
\isacommand{lemma}\isamarkupfalse%
\ Med{\isacharunderscore}lemma{\isadigit{1}}{\isacharbrackleft}rule{\isacharunderscore}format{\isacharbrackright}{\isacharcolon}\ \isanewline
\ \ {\isachardoublequoteopen}Med\ x\ {\isasymepsilon}\ {\isasymlongrightarrow}\ Med\ {\isacharparenleft}fdrop\ n{\isasymcdot}x{\isacharparenright}\ {\isasymepsilon}{\isachardoublequoteclose}\isanewline
\isadelimproof
\endisadelimproof
\isatagproof
\isacommand{apply}\isamarkupfalse%
\ {\isacharparenleft}induct{\isacharunderscore}tac\ n{\isacharcomma}\ auto{\isacharparenright}\isanewline
\isacommand{apply}\isamarkupfalse%
\ {\isacharparenleft}drule\ Med{\isacharunderscore}frt{\isacharunderscore}both{\isacharparenright}\isanewline
\isacommand{apply}\isamarkupfalse%
\ {\isacharparenleft}drule\ Med{\isacharunderscore}frt{\isacharunderscore}both{\isacharparenright}\isanewline
\isacommand{by}\isamarkupfalse%
\ {\isacharparenleft}simp\ add{\isacharcolon}\ fdrop{\isacharunderscore}unfold{\isadigit{2}}{\isacharparenright}%
\endisatagproof
{\isafoldproof}%
\isadelimproof
\isanewline
\endisadelimproof
\isanewline
\isacommand{lemma}\isamarkupfalse%
\ Med{\isacharunderscore}lemma{\isadigit{2}}{\isacharcolon}\ \isanewline
\ \ {\isachardoublequoteopen}{\isasymlbrakk}x\ {\isasymnoteq}\ {\isasymepsilon}{\isacharsemicolon}\ y\ {\isasymnoteq}\ {\isasymepsilon}{\isacharsemicolon}\ fft\ x\ {\isasymnoteq}\ fft\ y{\isacharsemicolon}\ Med\ x\ y{\isasymrbrakk}\ {\isasymLongrightarrow}\ Med\ {\isacharparenleft}frt{\isasymcdot}x{\isacharparenright}\ y{\isachardoublequoteclose}\isanewline
\isadelimproof
\endisadelimproof
\isatagproof
\isacommand{apply}\isamarkupfalse%
\ {\isacharparenleft}drule\ fscase{\isadigit{2}}{\isacharcomma}\ auto{\isacharparenright}{\isacharplus}\isanewline
\isacommand{apply}\isamarkupfalse%
\ {\isacharparenleft}auto\ simp\ add{\isacharcolon}\ Med{\isacharunderscore}def{\isacharparenright}\isanewline
\isacommand{apply}\isamarkupfalse%
\ {\isacharparenleft}case{\isacharunderscore}tac\ {\isachardoublequoteopen}p{\isacharequal}{\isasymepsilon}{\isachardoublequoteclose}{\isacharcomma}\ auto{\isacharparenright}\isanewline
\isacommand{apply}\isamarkupfalse%
\ {\isacharparenleft}drule\ fscase{\isadigit{2}}{\isacharcomma}\ auto{\isacharparenright}\isanewline
\isacommand{apply}\isamarkupfalse%
\ {\isacharparenleft}case{\isacharunderscore}tac\ ab{\isacharcomma}\ auto{\isacharparenright}\isanewline
\isacommand{by}\isamarkupfalse%
\ {\isacharparenleft}drule\ fscons{\isadigit{2}}{\isacharunderscore}injects{\isacharcomma}\ simp{\isacharparenright}%
\endisatagproof
{\isafoldproof}%
\isadelimproof
\isanewline
\endisadelimproof
\isanewline
\isacommand{lemma}\isamarkupfalse%
\ Med{\isacharunderscore}lemma{\isadigit{3}}{\isacharcolon}\ \isanewline
\ \ {\isachardoublequoteopen}{\isasymlbrakk}a\ {\isasymnoteq}\ b{\isacharsemicolon}\ Med\ {\isacharparenleft}{\isacharless}a{\isachargreater}\ {\isasymfrown}\ x{\isacharparenright}\ {\isacharparenleft}{\isacharless}b{\isachargreater}\ {\isasymfrown}\ y{\isacharparenright}{\isasymrbrakk}\ {\isasymLongrightarrow}\ Med\ x\ {\isacharparenleft}{\isacharless}b{\isachargreater}\ {\isasymfrown}\ y{\isacharparenright}{\isachardoublequoteclose}\isanewline
\isadelimproof
\endisadelimproof
\isatagproof
\isacommand{by}\isamarkupfalse%
\ {\isacharparenleft}insert\ Med{\isacharunderscore}lemma{\isadigit{2}}\ {\isacharbrackleft}of\ {\isachardoublequoteopen}{\isacharless}a{\isachargreater}\ {\isasymfrown}\ x{\isachardoublequoteclose}\ {\isachardoublequoteopen}{\isacharless}b{\isachargreater}\ {\isasymfrown}\ y{\isachardoublequoteclose}{\isacharbrackright}{\isacharcomma}\ auto{\isacharparenright}%
\endisatagproof
{\isafoldproof}%
\isadelimproof
\isanewline
\endisadelimproof
\isanewline
\isacommand{lemma}\isamarkupfalse%
\ Med{\isacharunderscore}lone{\isacharcolon}\ \isanewline
\ \ {\isachardoublequoteopen}Med\ {\isacharless}a{\isachargreater}\ y\ {\isasymLongrightarrow}\ y\ {\isacharequal}\ {\isacharless}a{\isachargreater}\ {\isasymor}\ y\ {\isacharequal}\ {\isasymepsilon}{\isachardoublequoteclose}\isanewline
\isadelimproof
\endisadelimproof
\isatagproof
\isacommand{apply}\isamarkupfalse%
\ {\isacharparenleft}auto{\isacharparenright}\isanewline
\isacommand{apply}\isamarkupfalse%
\ {\isacharparenleft}drule\ fscase{\isadigit{2}}{\isacharcomma}\ auto{\isacharparenright}\isanewline
\isacommand{apply}\isamarkupfalse%
\ {\isacharparenleft}case{\isacharunderscore}tac\ {\isachardoublequoteopen}rs{\isacharequal}{\isasymepsilon}{\isachardoublequoteclose}{\isacharcomma}\ auto{\isacharparenright}\isanewline
\isacommand{apply}\isamarkupfalse%
\ {\isacharparenleft}simp\ add{\isacharcolon}\ Med{\isacharunderscore}def{\isacharcomma}\ auto{\isacharparenright}\isanewline
\isacommand{apply}\isamarkupfalse%
\ {\isacharparenleft}case{\isacharunderscore}tac\ {\isachardoublequoteopen}p{\isacharequal}{\isasymepsilon}{\isachardoublequoteclose}{\isacharcomma}\ auto{\isacharparenright}\isanewline
\isacommand{apply}\isamarkupfalse%
\ {\isacharparenleft}drule\ fscase{\isadigit{2}}{\isacharcomma}\ auto{\isacharparenright}\isanewline
\isacommand{apply}\isamarkupfalse%
\ {\isacharparenleft}drule\ Med{\isacharunderscore}frt{\isacharunderscore}both{\isacharcomma}\ simp{\isacharparenright}\isanewline
\isacommand{by}\isamarkupfalse%
\ {\isacharparenleft}drule\ strict{\isacharunderscore}rev{\isacharunderscore}Med{\isacharcomma}\ simp{\isacharparenright}%
\endisatagproof
{\isafoldproof}%
\isadelimproof
\isanewline
\endisadelimproof
\isanewline
\isacommand{lemma}\isamarkupfalse%
\ Med{\isacharunderscore}lemma{\isadigit{4}}{\isacharcolon}\ \isanewline
\ \ {\isachardoublequoteopen}{\isasymforall}x{\isachardot}\ x\ {\isasymnoteq}\ {\isasymepsilon}\ {\isasymand}\ y\ {\isasymnoteq}\ {\isasymepsilon}\ {\isasymand}\ fft\ x\ {\isasymnoteq}\ fft\ y\ {\isasymand}\ \ \isanewline
\ \ \ \ \ \ \ Med\ x\ y\ {\isasymand}\ {\isacharhash}{\isacharparenleft}fftx{\isasymcdot}x{\isacharparenright}\ {\isacharequal}\ Fin\ k\ {\isasymlongrightarrow}\ Med\ {\isacharparenleft}frtx{\isasymcdot}x{\isacharparenright}\ y{\isachardoublequoteclose}\ \isanewline
\isadelimproof
\endisadelimproof
\isatagproof
\isacommand{apply}\isamarkupfalse%
\ {\isacharparenleft}induct{\isacharunderscore}tac\ k{\isacharcomma}\ auto{\isacharparenright}\isanewline
\isacommand{apply}\isamarkupfalse%
\ {\isacharparenleft}simp\ add{\isacharcolon}\ Fin{\isacharunderscore}{\isadigit{0}}{\isacharparenright}\isanewline
\isacommand{apply}\isamarkupfalse%
\ {\isacharparenleft}drule\ strict{\isacharunderscore}rev{\isacharunderscore}fftx{\isacharcomma}\ simp{\isacharparenright}\isanewline
\isacommand{apply}\isamarkupfalse%
\ {\isacharparenleft}drule\ fscase{\isadigit{2}}{\isacharcomma}\ auto{\isacharparenright}{\isacharplus}\isanewline
\isacommand{apply}\isamarkupfalse%
\ {\isacharparenleft}case{\isacharunderscore}tac\ {\isachardoublequoteopen}rs\ {\isacharequal}\ {\isasymepsilon}{\isachardoublequoteclose}{\isacharcomma}\ auto{\isacharparenright}\isanewline
\isacommand{apply}\isamarkupfalse%
\ {\isacharparenleft}drule\ Med{\isacharunderscore}lone{\isacharcomma}\ auto{\isacharparenright}\ \isanewline
\isacommand{apply}\isamarkupfalse%
\ {\isacharparenleft}drule\ lone{\isacharunderscore}lemma{\isadigit{1}}{\isacharcomma}\ auto{\isacharparenright}\isanewline
\isacommand{apply}\isamarkupfalse%
\ {\isacharparenleft}drule\ fscase{\isadigit{2}}{\isacharcomma}\ auto{\isacharparenright}\isanewline
\isacommand{apply}\isamarkupfalse%
\ {\isacharparenleft}case{\isacharunderscore}tac\ {\isachardoublequoteopen}a{\isacharequal}ab{\isachardoublequoteclose}{\isacharcomma}\ auto{\isacharparenright}\isanewline
\isacommand{apply}\isamarkupfalse%
\ {\isacharparenleft}erule{\isacharunderscore}tac\ x{\isacharequal}{\isachardoublequoteopen}{\isacharless}ab{\isachargreater}\ {\isasymfrown}\ rsb{\isachardoublequoteclose}\ \isakeyword{in}\ allE{\isacharcomma}\ auto{\isacharparenright}\isanewline
\isacommand{apply}\isamarkupfalse%
\ {\isacharparenleft}rule\ Med{\isacharunderscore}lemma{\isadigit{3}}\ {\isacharbrackleft}rule{\isacharunderscore}format{\isacharbrackright}{\isacharcomma}\ auto{\isacharparenright}\isanewline
\isacommand{apply}\isamarkupfalse%
\ {\isacharparenleft}simp\ add{\isacharcolon}\ inat{\isacharunderscore}defs\ split{\isacharcolon}\ inat{\isacharunderscore}splits{\isacharparenright}\isanewline
\isacommand{by}\isamarkupfalse%
\ {\isacharparenleft}rule\ Med{\isacharunderscore}lemma{\isadigit{3}}\ {\isacharbrackleft}rule{\isacharunderscore}format{\isacharbrackright}{\isacharcomma}\ auto{\isacharparenright}%
\endisatagproof
{\isafoldproof}%
\isadelimproof
\isanewline
\endisadelimproof
\isanewline
\isacommand{lemma}\isamarkupfalse%
\ Med{\isacharunderscore}lemma{\isadigit{5}}{\isacharcolon}\ \isanewline
\ \ {\isachardoublequoteopen}{\isasymlbrakk}Med\ x\ y{\isacharsemicolon}\ {\isacharhash}{\isacharparenleft}fftx{\isasymcdot}x{\isacharparenright}\ {\isacharequal}\ Fin\ k{\isacharsemicolon}\ {\isacharhash}{\isacharparenleft}fftx{\isasymcdot}y{\isacharparenright}\ {\isacharequal}\ Fin\ m{\isasymrbrakk}\ {\isasymLongrightarrow}\ Med\ {\isacharparenleft}frtx{\isasymcdot}x{\isacharparenright}\ {\isacharparenleft}frtx{\isasymcdot}y{\isacharparenright}{\isachardoublequoteclose}\ \isanewline
\isadelimproof
\endisadelimproof
\isatagproof
\isacommand{apply}\isamarkupfalse%
\ {\isacharparenleft}case{\isacharunderscore}tac\ k{\isacharcomma}\ auto{\isacharparenright}\isanewline
\isacommand{apply}\isamarkupfalse%
\ {\isacharparenleft}simp\ add{\isacharcolon}\ Fin{\isacharunderscore}{\isadigit{0}}{\isacharparenright}\isanewline
\isacommand{apply}\isamarkupfalse%
\ {\isacharparenleft}drule\ strict{\isacharunderscore}rev{\isacharunderscore}fftx{\isacharcomma}\ simp{\isacharparenright}\isanewline
\isacommand{apply}\isamarkupfalse%
\ {\isacharparenleft}drule\ strict{\isacharunderscore}rev{\isacharunderscore}Med{\isacharcomma}\ simp{\isacharparenright}\isanewline
\isacommand{apply}\isamarkupfalse%
\ {\isacharparenleft}case{\isacharunderscore}tac\ m{\isacharcomma}\ auto{\isacharparenright}\isanewline
\isacommand{apply}\isamarkupfalse%
\ {\isacharparenleft}simp\ add{\isacharcolon}\ Fin{\isacharunderscore}{\isadigit{0}}{\isacharparenright}\isanewline
\isacommand{apply}\isamarkupfalse%
\ {\isacharparenleft}drule\ strict{\isacharunderscore}rev{\isacharunderscore}fftx{\isacharcomma}\ simp{\isacharparenright}\isanewline
\isacommand{apply}\isamarkupfalse%
\ {\isacharparenleft}simp\ add{\isacharcolon}\ frtx{\isadigit{2}}fdrop{\isacharparenright}\isanewline
\isacommand{apply}\isamarkupfalse%
\ {\isacharparenleft}rule\ Med{\isacharunderscore}lemma{\isadigit{1}}{\isacharcomma}\ simp{\isacharparenright}\isanewline
\isacommand{apply}\isamarkupfalse%
\ {\isacharparenleft}case{\isacharunderscore}tac\ {\isachardoublequoteopen}x{\isacharequal}{\isasymepsilon}{\isachardoublequoteclose}{\isacharcomma}\ auto{\isacharparenright}\isanewline
\isacommand{apply}\isamarkupfalse%
\ {\isacharparenleft}simp\ add{\isacharcolon}\ inat{\isacharunderscore}defs\ split{\isacharcolon}\ inat{\isacharunderscore}splits{\isacharparenright}\isanewline
\isacommand{apply}\isamarkupfalse%
\ {\isacharparenleft}case{\isacharunderscore}tac\ {\isachardoublequoteopen}y{\isacharequal}{\isasymepsilon}{\isachardoublequoteclose}{\isacharcomma}\ auto{\isacharparenright}\isanewline
\isacommand{apply}\isamarkupfalse%
\ {\isacharparenleft}simp\ add{\isacharcolon}\ inat{\isacharunderscore}defs\ split{\isacharcolon}\ inat{\isacharunderscore}splits{\isacharparenright}\isanewline
\isacommand{apply}\isamarkupfalse%
\ {\isacharparenleft}case{\isacharunderscore}tac\ {\isachardoublequoteopen}fft\ x\ {\isasymnoteq}\ fft\ y{\isachardoublequoteclose}{\isacharcomma}\ auto{\isacharparenright}\isanewline
\isacommand{apply}\isamarkupfalse%
\ {\isacharparenleft}subgoal{\isacharunderscore}tac\ {\isachardoublequoteopen}Med\ {\isacharparenleft}frtx{\isasymcdot}x{\isacharparenright}\ y{\isachardoublequoteclose}{\isacharparenright}\isanewline
\isacommand{apply}\isamarkupfalse%
\ {\isacharparenleft}simp\ add{\isacharcolon}\ frtx{\isadigit{2}}fdrop{\isacharparenright}\isanewline
\isacommand{apply}\isamarkupfalse%
\ {\isacharparenleft}drule\ Med{\isacharunderscore}fdrop{\isadigit{2}}\ {\isacharbrackleft}rule{\isacharunderscore}format{\isacharbrackright}{\isacharparenright}\isanewline
\isacommand{apply}\isamarkupfalse%
\ {\isacharparenleft}drule\ Med{\isacharunderscore}fdrop{\isadigit{2}}\ {\isacharbrackleft}rule{\isacharunderscore}format{\isacharbrackright}{\isacharcomma}\ auto{\isacharparenright}\isanewline
\isacommand{apply}\isamarkupfalse%
\ {\isacharparenleft}rule\ Med{\isacharunderscore}lemma{\isadigit{4}}\ {\isacharbrackleft}rule{\isacharunderscore}format{\isacharbrackright}{\isacharcomma}\ auto{\isacharparenright}\isanewline
\isacommand{apply}\isamarkupfalse%
\ {\isacharparenleft}subgoal{\isacharunderscore}tac\ {\isachardoublequoteopen}Med\ x\ {\isacharparenleft}frtx{\isasymcdot}y{\isacharparenright}{\isachardoublequoteclose}{\isacharparenright}\isanewline
\isacommand{apply}\isamarkupfalse%
\ {\isacharparenleft}case{\isacharunderscore}tac\ {\isachardoublequoteopen}frtx{\isasymcdot}y\ {\isacharequal}\ {\isasymepsilon}{\isachardoublequoteclose}{\isacharcomma}\ auto{\isacharparenright}\isanewline
\isacommand{apply}\isamarkupfalse%
\ {\isacharparenleft}subst\ frtx{\isadigit{2}}fdrop{\isacharcomma}\ auto{\isacharparenright}\isanewline
\isacommand{apply}\isamarkupfalse%
\ {\isacharparenleft}rule\ Med{\isacharunderscore}lemma{\isadigit{1}}{\isacharcomma}\ assumption{\isacharparenright}\isanewline
\isacommand{apply}\isamarkupfalse%
\ {\isacharparenleft}subgoal{\isacharunderscore}tac\ {\isachardoublequoteopen}fft\ x\ {\isasymnoteq}\ fft\ {\isacharparenleft}frtx{\isasymcdot}y{\isacharparenright}{\isachardoublequoteclose}{\isacharparenright}\isanewline
\isacommand{apply}\isamarkupfalse%
\ {\isacharparenleft}rule\ Med{\isacharunderscore}lemma{\isadigit{4}}\ {\isacharbrackleft}rule{\isacharunderscore}format{\isacharbrackright}{\isacharcomma}\ auto{\isacharparenright}\isanewline
\isacommand{apply}\isamarkupfalse%
\ {\isacharparenleft}simp\ add{\isacharcolon}\ fft{\isacharunderscore}neq{\isacharunderscore}fft{\isacharunderscore}frtx{\isacharunderscore}lemma{\isacharparenright}\ \isanewline
\isacommand{apply}\isamarkupfalse%
\ {\isacharparenleft}subst\ frtx{\isadigit{2}}fdrop{\isacharcomma}\ auto{\isacharparenright}\isanewline
\isacommand{by}\isamarkupfalse%
\ {\isacharparenleft}rule\ Med{\isacharunderscore}fdrop{\isadigit{2}}\ {\isacharbrackleft}rule{\isacharunderscore}format{\isacharbrackright}{\isacharparenright}%
\endisatagproof
{\isafoldproof}%
\isadelimproof
\isanewline
\endisadelimproof
\isanewline
\isacommand{lemma}\isamarkupfalse%
\ fftx{\isacharunderscore}inf{\isacharunderscore}Med{\isacharunderscore}lemma{\isacharcolon}\ \isanewline
\ \ {\isachardoublequoteopen}{\isasymforall}p{\isachardot}\ frtx{\isasymcdot}x\ {\isacharequal}\ {\isasymepsilon}\ {\isasymlongrightarrow}\ \isanewline
\ \ \ \ \ \ \ fproj{\isadigit{1}}{\isasymcdot}{\isacharparenleft}ffilter\ {\isacharbraceleft}a{\isachardot}\ {\isasymexists}b{\isachardot}\ a\ {\isacharequal}\ {\isacharparenleft}b{\isacharcomma}\ True{\isacharparenright}{\isacharbraceright}{\isasymcdot}{\isacharparenleft}fzip{\isasymcdot}x{\isasymcdot}p{\isacharparenright}{\isacharparenright}\ {\isasymsqsubseteq}\ x{\isachardoublequoteclose}\isanewline
\isadelimproof
\endisadelimproof
\isatagproof
\isacommand{apply}\isamarkupfalse%
\ {\isacharparenleft}rule\ fstream{\isacharunderscore}ind{\isadigit{1}}\ {\isacharbrackleft}of\ {\isacharunderscore}\ x{\isacharbrackright}{\isacharcomma}\ auto{\isacharparenright}\isanewline
\isacommand{apply}\isamarkupfalse%
\ {\isacharparenleft}case{\isacharunderscore}tac\ {\isachardoublequoteopen}s{\isacharequal}{\isasymepsilon}{\isachardoublequoteclose}{\isacharcomma}\ auto{\isacharparenright}\isanewline
\isacommand{apply}\isamarkupfalse%
\ {\isacharparenleft}drule\ fscase{\isadigit{2}}{\isacharcomma}\ auto{\isacharparenright}{\isacharplus}\isanewline
\isacommand{apply}\isamarkupfalse%
\ {\isacharparenleft}case{\isacharunderscore}tac\ {\isachardoublequoteopen}a{\isacharequal}ab{\isachardoublequoteclose}{\isacharcomma}\ auto{\isacharparenright}\isanewline
\isacommand{apply}\isamarkupfalse%
\ {\isacharparenleft}case{\isacharunderscore}tac\ {\isachardoublequoteopen}p{\isacharequal}{\isasymepsilon}{\isachardoublequoteclose}{\isacharcomma}\ auto{\isacharparenright}\isanewline
\isacommand{apply}\isamarkupfalse%
\ {\isacharparenleft}drule\ fscase{\isadigit{2}}{\isacharcomma}\ auto{\isacharparenright}\isanewline
\isacommand{apply}\isamarkupfalse%
\ {\isacharparenleft}case{\isacharunderscore}tac\ aa{\isacharcomma}\ auto{\isacharparenright}\isanewline
\isacommand{apply}\isamarkupfalse%
\ {\isacharparenleft}rule\ monofun{\isacharunderscore}cfun{\isacharunderscore}arg{\isacharcomma}\ simp{\isacharparenright}\isanewline
\isacommand{apply}\isamarkupfalse%
\ {\isacharparenleft}erule{\isacharunderscore}tac\ x{\isacharequal}{\isachardoublequoteopen}rs{\isachardoublequoteclose}\ \isakeyword{in}\ allE{\isacharparenright}\isanewline
\isacommand{apply}\isamarkupfalse%
\ {\isacharparenleft}drule\ frtx{\isacharunderscore}eps{\isacharunderscore}to{\isacharunderscore}less{\isacharunderscore}lemma\ {\isacharbrackleft}rule{\isacharunderscore}format{\isacharbrackright}{\isacharparenright}\isanewline
\isacommand{by}\isamarkupfalse%
\ {\isacharparenleft}rule\ trans{\isacharunderscore}less{\isacharcomma}\ auto{\isacharparenright}%
\endisatagproof
{\isafoldproof}%
\isadelimproof
\isanewline
\endisadelimproof
\isanewline
\isacommand{lemma}\isamarkupfalse%
\ fftx{\isacharunderscore}inf{\isacharunderscore}Med{\isacharcolon}\ \isanewline
\ \ {\isachardoublequoteopen}{\isasymlbrakk}Med\ x\ y{\isacharsemicolon}\ {\isacharhash}{\isacharparenleft}fftx{\isasymcdot}x{\isacharparenright}\ {\isacharequal}\ {\isasyminfinity}{\isasymrbrakk}\ {\isasymLongrightarrow}\ x\ {\isacharequal}\ y{\isachardoublequoteclose}\isanewline
\isadelimproof
\endisadelimproof
\isatagproof
\isacommand{apply}\isamarkupfalse%
\ {\isacharparenleft}frule\ fftx{\isacharunderscore}inf{\isacharparenright}\isanewline
\isacommand{apply}\isamarkupfalse%
\ {\isacharparenleft}frule\ fair{\isacharunderscore}Med{\isacharcomma}\ auto{\isacharparenright}\isanewline
\isacommand{apply}\isamarkupfalse%
\ {\isacharparenleft}drule\ frtx{\isacharunderscore}empty{\isacharparenright}\isanewline
\isacommand{apply}\isamarkupfalse%
\ {\isacharparenleft}auto\ simp\ add{\isacharcolon}\ Med{\isacharunderscore}def{\isacharparenright}\isanewline
\isacommand{apply}\isamarkupfalse%
\ {\isacharparenleft}rule\ sym{\isacharparenright}\isanewline
\isacommand{apply}\isamarkupfalse%
\ {\isacharparenleft}rule\ size{\isacharunderscore}eq{\isacharcomma}\ auto{\isacharparenright}\isanewline
\isacommand{by}\isamarkupfalse%
\ {\isacharparenleft}rule\ fftx{\isacharunderscore}inf{\isacharunderscore}Med{\isacharunderscore}lemma\ {\isacharbrackleft}rule{\isacharunderscore}format{\isacharbrackright}{\isacharparenright}%
\endisatagproof
{\isafoldproof}%
\isadelimproof
\endisadelimproof
\begin{isamarkuptext}%
The following unfolding property for the predicate {\pisastyle{Med}} 
plays a key role in the proof of {\pisastyle{Med\_trans\_lemma}}, which
is located at the end of this theory.%
\end{isamarkuptext}%
\isamarkuptrue%
\isacommand{lemma}\isamarkupfalse%
\ Med{\isacharunderscore}burst{\isacharunderscore}lemma{\isacharcolon}\ \isanewline
\ \ {\isachardoublequoteopen}{\isasymlbrakk}{\isacharhash}{\isacharparenleft}fftx{\isasymcdot}y{\isacharparenright}\ {\isacharequal}\ Fin\ k{\isacharsemicolon}\ Med\ x\ y{\isasymrbrakk}\ {\isasymLongrightarrow}\ Med\ {\isacharparenleft}frtx{\isasymcdot}x{\isacharparenright}\ {\isacharparenleft}frtx{\isasymcdot}y{\isacharparenright}{\isachardoublequoteclose}\ \isanewline
\isadelimproof
\endisadelimproof
\isatagproof
\isacommand{apply}\isamarkupfalse%
\ {\isacharparenleft}case{\isacharunderscore}tac\ {\isachardoublequoteopen}{\isacharhash}{\isacharparenleft}fftx{\isasymcdot}x{\isacharparenright}{\isachardoublequoteclose}{\isacharparenright}\isanewline
\isacommand{apply}\isamarkupfalse%
\ {\isacharparenleft}rule\ Med{\isacharunderscore}lemma{\isadigit{5}}{\isacharcomma}\ assumption{\isacharplus}{\isacharparenright}\isanewline
\isacommand{by}\isamarkupfalse%
\ {\isacharparenleft}drule\ fftx{\isacharunderscore}inf{\isacharunderscore}Med{\isacharcomma}\ auto{\isacharparenright}%
\endisatagproof
{\isafoldproof}%
\isadelimproof
\endisadelimproof
\begin{isamarkuptext}%
Now, we prove some properties of {\pisastyle{Med}} also involving the length function on streams.%
\end{isamarkuptext}%
\isamarkuptrue%
\isacommand{lemma}\isamarkupfalse%
\ fnub{\isacharunderscore}less{\isacharunderscore}Med{\isacharunderscore}lemma{\isacharcolon}\ \isanewline
\ \ {\isachardoublequoteopen}{\isasymforall}x\ y{\isachardot}\ Med\ x\ y\ {\isasymand}\ {\isacharhash}{\isacharparenleft}fnub{\isasymcdot}x{\isacharparenright}\ {\isacharequal}\ Fin\ k\ {\isasymlongrightarrow}\ {\isacharhash}{\isacharparenleft}fnub{\isasymcdot}y{\isacharparenright}\ {\isasymle}\ {\isacharhash}{\isacharparenleft}fnub{\isasymcdot}x{\isacharparenright}{\isachardoublequoteclose}\isanewline
\isadelimproof
\endisadelimproof
\isatagproof
\isacommand{apply}\isamarkupfalse%
\ {\isacharparenleft}induct{\isacharunderscore}tac\ k{\isacharcomma}\ auto{\isacharparenright}\isanewline
\isacommand{apply}\isamarkupfalse%
\ {\isacharparenleft}simp\ add{\isacharcolon}\ Fin{\isacharunderscore}{\isadigit{0}}{\isacharparenright}\isanewline
\isacommand{apply}\isamarkupfalse%
\ {\isacharparenleft}drule\ strict{\isacharunderscore}rev{\isacharunderscore}fnub\ {\isacharbrackleft}rule{\isacharunderscore}format{\isacharbrackright}{\isacharcomma}\ simp{\isacharparenright}\isanewline
\isacommand{apply}\isamarkupfalse%
\ {\isacharparenleft}drule\ strict{\isacharunderscore}rev{\isacharunderscore}Med{\isacharcomma}\ simp{\isacharparenright}\isanewline
\isacommand{apply}\isamarkupfalse%
\ {\isacharparenleft}case{\isacharunderscore}tac\ {\isachardoublequoteopen}{\isacharhash}{\isacharparenleft}fftx{\isasymcdot}y{\isacharparenright}{\isachardoublequoteclose}{\isacharparenright}\isanewline
\isacommand{apply}\isamarkupfalse%
\ {\isacharparenleft}case{\isacharunderscore}tac\ {\isachardoublequoteopen}fnub{\isasymcdot}x\ {\isacharequal}\ {\isasymepsilon}{\isachardoublequoteclose}{\isacharcomma}\ auto{\isacharparenright}\isanewline
\isacommand{apply}\isamarkupfalse%
\ {\isacharparenleft}simp\ add{\isacharcolon}\ inat{\isacharunderscore}defs\ split{\isacharcolon}\ inat{\isacharunderscore}splits{\isacharparenright}\isanewline
\isacommand{apply}\isamarkupfalse%
\ {\isacharparenleft}drule\ fscase{\isadigit{2}}{\isacharcomma}\ auto{\isacharparenright}\isanewline
\isacommand{apply}\isamarkupfalse%
\ {\isacharparenleft}erule{\isacharunderscore}tac\ x{\isacharequal}{\isachardoublequoteopen}frtx{\isasymcdot}x{\isachardoublequoteclose}\ \isakeyword{in}\ allE{\isacharparenright}\isanewline
\isacommand{apply}\isamarkupfalse%
\ {\isacharparenleft}erule{\isacharunderscore}tac\ x{\isacharequal}{\isachardoublequoteopen}frtx{\isasymcdot}y{\isachardoublequoteclose}\ \isakeyword{in}\ allE{\isacharcomma}\ auto{\isacharparenright}\isanewline
\isacommand{apply}\isamarkupfalse%
\ {\isacharparenleft}simp\ add{\isacharcolon}\ Med{\isacharunderscore}burst{\isacharunderscore}lemma{\isacharparenright}\isanewline
\isacommand{apply}\isamarkupfalse%
\ {\isacharparenleft}simp\ add{\isacharcolon}\ inat{\isacharunderscore}defs\ split{\isacharcolon}\ inat{\isacharunderscore}splits{\isacharparenright}\isanewline
\isacommand{apply}\isamarkupfalse%
\ {\isacharparenleft}rule\ fslen{\isacharunderscore}frt{\isacharunderscore}{\isadigit{2}}{\isacharunderscore}less{\isacharcomma}\ assumption{\isacharparenright}\isanewline
\isacommand{apply}\isamarkupfalse%
\ {\isacharparenleft}drule\ fnub{\isacharunderscore}lemma{\isadigit{2}}{\isacharparenright}\isanewline
\isacommand{by}\isamarkupfalse%
\ {\isacharparenleft}simp\ add{\isacharcolon}\ inat{\isacharunderscore}defs\ split{\isacharcolon}\ inat{\isacharunderscore}splits{\isacharparenright}%
\endisatagproof
{\isafoldproof}%
\isadelimproof
\isanewline
\endisadelimproof
\isanewline
\isacommand{lemma}\isamarkupfalse%
\ fnub{\isacharunderscore}less{\isacharunderscore}Med{\isacharcolon}\ \isanewline
\ \ {\isachardoublequoteopen}Med\ x\ y\ {\isasymLongrightarrow}\ {\isacharhash}{\isacharparenleft}fnub{\isasymcdot}y{\isacharparenright}\ {\isasymle}\ {\isacharhash}{\isacharparenleft}fnub{\isasymcdot}x{\isacharparenright}{\isachardoublequoteclose}\isanewline
\isadelimproof
\endisadelimproof
\isatagproof
\isacommand{apply}\isamarkupfalse%
\ {\isacharparenleft}case{\isacharunderscore}tac\ {\isachardoublequoteopen}{\isacharhash}{\isacharparenleft}fnub{\isasymcdot}x{\isacharparenright}{\isachardoublequoteclose}{\isacharparenright}\isanewline
\isacommand{by}\isamarkupfalse%
\ {\isacharparenleft}rule\ fnub{\isacharunderscore}less{\isacharunderscore}Med{\isacharunderscore}lemma\ {\isacharbrackleft}rule{\isacharunderscore}format{\isacharbrackright}{\isacharcomma}\ auto{\isacharparenright}%
\endisatagproof
{\isafoldproof}%
\isadelimproof
\isanewline
\endisadelimproof
\isanewline
\isacommand{lemma}\isamarkupfalse%
\ Med{\isacharunderscore}fslen{\isacharunderscore}lemma{\isacharcolon}\isanewline
\ \ {\isachardoublequoteopen}{\isasymforall}x\ y{\isachardot}\ Med\ x\ y\ {\isasymand}\ {\isacharhash}x\ {\isacharequal}\ Fin\ k\ {\isasymlongrightarrow}\ {\isacharhash}y\ {\isasymle}\ Fin\ k{\isachardoublequoteclose}\isanewline
\isadelimproof
\endisadelimproof
\isatagproof
\isacommand{apply}\isamarkupfalse%
\ {\isacharparenleft}induct{\isacharunderscore}tac\ k{\isacharcomma}\ auto{\isacharparenright}\isanewline
\isacommand{apply}\isamarkupfalse%
\ {\isacharparenleft}simp\ add{\isacharcolon}\ Fin{\isacharunderscore}{\isadigit{0}}{\isacharparenright}\isanewline
\isacommand{apply}\isamarkupfalse%
\ {\isacharparenleft}drule\ strict{\isacharunderscore}rev{\isacharunderscore}Med{\isacharcomma}\ simp{\isacharparenright}\isanewline
\isacommand{apply}\isamarkupfalse%
\ {\isacharparenleft}erule{\isacharunderscore}tac\ x{\isacharequal}{\isachardoublequoteopen}frt{\isasymcdot}x{\isachardoublequoteclose}\ \isakeyword{in}\ allE{\isacharparenright}\isanewline
\isacommand{apply}\isamarkupfalse%
\ {\isacharparenleft}erule{\isacharunderscore}tac\ x{\isacharequal}{\isachardoublequoteopen}frt{\isasymcdot}y{\isachardoublequoteclose}\ \isakeyword{in}\ allE{\isacharcomma}\ auto{\isacharparenright}\isanewline
\isacommand{apply}\isamarkupfalse%
\ {\isacharparenleft}rule\ Med{\isacharunderscore}frt{\isacharunderscore}both{\isacharcomma}\ assumption{\isacharparenright}\isanewline
\isacommand{apply}\isamarkupfalse%
\ {\isacharparenleft}rule\ fslen{\isacharunderscore}Suc{\isacharunderscore}Suc{\isacharunderscore}{\isadigit{2}}{\isacharunderscore}frt{\isacharcomma}\ assumption{\isacharparenright}\isanewline
\isacommand{by}\isamarkupfalse%
\ {\isacharparenleft}rule\ fslen{\isacharunderscore}frt{\isacharunderscore}{\isadigit{2}}{\isacharunderscore}less{\isacharparenright}%
\endisatagproof
{\isafoldproof}%
\isadelimproof
\isanewline
\endisadelimproof
\isanewline
\isacommand{lemma}\isamarkupfalse%
\ Med{\isacharunderscore}fslen{\isacharcolon}\isanewline
\ \ {\isachardoublequoteopen}Med\ x\ y\ {\isasymLongrightarrow}\ {\isacharhash}y\ {\isasymle}\ {\isacharhash}x{\isachardoublequoteclose}\isanewline
\isadelimproof
\endisadelimproof
\isatagproof
\isacommand{apply}\isamarkupfalse%
\ {\isacharparenleft}case{\isacharunderscore}tac\ {\isachardoublequoteopen}{\isacharhash}x{\isachardoublequoteclose}{\isacharcomma}\ auto{\isacharparenright}\isanewline
\isacommand{by}\isamarkupfalse%
\ {\isacharparenleft}rule\ Med{\isacharunderscore}fslen{\isacharunderscore}lemma\ {\isacharbrackleft}rule{\isacharunderscore}format{\isacharbrackright}{\isacharcomma}\ auto{\isacharparenright}%
\endisatagproof
{\isafoldproof}%
\isadelimproof
\isanewline
\endisadelimproof
\isanewline
\isacommand{lemma}\isamarkupfalse%
\ fnub{\isacharunderscore}eq{\isacharunderscore}Med{\isacharunderscore}lemma{\isacharcolon}\ \isanewline
\ \ {\isachardoublequoteopen}{\isasymlbrakk}{\isacharhash}fftx{\isasymcdot}x\ {\isacharequal}\ Fin\ n{\isacharsemicolon}\ Med\ x\ y{\isacharsemicolon}\ frtx{\isasymcdot}x\ {\isacharequal}\ {\isasymepsilon}{\isasymrbrakk}\ {\isasymLongrightarrow}\ {\isacharhash}y\ {\isasymnoteq}\ {\isasyminfinity}{\isachardoublequoteclose}\isanewline
\isadelimproof
\endisadelimproof
\isatagproof
\isacommand{apply}\isamarkupfalse%
\ {\isacharparenleft}subgoal{\isacharunderscore}tac\ {\isachardoublequoteopen}{\isacharhash}x\ {\isacharequal}\ Fin\ n{\isachardoublequoteclose}{\isacharparenright}\isanewline
\isacommand{apply}\isamarkupfalse%
\ {\isacharparenleft}rule\ ccontr{\isacharcomma}\ simp{\isacharparenright}\isanewline
\isacommand{apply}\isamarkupfalse%
\ {\isacharparenleft}drule\ Med{\isacharunderscore}fslen{\isacharparenright}\isanewline
\isacommand{apply}\isamarkupfalse%
\ {\isacharparenleft}simp\ add{\isacharcolon}\ inat{\isacharunderscore}defs\ split{\isacharcolon}\ inat{\isacharunderscore}splits{\isacharparenright}\isanewline
\isacommand{by}\isamarkupfalse%
\ {\isacharparenleft}subst\ frtx{\isacharunderscore}empty{\isacharunderscore}fftx\ {\isacharbrackleft}THEN\ sym{\isacharbrackright}{\isacharcomma}\ auto{\isacharparenright}%
\endisatagproof
{\isafoldproof}%
\isadelimproof
\isanewline
\endisadelimproof
\isanewline
\isacommand{lemma}\isamarkupfalse%
\ fnub{\isacharunderscore}eq{\isacharunderscore}Med{\isacharunderscore}lemma{\isadigit{1}}{\isacharcolon}\ \isanewline
\ \ {\isachardoublequoteopen}{\isasymlbrakk}{\isacharhash}{\isacharparenleft}fftx{\isasymcdot}x{\isacharparenright}\ {\isacharequal}\ Fin\ n{\isacharsemicolon}\ Med\ x\ y{\isacharsemicolon}\ {\isacharhash}{\isacharparenleft}fnub{\isasymcdot}x{\isacharparenright}\ {\isacharequal}\ Fin\ {\isacharparenleft}Suc\ {\isadigit{0}}{\isacharparenright}{\isasymrbrakk}\ {\isasymLongrightarrow}\ {\isacharhash}y\ {\isasymnoteq}\ {\isasyminfinity}{\isachardoublequoteclose}\ \isanewline
\isadelimproof
\endisadelimproof
\isatagproof
\isacommand{apply}\isamarkupfalse%
\ {\isacharparenleft}subgoal{\isacharunderscore}tac\ {\isachardoublequoteopen}frtx{\isasymcdot}x\ {\isacharequal}\ {\isasymepsilon}{\isachardoublequoteclose}{\isacharparenright}\isanewline
\isacommand{apply}\isamarkupfalse%
\ {\isacharparenleft}rule\ fnub{\isacharunderscore}eq{\isacharunderscore}Med{\isacharunderscore}lemma\ {\isacharbrackleft}rule{\isacharunderscore}format{\isacharbrackright}{\isacharcomma}\ auto{\isacharparenright}\isanewline
\isacommand{by}\isamarkupfalse%
\ {\isacharparenleft}rule\ fslen{\isacharunderscore}fnub{\isacharunderscore}Suc{\isadigit{0}}{\isacharparenright}%
\endisatagproof
{\isafoldproof}%
\isadelimproof
\endisadelimproof
\begin{isamarkuptext}%
The following lemma states the equality of the input and output streams
on the input and output channel of $Medium$ if the consecutive repetitions 
are removed and such streams are finite and of equal length.%
\end{isamarkuptext}%
\isamarkuptrue%
\isacommand{lemma}\isamarkupfalse%
\ fnub{\isacharunderscore}eq{\isacharunderscore}Med{\isacharcolon}\ \isanewline
\ \ {\isachardoublequoteopen}{\isasymforall}x\ y{\isachardot}\ {\isacharhash}{\isacharparenleft}fnub{\isasymcdot}x{\isacharparenright}\ {\isacharequal}\ {\isacharhash}{\isacharparenleft}fnub{\isasymcdot}y{\isacharparenright}\ {\isasymand}\ {\isacharhash}{\isacharparenleft}fnub{\isasymcdot}x{\isacharparenright}\ {\isacharequal}\ Fin\ k\ {\isasymand}\ \isanewline
\ \ \ \ \ \ \ \ \ \ Med\ x\ y\ {\isasymlongrightarrow}\ fnub{\isasymcdot}x\ {\isacharequal}\ fnub{\isasymcdot}y{\isachardoublequoteclose}\isanewline
\isadelimproof
\endisadelimproof
\isatagproof
\isacommand{apply}\isamarkupfalse%
\ {\isacharparenleft}induct{\isacharunderscore}tac\ k{\isacharcomma}\ auto{\isacharparenright}\isanewline
\isacommand{apply}\isamarkupfalse%
\ {\isacharparenleft}simp\ add{\isacharcolon}\ Fin{\isacharunderscore}{\isadigit{0}}{\isacharparenright}\isanewline
\isacommand{apply}\isamarkupfalse%
\ {\isacharparenleft}case{\isacharunderscore}tac\ {\isachardoublequoteopen}x\ {\isacharequal}\ {\isasymepsilon}{\isachardoublequoteclose}{\isacharcomma}\ auto{\isacharparenright}\isanewline
\isacommand{apply}\isamarkupfalse%
\ {\isacharparenleft}case{\isacharunderscore}tac\ {\isachardoublequoteopen}y\ {\isacharequal}\ {\isasymepsilon}{\isachardoublequoteclose}{\isacharcomma}\ auto{\isacharparenright}\isanewline
\isacommand{apply}\isamarkupfalse%
\ {\isacharparenleft}case{\isacharunderscore}tac\ {\isachardoublequoteopen}{\isacharhash}{\isacharparenleft}fftx{\isasymcdot}x{\isacharparenright}{\isachardoublequoteclose}{\isacharparenright}\isanewline
\isacommand{apply}\isamarkupfalse%
\ {\isacharparenleft}case{\isacharunderscore}tac\ {\isachardoublequoteopen}{\isacharhash}{\isacharparenleft}fftx{\isasymcdot}y{\isacharparenright}{\isachardoublequoteclose}{\isacharparenright}\isanewline
\isacommand{apply}\isamarkupfalse%
\ {\isacharparenleft}frule\ Med{\isacharunderscore}lemma{\isadigit{5}}{\isacharcomma}\ auto{\isacharparenright}\isanewline
\isacommand{apply}\isamarkupfalse%
\ {\isacharparenleft}drule\ sym{\isacharparenright}\isanewline
\isacommand{apply}\isamarkupfalse%
\ {\isacharparenleft}case{\isacharunderscore}tac\ {\isachardoublequoteopen}fft\ x\ {\isacharequal}\ fft\ y{\isachardoublequoteclose}{\isacharparenright}\isanewline
\isacommand{apply}\isamarkupfalse%
\ {\isacharparenleft}drule\ fslen{\isacharunderscore}fnub{\isacharunderscore}lemma{\isadigit{1}}{\isacharcomma}\ auto{\isacharparenright}\isanewline
\isacommand{apply}\isamarkupfalse%
\ {\isacharparenleft}drule\ fslen{\isacharunderscore}fnub{\isacharunderscore}lemma{\isadigit{2}}{\isacharcomma}\ auto{\isacharparenright}\isanewline
\isacommand{apply}\isamarkupfalse%
\ {\isacharparenleft}erule{\isacharunderscore}tac\ x{\isacharequal}{\isachardoublequoteopen}frtx{\isasymcdot}x{\isachardoublequoteclose}\ \isakeyword{in}\ allE{\isacharparenright}\isanewline
\isacommand{apply}\isamarkupfalse%
\ {\isacharparenleft}erule{\isacharunderscore}tac\ x{\isacharequal}{\isachardoublequoteopen}frtx{\isasymcdot}y{\isachardoublequoteclose}\ \isakeyword{in}\ allE{\isacharcomma}\ auto{\isacharparenright}\isanewline
\isacommand{apply}\isamarkupfalse%
\ {\isacharparenleft}case{\isacharunderscore}tac\ {\isachardoublequoteopen}fnub{\isasymcdot}x\ {\isacharequal}\ {\isasymepsilon}{\isachardoublequoteclose}{\isacharcomma}\ auto{\isacharparenright}\isanewline
\isacommand{apply}\isamarkupfalse%
\ {\isacharparenleft}drule\ strict{\isacharunderscore}rev{\isacharunderscore}fnub\ {\isacharbrackleft}rule{\isacharunderscore}format{\isacharbrackright}{\isacharcomma}\ simp{\isacharparenright}\isanewline
\isacommand{apply}\isamarkupfalse%
\ {\isacharparenleft}case{\isacharunderscore}tac\ {\isachardoublequoteopen}fnub{\isasymcdot}y\ {\isacharequal}\ {\isasymepsilon}{\isachardoublequoteclose}{\isacharcomma}\ auto{\isacharparenright}\isanewline
\isacommand{apply}\isamarkupfalse%
\ {\isacharparenleft}drule\ strict{\isacharunderscore}rev{\isacharunderscore}fnub\ {\isacharbrackleft}rule{\isacharunderscore}format{\isacharbrackright}{\isacharcomma}\ simp{\isacharparenright}\isanewline
\isacommand{apply}\isamarkupfalse%
\ {\isacharparenleft}drule\ fft{\isacharunderscore}fnub{\isacharunderscore}eq{\isacharunderscore}lemma{\isadigit{1}}{\isacharcomma}\ auto{\isacharparenright}\isanewline
\isacommand{apply}\isamarkupfalse%
\ {\isacharparenleft}subst\ exhaust{\isacharunderscore}to{\isacharunderscore}fft{\isacharunderscore}frt{\isacharcomma}\ auto{\isacharparenright}\isanewline
\isacommand{apply}\isamarkupfalse%
\ {\isacharparenleft}rule\ sym{\isacharparenright}\isanewline
\isacommand{apply}\isamarkupfalse%
\ {\isacharparenleft}subst\ exhaust{\isacharunderscore}to{\isacharunderscore}fft{\isacharunderscore}frt{\isacharcomma}\ auto{\isacharparenright}\isanewline
\isacommand{apply}\isamarkupfalse%
\ {\isacharparenleft}subgoal{\isacharunderscore}tac\ {\isachardoublequoteopen}Med\ {\isacharparenleft}frtx{\isasymcdot}x{\isacharparenright}\ y{\isachardoublequoteclose}{\isacharparenright}\isanewline
\isacommand{apply}\isamarkupfalse%
\ {\isacharparenleft}subgoal{\isacharunderscore}tac\ {\isachardoublequoteopen}{\isacharhash}{\isacharparenleft}fnub{\isasymcdot}y{\isacharparenright}\ {\isasymle}\ {\isacharhash}{\isacharparenleft}fnub{\isasymcdot}{\isacharparenleft}frtx{\isasymcdot}x{\isacharparenright}{\isacharparenright}{\isachardoublequoteclose}{\isacharparenright}\isanewline
\isacommand{apply}\isamarkupfalse%
\ {\isacharparenleft}drule\ fslen{\isacharunderscore}fnub{\isacharunderscore}Suc{\isacharunderscore}lemma{\isacharcomma}\ simp{\isacharparenright}\isanewline
\isacommand{apply}\isamarkupfalse%
\ {\isacharparenleft}drule\ fslen{\isacharunderscore}fnub{\isacharunderscore}Suc{\isacharunderscore}lemma{\isacharparenright}\isanewline
\isacommand{apply}\isamarkupfalse%
\ {\isacharparenleft}rule\ fnub{\isacharunderscore}less{\isacharunderscore}Med\ {\isacharbrackleft}rule{\isacharunderscore}format{\isacharbrackright}{\isacharcomma}\ auto{\isacharparenright}\isanewline
\isacommand{apply}\isamarkupfalse%
\ {\isacharparenleft}rule\ Med{\isacharunderscore}lemma{\isadigit{4}}\ {\isacharbrackleft}rule{\isacharunderscore}format{\isacharbrackright}{\isacharcomma}\ auto{\isacharparenright}\isanewline
\isacommand{apply}\isamarkupfalse%
\ {\isacharparenleft}frule\ fnub{\isacharunderscore}of{\isacharunderscore}fftx{\isacharcomma}\ auto{\isacharparenright}\isanewline
\isacommand{apply}\isamarkupfalse%
\ {\isacharparenleft}drule\ fnub{\isacharunderscore}eq{\isacharunderscore}Med{\isacharunderscore}lemma{\isadigit{1}}{\isacharcomma}\ auto{\isacharparenright}\isanewline
\isacommand{apply}\isamarkupfalse%
\ {\isacharparenleft}case{\isacharunderscore}tac\ {\isachardoublequoteopen}{\isacharhash}y{\isachardoublequoteclose}{\isacharcomma}\ auto{\isacharparenright}\isanewline
\isacommand{apply}\isamarkupfalse%
\ {\isacharparenleft}drule\ fslen{\isacharunderscore}fftx{\isacharunderscore}mono{\isacharparenright}{\isacharplus}\isanewline
\isacommand{apply}\isamarkupfalse%
\ auto\isanewline
\isacommand{by}\isamarkupfalse%
\ {\isacharparenleft}drule\ fftx{\isacharunderscore}inf{\isacharunderscore}Med{\isacharcomma}\ auto{\isacharparenright}%
\endisatagproof
{\isafoldproof}%
\isadelimproof
\isanewline
\endisadelimproof
\isanewline
\isacommand{lemma}\isamarkupfalse%
\ Med{\isacharunderscore}fdrop{\isacharunderscore}both{\isacharbrackleft}rule{\isacharunderscore}format{\isacharbrackright}{\isacharcolon}\ \isanewline
\ \ {\isachardoublequoteopen}Med\ x\ y\ {\isasymlongrightarrow}\ Med\ {\isacharparenleft}fdrop\ n{\isasymcdot}x{\isacharparenright}\ {\isacharparenleft}fdrop\ n{\isasymcdot}y{\isacharparenright}{\isachardoublequoteclose}\isanewline
\isadelimproof
\endisadelimproof
\isatagproof
\isacommand{apply}\isamarkupfalse%
\ {\isacharparenleft}induct{\isacharunderscore}tac\ n{\isacharcomma}\ auto{\isacharparenright}\isanewline
\isacommand{apply}\isamarkupfalse%
\ {\isacharparenleft}subst\ fdrop{\isacharunderscore}unfold{\isadigit{2}}{\isacharparenright}{\isacharplus}\isanewline
\isacommand{by}\isamarkupfalse%
\ {\isacharparenleft}rule\ Med{\isacharunderscore}frt{\isacharunderscore}both{\isacharparenright}%
\endisatagproof
{\isafoldproof}%
\isadelimproof
\isanewline
\endisadelimproof
\isanewline
\isacommand{lemma}\isamarkupfalse%
\ fslen{\isacharunderscore}inat{\isacharunderscore}simp{\isacharcolon}\ \isanewline
\ \ {\isachardoublequoteopen}{\isasymlbrakk}{\isacharhash}x\ {\isasymle}\ Fin\ {\isacharparenleft}Suc\ {\isacharparenleft}Suc\ {\isadigit{0}}{\isacharparenright}{\isacharparenright}{\isacharsemicolon}\ {\isacharhash}x\ {\isasymnoteq}\ Fin\ {\isacharparenleft}Suc\ {\isacharparenleft}Suc\ {\isadigit{0}}{\isacharparenright}{\isacharparenright}{\isacharsemicolon}\ x\ {\isasymnoteq}\ {\isasymepsilon}{\isasymrbrakk}\ \isanewline
\ \ \ \ {\isasymLongrightarrow}\ {\isacharhash}x\ {\isacharequal}\ Fin\ {\isacharparenleft}Suc\ {\isadigit{0}}{\isacharparenright}{\isachardoublequoteclose}\isanewline
\isadelimproof
\endisadelimproof
\isatagproof
\isacommand{apply}\isamarkupfalse%
\ {\isacharparenleft}drule\ fscase{\isadigit{2}}{\isacharcomma}\ auto{\isacharparenright}\isanewline
\isacommand{by}\isamarkupfalse%
\ {\isacharparenleft}auto\ simp\ add{\isacharcolon}\ inat{\isacharunderscore}defs\ split{\isacharcolon}\ inat{\isacharunderscore}splits{\isacharparenright}%
\endisatagproof
{\isafoldproof}%
\isadelimproof
\isanewline
\endisadelimproof
\isanewline
\isacommand{lemma}\isamarkupfalse%
\ ftake{\isacharunderscore}Suc{\isacharunderscore}fnub{\isacharunderscore}eq{\isacharunderscore}fnub{\isacharunderscore}lemma{\isacharcolon}\ \isanewline
\ \ {\isachardoublequoteopen}ftake\ {\isacharparenleft}Suc\ n{\isacharparenright}{\isasymcdot}{\isacharparenleft}fnub{\isasymcdot}x{\isacharparenright}\ {\isacharequal}\ fnub{\isasymcdot}y\ {\isasymLongrightarrow}\ ftake\ n{\isasymcdot}{\isacharparenleft}frt{\isasymcdot}{\isacharparenleft}fnub{\isasymcdot}x{\isacharparenright}{\isacharparenright}\ {\isacharequal}\ frt{\isasymcdot}{\isacharparenleft}fnub{\isasymcdot}y{\isacharparenright}{\isachardoublequoteclose}\isanewline
\isadelimproof
\endisadelimproof
\isatagproof
\isacommand{apply}\isamarkupfalse%
\ {\isacharparenleft}case{\isacharunderscore}tac\ {\isachardoublequoteopen}fnub{\isasymcdot}x\ {\isacharequal}\ {\isasymepsilon}{\isachardoublequoteclose}{\isacharcomma}\ auto{\isacharparenright}\isanewline
\isacommand{apply}\isamarkupfalse%
\ {\isacharparenleft}drule\ fscase{\isadigit{2}}{\isacharcomma}\ auto{\isacharparenright}\isanewline
\isacommand{apply}\isamarkupfalse%
\ {\isacharparenleft}case{\isacharunderscore}tac\ {\isachardoublequoteopen}fnub{\isasymcdot}y\ {\isacharequal}\ {\isasymepsilon}{\isachardoublequoteclose}{\isacharcomma}\ auto{\isacharparenright}\isanewline
\isacommand{apply}\isamarkupfalse%
\ {\isacharparenleft}drule\ fscase{\isadigit{2}}{\isacharcomma}\ auto{\isacharparenright}\isanewline
\isacommand{by}\isamarkupfalse%
\ {\isacharparenleft}drule\ fscons{\isadigit{2}}{\isacharunderscore}injects{\isacharcomma}\ simp{\isacharparenright}%
\endisatagproof
{\isafoldproof}%
\isadelimproof
\endisadelimproof
\begin{isamarkuptext}%
We also prove the following lemma, that we later use together with the properties of $Sender$, 
to prove the correctness of the protocol at the end of this chapter (Section~\ref{ABP_sys}).%
\end{isamarkuptext}%
\isamarkuptrue%
\isacommand{lemma}\isamarkupfalse%
\ Med{\isacharunderscore}trans{\isacharunderscore}lemma{\isacharcolon}\ \isanewline
\ \ {\isachardoublequoteopen}{\isasymforall}x\ y{\isachardot}\ \isanewline
\ \ \ \ \ \ Med\ x\ y\ {\isasymand}\ {\isacharhash}x\ {\isacharequal}\ {\isasyminfinity}\ {\isasymand}\ \isanewline
\ \ \ \ \ \ ftake\ k{\isasymcdot}{\isacharparenleft}fnub{\isasymcdot}x{\isacharparenright}\ {\isacharequal}\ fnub{\isasymcdot}y\ {\isasymand}\ \isanewline
\ \ \ \ \ \ {\isacharhash}{\isacharparenleft}fnub{\isasymcdot}y{\isacharparenright}\ {\isacharequal}\ Fin\ k\ {\isasymand}\ {\isacharhash}{\isacharparenleft}fnub{\isasymcdot}x{\isacharparenright}\ {\isasymle}\ Fin\ {\isacharparenleft}Suc\ k{\isacharparenright}\ \isanewline
\ \ \ \ \ \ {\isasymlongrightarrow}\ {\isacharhash}{\isacharparenleft}fnub{\isasymcdot}x{\isacharparenright}\ {\isacharequal}\ {\isacharhash}{\isacharparenleft}fnub{\isasymcdot}y{\isacharparenright}{\isachardoublequoteclose}\ \isanewline
\isadelimproof
\endisadelimproof
\isatagproof
\isacommand{apply}\isamarkupfalse%
\ {\isacharparenleft}induct{\isacharunderscore}tac\ k{\isacharcomma}\ auto{\isacharparenright}\isanewline
\isacommand{apply}\isamarkupfalse%
\ {\isacharparenleft}drule\ fair{\isacharunderscore}Med{\isacharcomma}\ auto{\isacharparenright}\isanewline
\isacommand{apply}\isamarkupfalse%
\ {\isacharparenleft}drule\ sym{\isacharparenright}\isanewline
\isacommand{apply}\isamarkupfalse%
\ {\isacharparenleft}drule\ strict{\isacharunderscore}rev{\isacharunderscore}fnub\ {\isacharbrackleft}rule{\isacharunderscore}format{\isacharbrackright}{\isacharcomma}\ simp{\isacharparenright}\isanewline
\isacommand{apply}\isamarkupfalse%
\ {\isacharparenleft}case{\isacharunderscore}tac\ {\isachardoublequoteopen}{\isacharhash}{\isacharparenleft}fftx{\isasymcdot}y{\isacharparenright}{\isachardoublequoteclose}{\isacharparenright}\isanewline
\isacommand{apply}\isamarkupfalse%
\ {\isacharparenleft}drule\ Med{\isacharunderscore}burst{\isacharunderscore}lemma{\isacharcomma}\ auto{\isacharparenright}\isanewline
\isacommand{apply}\isamarkupfalse%
\ {\isacharparenleft}drule\ ftake{\isacharunderscore}Suc{\isacharunderscore}fnub{\isacharunderscore}eq{\isacharunderscore}fnub{\isacharunderscore}lemma{\isacharparenright}\isanewline
\isacommand{apply}\isamarkupfalse%
\ {\isacharparenleft}erule{\isacharunderscore}tac\ x{\isacharequal}{\isachardoublequoteopen}frtx{\isasymcdot}x{\isachardoublequoteclose}\ \isakeyword{in}\ allE{\isacharcomma}\ auto{\isacharparenright}\isanewline
\isacommand{apply}\isamarkupfalse%
\ {\isacharparenleft}erule{\isacharunderscore}tac\ x{\isacharequal}{\isachardoublequoteopen}frtx{\isasymcdot}y{\isachardoublequoteclose}\ \isakeyword{in}\ allE{\isacharcomma}\ auto{\isacharparenright}\isanewline
\isacommand{apply}\isamarkupfalse%
\ {\isacharparenleft}simp\ add{\isacharcolon}\ fslen{\isacharunderscore}Suc{\isacharunderscore}Suc{\isacharunderscore}{\isadigit{2}}{\isacharunderscore}frt{\isacharparenright}\isanewline
\isacommand{apply}\isamarkupfalse%
\ {\isacharparenleft}case{\isacharunderscore}tac\ {\isachardoublequoteopen}{\isacharhash}{\isacharparenleft}fftx{\isasymcdot}x{\isacharparenright}{\isachardoublequoteclose}{\isacharparenright}\isanewline
\isacommand{apply}\isamarkupfalse%
\ {\isacharparenleft}drule\ fslen{\isacharunderscore}frtx{\isacharunderscore}inf{\isacharunderscore}lemma{\isacharcomma}\ auto{\isacharparenright}\isanewline
\isacommand{apply}\isamarkupfalse%
\ {\isacharparenleft}drule\ fftx{\isacharunderscore}inf{\isacharparenright}\isanewline
\isacommand{apply}\isamarkupfalse%
\ {\isacharparenleft}drule\ fslen{\isacharunderscore}fnub{\isacharunderscore}one{\isacharcomma}\ auto{\isacharparenright}\isanewline
\isacommand{apply}\isamarkupfalse%
\ {\isacharparenleft}drule\ fnub{\isacharunderscore}less{\isacharunderscore}Med{\isacharcomma}\ auto{\isacharparenright}\isanewline
\isacommand{apply}\isamarkupfalse%
\ {\isacharparenleft}simp\ add{\isacharcolon}\ fslen{\isacharunderscore}Suc{\isacharunderscore}Suc{\isacharunderscore}{\isadigit{2}}{\isacharunderscore}frt{\isacharunderscore}less{\isacharparenright}\isanewline
\isacommand{apply}\isamarkupfalse%
\ {\isacharparenleft}rule\ fslen{\isacharunderscore}Suc{\isacharunderscore}Suc{\isacharunderscore}{\isadigit{2}}{\isacharunderscore}frt{\isacharunderscore}rev{\isacharcomma}\ auto{\isacharparenright}\isanewline
\isacommand{apply}\isamarkupfalse%
\ {\isacharparenleft}drule\ strict{\isacharunderscore}rev{\isacharunderscore}fnub\ {\isacharbrackleft}rule{\isacharunderscore}format{\isacharbrackright}{\isacharcomma}\ simp{\isacharparenright}\isanewline
\isacommand{apply}\isamarkupfalse%
\ {\isacharparenleft}drule\ fftx{\isacharunderscore}inf{\isacharparenright}\isanewline
\isacommand{apply}\isamarkupfalse%
\ {\isacharparenleft}frule\ fair{\isacharunderscore}Med{\isacharcomma}\ auto{\isacharparenright}\isanewline
\isacommand{apply}\isamarkupfalse%
\ {\isacharparenleft}simp\ add{\isacharcolon}\ fslen{\isacharunderscore}fnub{\isacharunderscore}one{\isacharparenright}\isanewline
\isacommand{apply}\isamarkupfalse%
\ {\isacharparenleft}case{\isacharunderscore}tac\ {\isachardoublequoteopen}{\isacharhash}{\isacharparenleft}fnub{\isasymcdot}x{\isacharparenright}\ {\isacharequal}\ Fin\ {\isacharparenleft}Suc\ {\isacharparenleft}Suc\ {\isadigit{0}}{\isacharparenright}{\isacharparenright}{\isachardoublequoteclose}{\isacharparenright}\isanewline
\isacommand{apply}\isamarkupfalse%
\ {\isacharparenleft}frule\ fslen{\isacharunderscore}fnub{\isacharunderscore}two{\isacharunderscore}fftx{\isacharunderscore}fin{\isacharcomma}\ auto{\isacharparenright}\isanewline
\isacommand{apply}\isamarkupfalse%
\ {\isacharparenleft}subgoal{\isacharunderscore}tac\ {\isachardoublequoteopen}Med\ {\isacharparenleft}frtx{\isasymcdot}x{\isacharparenright}\ y{\isachardoublequoteclose}{\isacharparenright}\isanewline
\isacommand{apply}\isamarkupfalse%
\ {\isacharparenleft}frule\ fslen{\isacharunderscore}fnub{\isacharunderscore}two{\isacharunderscore}fftx{\isacharunderscore}frtx{\isacharunderscore}inf{\isacharcomma}\ auto{\isacharparenright}\isanewline
\isacommand{apply}\isamarkupfalse%
\ {\isacharparenleft}subgoal{\isacharunderscore}tac\ {\isachardoublequoteopen}frtx{\isasymcdot}x\ {\isacharequal}\ y{\isachardoublequoteclose}{\isacharcomma}\ auto{\isacharparenright}\isanewline
\isacommand{apply}\isamarkupfalse%
\ {\isacharparenleft}case{\isacharunderscore}tac\ {\isachardoublequoteopen}fnub{\isasymcdot}x{\isacharequal}{\isasymepsilon}{\isachardoublequoteclose}{\isacharcomma}\ auto{\isacharparenright}\isanewline
\isacommand{apply}\isamarkupfalse%
\ {\isacharparenleft}drule\ strict{\isacharunderscore}rev{\isacharunderscore}fnub\ {\isacharbrackleft}rule{\isacharunderscore}format{\isacharbrackright}{\isacharcomma}\ auto{\isacharparenright}\isanewline
\isacommand{apply}\isamarkupfalse%
\ {\isacharparenleft}simp\ add{\isacharcolon}\ fft{\isacharunderscore}ftake{\isadigit{2}}{\isacharparenright}\isanewline
\isacommand{apply}\isamarkupfalse%
\ {\isacharparenleft}drule\ fscase{\isadigit{2}}{\isacharcomma}\ auto{\isacharparenright}\isanewline
\isacommand{apply}\isamarkupfalse%
\ {\isacharparenleft}rule\ fftx{\isacharunderscore}inf{\isacharunderscore}Med{\isacharcomma}\ auto{\isacharparenright}\isanewline
\isacommand{apply}\isamarkupfalse%
\ {\isacharparenleft}simp\ add{\isacharcolon}\ frtx{\isadigit{2}}fdrop{\isacharparenright}\isanewline
\isacommand{apply}\isamarkupfalse%
\ {\isacharparenleft}subgoal{\isacharunderscore}tac\ {\isachardoublequoteopen}Med\ {\isacharparenleft}fdrop\ k{\isasymcdot}x{\isacharparenright}\ {\isacharparenleft}fdrop\ k{\isasymcdot}y{\isacharparenright}{\isachardoublequoteclose}{\isacharparenright}\isanewline
\isacommand{apply}\isamarkupfalse%
\ {\isacharparenleft}simp\ add{\isacharcolon}\ fslen{\isacharunderscore}fftx{\isacharunderscore}inf{\isacharunderscore}fdrop{\isacharunderscore}eq{\isacharunderscore}lemma\ {\isacharbrackleft}rule{\isacharunderscore}format{\isacharbrackright}{\isacharparenright}\isanewline
\isacommand{apply}\isamarkupfalse%
\ {\isacharparenleft}rule\ Med{\isacharunderscore}fdrop{\isacharunderscore}both{\isacharcomma}\ assumption{\isacharparenright}\isanewline
\isacommand{apply}\isamarkupfalse%
\ {\isacharparenleft}rule\ fslen{\isacharunderscore}inat{\isacharunderscore}simp{\isacharcomma}\ auto{\isacharparenright}\isanewline
\isacommand{by}\isamarkupfalse%
\ {\isacharparenleft}drule\ strict{\isacharunderscore}rev{\isacharunderscore}fnub\ {\isacharbrackleft}rule{\isacharunderscore}format{\isacharbrackright}{\isacharcomma}\ simp{\isacharparenright}%
\endisatagproof
{\isafoldproof}%
\isadelimproof
\isanewline
\endisadelimproof
\isanewline
\isacommand{lemma}\isamarkupfalse%
\ {\isacharbrackleft}rule{\isacharunderscore}format{\isacharcomma}\ simp{\isacharbrackright}{\isacharcolon}\isanewline
\ \ {\isachardoublequoteopen}{\isasymforall}p{\isachardot}\ fproj{\isadigit{2}}{\isasymcdot}{\isacharparenleft}fproj{\isadigit{1}}{\isasymcdot}{\isacharparenleft}ffilter\ {\isacharbraceleft}a{\isachardot}\ {\isasymexists}aa\ b{\isachardot}\ a\ {\isacharequal}\ {\isacharparenleft}{\isacharparenleft}aa{\isacharcomma}\ b{\isacharparenright}{\isacharcomma}\ True{\isacharparenright}{\isacharbraceright}{\isasymcdot}{\isacharparenleft}fzip{\isasymcdot}x{\isasymcdot}p{\isacharparenright}{\isacharparenright}{\isacharparenright}\ {\isacharequal}\isanewline
\ \ \ \ \ \ \ fproj{\isadigit{1}}{\isasymcdot}{\isacharparenleft}ffilter\ {\isacharbraceleft}a{\isachardot}\ {\isasymexists}b{\isachardot}\ a\ {\isacharequal}\ {\isacharparenleft}b{\isacharcomma}\ True{\isacharparenright}{\isacharbraceright}{\isasymcdot}{\isacharparenleft}fzip{\isasymcdot}{\isacharparenleft}fproj{\isadigit{2}}{\isasymcdot}x{\isacharparenright}{\isasymcdot}p{\isacharparenright}{\isacharparenright}{\isachardoublequoteclose}\isanewline
\isadelimproof
\endisadelimproof
\isatagproof
\isacommand{apply}\isamarkupfalse%
\ {\isacharparenleft}rule\ fstream{\isacharunderscore}ind{\isadigit{1}}\ {\isacharbrackleft}of\ {\isacharunderscore}\ x{\isacharbrackright}{\isacharcomma}\ auto{\isacharparenright}\isanewline
\isacommand{apply}\isamarkupfalse%
\ {\isacharparenleft}case{\isacharunderscore}tac\ {\isachardoublequoteopen}p{\isacharequal}{\isasymepsilon}{\isachardoublequoteclose}{\isacharcomma}\ auto{\isacharparenright}\isanewline
\isacommand{apply}\isamarkupfalse%
\ {\isacharparenleft}drule\ fscase{\isadigit{2}}{\isacharcomma}\ auto{\isacharparenright}\isanewline
\isacommand{by}\isamarkupfalse%
\ {\isacharparenleft}case{\isacharunderscore}tac\ aa{\isacharcomma}\ auto{\isacharparenright}%
\endisatagproof
{\isafoldproof}%
\isadelimproof
\isanewline
\endisadelimproof
\isanewline
\isacommand{lemma}\isamarkupfalse%
\ proj{\isadigit{2}}{\isacharunderscore}Med{\isacharcolon}\ \isanewline
\ \ {\isachardoublequoteopen}Med\ x\ y\ {\isasymLongrightarrow}\ Med\ {\isacharparenleft}fproj{\isadigit{2}}{\isasymcdot}x{\isacharparenright}\ {\isacharparenleft}fproj{\isadigit{2}}{\isasymcdot}y{\isacharparenright}{\isachardoublequoteclose}\isanewline
\isadelimproof
\endisadelimproof
\isatagproof
\isacommand{by}\isamarkupfalse%
\ {\isacharparenleft}auto\ simp\ add{\isacharcolon}\ Med{\isacharunderscore}def{\isacharparenright}%
\endisatagproof
{\isafoldproof}%
\isadelimproof
\isanewline
\endisadelimproof
\isadelimtheory
\isanewline
\endisadelimtheory
\isatagtheory
\isacommand{end}\isamarkupfalse%
\endisatagtheory
{\isafoldtheory}%
\isadelimtheory
\isanewline
\endisadelimtheory
\isanewline
\isanewline
\isanewline
\isanewline
\isanewline
\isanewline
\isanewline
\isanewline
\isanewline
\isanewline
\isanewline
\isanewline
\isanewline
\end{isabellebody}%
%%% Local Variables:
%%% mode: latex
%%% TeX-master: "root"
%%% End:

%
\section{Receiver} \label{ABP_Receiver}
\begin{isabellebody}%
\isacommand{constdefs}\isamarkupfalse%
\isanewline
\ \ Rcv\ {\isacharcolon}{\isacharcolon}\ {\isachardoublequoteopen}{\isacharparenleft}Data\ {\isacharasterisk}\ Bit{\isacharparenright}\ fstream\ {\isasymRightarrow}\ Bit\ fstream\ {\isasymRightarrow}\ Data\ fstream\ {\isasymRightarrow}\ bool{\isachardoublequoteclose}\isanewline
\ \ Rcv{\isacharunderscore}def{\isacharcolon}\ \isanewline
\ \ \ \ {\isachardoublequoteopen}Rcv\ dr\ ar\ out\ {\isasymequiv}\ \isanewline
\ \ \ \ \ \ \ ar\ {\isacharequal}\ fproj{\isadigit{2}}{\isasymcdot}dr\ {\isasymand}\ \isanewline
\ \ \ \ \ \ \ out\ {\isacharequal}\ fproj{\isadigit{1}}{\isasymcdot}{\isacharparenleft}fnub{\isasymcdot}dr{\isacharparenright}{\isachardoublequoteclose}\isanewline
\end{isabellebody}%
%%% Local Variables:
%%% mode: latex
%%% TeX-master: "root"
%%% End:

%
\section{System} \label{ABP_sys}
\begin{isabellebody}%
\isadelimtheory
\endisadelimtheory
\isatagtheory
\isacommand{theory}\isamarkupfalse%
\ ABP\isanewline
\isakeyword{imports}\ Sender\ Medium\ Receiver\isanewline
\isakeyword{begin}%
\endisatagtheory
{\isafoldtheory}%
\isadelimtheory
\isanewline
\endisadelimtheory
\isanewline
\isacommand{lemma}\isamarkupfalse%
\ proj{\isadigit{2}}{\isacharunderscore}abp{\isacharcolon}\ \isanewline
\ \ {\isachardoublequoteopen}{\isasymlbrakk}Snd\ i\ as\ ds{\isacharsemicolon}\ Med\ ds\ dr{\isacharsemicolon}\ Med\ {\isacharparenleft}fproj{\isadigit{2}}{\isasymcdot}dr{\isacharparenright}\ as{\isasymrbrakk}\ {\isasymLongrightarrow}\ Med\ {\isacharparenleft}fproj{\isadigit{2}}{\isasymcdot}ds{\isacharparenright}\ {\isacharparenleft}fproj{\isadigit{2}}{\isasymcdot}dr{\isacharparenright}{\isachardoublequoteclose}\isanewline
\isadelimproof
\endisadelimproof
\isatagproof
\isacommand{by}\isamarkupfalse%
\ {\isacharparenleft}rule\ proj{\isadigit{2}}{\isacharunderscore}Med{\isacharparenright}%
\endisatagproof
{\isafoldproof}%
\isadelimproof
\isanewline
\endisadelimproof
\isanewline
\isacommand{lemma}\isamarkupfalse%
\ abp{\isacharunderscore}one{\isacharunderscore}Med{\isacharcolon}\ \isanewline
\ \ {\isachardoublequoteopen}{\isasymlbrakk}Snd\ i\ as\ ds{\isacharsemicolon}\ Med\ ds\ dr{\isacharsemicolon}\ Med\ {\isacharparenleft}fproj{\isadigit{2}}{\isasymcdot}dr{\isacharparenright}\ as{\isasymrbrakk}\ {\isasymLongrightarrow}\ Med\ {\isacharparenleft}fproj{\isadigit{2}}{\isasymcdot}ds{\isacharparenright}\ as{\isachardoublequoteclose}\isanewline
\isadelimproof
\endisadelimproof
\isatagproof
\isacommand{apply}\isamarkupfalse%
\ {\isacharparenleft}drule\ proj{\isadigit{2}}{\isacharunderscore}abp{\isacharcomma}\ auto{\isacharparenright}\isanewline
\isacommand{by}\isamarkupfalse%
\ {\isacharparenleft}rule\ trans{\isacharunderscore}Med{\isacharcomma}\ auto{\isacharparenright}%
\endisatagproof
{\isafoldproof}%
\isadelimproof
\isanewline
\endisadelimproof
\isanewline
\isacommand{lemma}\isamarkupfalse%
\ fslen{\isacharunderscore}fnub{\isacharunderscore}fproj{\isadigit{2}}{\isacharunderscore}less{\isacharcolon}\ \isanewline
\ \ {\isachardoublequoteopen}{\isacharhash}{\isacharparenleft}fnub{\isasymcdot}{\isacharparenleft}fproj{\isadigit{2}}{\isasymcdot}x{\isacharparenright}{\isacharparenright}\ {\isasymsqsubseteq}\ {\isacharhash}{\isacharparenleft}fnub{\isasymcdot}x{\isacharparenright}{\isachardoublequoteclose}\isanewline
\isadelimproof
\endisadelimproof
\isatagproof
\isacommand{apply}\isamarkupfalse%
\ {\isacharparenleft}rule\ fstream{\isacharunderscore}ind{\isadigit{1}}\ {\isacharbrackleft}of\ {\isacharunderscore}\ x{\isacharbrackright}{\isacharcomma}\ auto{\isacharparenright}\isanewline
\isacommand{apply}\isamarkupfalse%
\ {\isacharparenleft}case{\isacharunderscore}tac\ {\isachardoublequoteopen}s{\isacharequal}{\isasymepsilon}{\isachardoublequoteclose}{\isacharcomma}\ auto{\isacharparenright}\isanewline
\isacommand{apply}\isamarkupfalse%
\ {\isacharparenleft}drule\ fscase{\isadigit{2}}{\isacharcomma}\ auto{\isacharparenright}\isanewline
\isacommand{apply}\isamarkupfalse%
\ {\isacharparenleft}case{\isacharunderscore}tac\ {\isachardoublequoteopen}b{\isacharequal}ba{\isachardoublequoteclose}{\isacharcomma}\ auto{\isacharparenright}\isanewline
\isacommand{apply}\isamarkupfalse%
\ {\isacharparenleft}case{\isacharunderscore}tac\ {\isachardoublequoteopen}a{\isacharequal}aa{\isachardoublequoteclose}{\isacharcomma}\ auto{\isacharparenright}\isanewline
\isacommand{by}\isamarkupfalse%
\ {\isacharparenleft}auto\ simp\ add{\isacharcolon}\ inat{\isacharunderscore}ord\ inat{\isacharunderscore}defs\ split{\isacharcolon}\ inat{\isacharunderscore}splits{\isacharparenright}%
\endisatagproof
{\isafoldproof}%
\isadelimproof
\isanewline
\endisadelimproof
\isanewline
\isacommand{lemma}\isamarkupfalse%
\ fslen{\isacharunderscore}fnub{\isacharunderscore}fproj{\isadigit{2}}{\isacharunderscore}mono{\isacharcolon}\ \isanewline
\ \ {\isachardoublequoteopen}{\isacharhash}{\isacharparenleft}fnub{\isasymcdot}{\isacharparenleft}fproj{\isadigit{2}}{\isasymcdot}x{\isacharparenright}{\isacharparenright}\ {\isasymle}\ {\isacharhash}{\isacharparenleft}fnub{\isasymcdot}x{\isacharparenright}{\isachardoublequoteclose}\isanewline
\isadelimproof
\endisadelimproof
\isatagproof
\isacommand{by}\isamarkupfalse%
\ {\isacharparenleft}insert\ fslen{\isacharunderscore}fnub{\isacharunderscore}fproj{\isadigit{2}}{\isacharunderscore}less\ {\isacharbrackleft}of\ x{\isacharbrackright}{\isacharcomma}\ simp\ add{\isacharcolon}\ inat{\isacharunderscore}ord{\isacharparenright}%
\endisatagproof
{\isafoldproof}%
\isadelimproof
\isanewline
\endisadelimproof
\isanewline
\isacommand{lemma}\isamarkupfalse%
\ Snd{\isacharunderscore}fslen{\isacharunderscore}lemma{\isacharcolon}\ \isanewline
\ \ {\isachardoublequoteopen}{\isasymlbrakk}Snd\ i\ as\ ds{\isacharsemicolon}\ Med\ ds\ dr{\isacharsemicolon}\ Med\ {\isacharparenleft}fproj{\isadigit{2}}{\isasymcdot}dr{\isacharparenright}\ as{\isasymrbrakk}\ {\isasymLongrightarrow}\ {\isacharhash}{\isacharparenleft}fnub{\isasymcdot}as{\isacharparenright}\ {\isasymle}\ {\isacharhash}{\isacharparenleft}fnub{\isasymcdot}ds{\isacharparenright}{\isachardoublequoteclose}\isanewline
\isadelimproof
\endisadelimproof
\isatagproof
\isacommand{apply}\isamarkupfalse%
\ {\isacharparenleft}drule\ abp{\isacharunderscore}one{\isacharunderscore}Med{\isacharcomma}\ auto{\isacharparenright}\isanewline
\isacommand{apply}\isamarkupfalse%
\ {\isacharparenleft}drule\ fnub{\isacharunderscore}less{\isacharunderscore}Med{\isacharparenright}{\isacharplus}\isanewline
\isacommand{apply}\isamarkupfalse%
\ {\isacharparenleft}insert\ fslen{\isacharunderscore}fnub{\isacharunderscore}fproj{\isadigit{2}}{\isacharunderscore}mono\ {\isacharbrackleft}of\ ds{\isacharbrackright}{\isacharparenright}\isanewline
\isacommand{by}\isamarkupfalse%
\ {\isacharparenleft}simp\ add{\isacharcolon}\ inat{\isacharunderscore}defs\ split{\isacharcolon}\ inat{\isacharunderscore}splits{\isacharparenright}%
\endisatagproof
{\isafoldproof}%
\isadelimproof
\isanewline
\endisadelimproof
\isanewline
\isacommand{lemma}\isamarkupfalse%
\ as{\isacharunderscore}less{\isacharunderscore}i{\isacharcolon}\isanewline
\ \ {\isachardoublequoteopen}{\isasymlbrakk}Snd\ i\ as\ ds{\isacharsemicolon}\ Med\ ds\ dr{\isacharsemicolon}\ Med\ {\isacharparenleft}fproj{\isadigit{2}}{\isasymcdot}dr{\isacharparenright}\ as{\isasymrbrakk}\ {\isasymLongrightarrow}\ {\isacharhash}{\isacharparenleft}fnub{\isasymcdot}as{\isacharparenright}\ {\isasymle}\ {\isacharhash}i{\isachardoublequoteclose}\isanewline
\isadelimproof
\endisadelimproof
\isatagproof
\isacommand{apply}\isamarkupfalse%
\ {\isacharparenleft}subgoal{\isacharunderscore}tac\ {\isachardoublequoteopen}{\isacharhash}{\isacharparenleft}fnub{\isasymcdot}ds{\isacharparenright}\ {\isasymle}\ {\isacharhash}i{\isachardoublequoteclose}{\isacharparenright}\ \isanewline
\isacommand{apply}\isamarkupfalse%
\ {\isacharparenleft}drule\ Snd{\isacharunderscore}fslen{\isacharunderscore}lemma{\isacharcomma}\ auto{\isacharparenright}\isanewline
\isacommand{apply}\isamarkupfalse%
\ {\isacharparenleft}simp\ add{\isacharcolon}\ inat{\isacharunderscore}defs\ split{\isacharcolon}\ inat{\isacharunderscore}splits{\isacharparenright}\isanewline
\isacommand{apply}\isamarkupfalse%
\ {\isacharparenleft}subgoal{\isacharunderscore}tac\ {\isachardoublequoteopen}fproj{\isadigit{1}}{\isasymcdot}{\isacharparenleft}fnub{\isasymcdot}ds{\isacharparenright}\ {\isasymsqsubseteq}\ i{\isachardoublequoteclose}{\isacharparenright}\isanewline
\isacommand{apply}\isamarkupfalse%
\ {\isacharparenleft}drule\ fslen{\isacharunderscore}mono{\isacharparenright}\isanewline
\isacommand{by}\isamarkupfalse%
\ {\isacharparenleft}auto\ simp\ add{\isacharcolon}\ fproj{\isadigit{1}}{\isacharunderscore}fslen\ Snd{\isacharunderscore}def\ Let{\isacharunderscore}def{\isacharparenright}%
\endisatagproof
{\isafoldproof}%
\isadelimproof
\isanewline
\endisadelimproof
\isanewline
\isacommand{lemma}\isamarkupfalse%
\ ABP{\isacharunderscore}fslen{\isacharunderscore}lemma{\isadigit{1}}{\isacharcolon}\ \isanewline
\ \ {\isachardoublequoteopen}{\isasymlbrakk}Snd\ i\ as\ ds{\isacharsemicolon}\ Med\ ds\ dr{\isacharsemicolon}\ Med\ {\isacharparenleft}fproj{\isadigit{2}}{\isasymcdot}dr{\isacharparenright}\ as{\isasymrbrakk}\ {\isasymLongrightarrow}\ {\isacharhash}{\isacharparenleft}fnub{\isasymcdot}ds{\isacharparenright}\ {\isacharequal}\ {\isacharhash}{\isacharparenleft}fnub{\isasymcdot}as{\isacharparenright}{\isachardoublequoteclose}\isanewline
\isadelimproof
\endisadelimproof
\isatagproof
\isacommand{apply}\isamarkupfalse%
\ {\isacharparenleft}case{\isacharunderscore}tac\ {\isachardoublequoteopen}{\isacharhash}{\isacharparenleft}fnub{\isasymcdot}as{\isacharparenright}\ {\isacharless}\ {\isacharhash}i{\isachardoublequoteclose}{\isacharparenright}\isanewline
\isacommand{apply}\isamarkupfalse%
\ {\isacharparenleft}case{\isacharunderscore}tac\ {\isachardoublequoteopen}fnub{\isasymcdot}as\ {\isacharequal}\ {\isasymepsilon}{\isachardoublequoteclose}{\isacharcomma}\ auto{\isacharparenright}\isanewline
\isacommand{apply}\isamarkupfalse%
\ {\isacharparenleft}drule\ strict{\isacharunderscore}rev{\isacharunderscore}fnub\ {\isacharbrackleft}rule{\isacharunderscore}format{\isacharbrackright}{\isacharparenright}\isanewline
\isacommand{apply}\isamarkupfalse%
\ {\isacharparenleft}simp\ add{\isacharcolon}\ Snd{\isacharunderscore}def\ Let{\isacharunderscore}def{\isacharcomma}\ auto{\isacharparenright}\isanewline
\isacommand{apply}\isamarkupfalse%
\ {\isacharparenleft}simp\ add{\isacharcolon}\ inat{\isacharunderscore}defs\ split{\isacharcolon}\ inat{\isacharunderscore}splits{\isacharparenright}\isanewline
\isacommand{apply}\isamarkupfalse%
\ {\isacharparenleft}drule\ fair{\isacharunderscore}Med{\isacharcomma}\ auto{\isacharparenright}\isanewline
\isacommand{apply}\isamarkupfalse%
\ {\isacharparenleft}simp\ add{\isacharcolon}\ fproj{\isadigit{2}}{\isacharunderscore}fslen\ {\isacharbrackleft}THEN\ sym{\isacharbrackright}{\isacharparenright}\isanewline
\isacommand{apply}\isamarkupfalse%
\ {\isacharparenleft}drule\ fair{\isacharunderscore}Med{\isacharcomma}\ auto{\isacharparenright}\isanewline
\isacommand{apply}\isamarkupfalse%
\ {\isacharparenleft}case{\isacharunderscore}tac\ {\isachardoublequoteopen}{\isacharhash}{\isacharparenleft}fnub{\isasymcdot}as{\isacharparenright}{\isachardoublequoteclose}{\isacharcomma}\ auto{\isacharparenright}\isanewline
\isacommand{apply}\isamarkupfalse%
\ {\isacharparenleft}case{\isacharunderscore}tac\ {\isachardoublequoteopen}nat{\isachardoublequoteclose}{\isacharcomma}\ auto{\isacharparenright}\isanewline
\isacommand{apply}\isamarkupfalse%
\ {\isacharparenleft}simp\ add{\isacharcolon}\ Fin{\isacharunderscore}{\isadigit{0}}{\isacharparenright}\isanewline
\isacommand{apply}\isamarkupfalse%
\ {\isacharparenleft}subgoal{\isacharunderscore}tac\ {\isachardoublequoteopen}{\isacharhash}ds\ {\isacharequal}\ {\isasyminfinity}{\isachardoublequoteclose}{\isacharparenright}\isanewline
\isacommand{apply}\isamarkupfalse%
\ {\isacharparenleft}frule\ abp{\isacharunderscore}one{\isacharunderscore}Med{\isacharcomma}\ auto{\isacharparenright}\isanewline
\isacommand{apply}\isamarkupfalse%
\ {\isacharparenleft}simp\ add{\isacharcolon}\ fproj{\isadigit{2}}{\isacharunderscore}fslen\ {\isacharbrackleft}THEN\ sym{\isacharbrackright}{\isacharparenright}\isanewline
\isacommand{apply}\isamarkupfalse%
\ {\isacharparenleft}subgoal{\isacharunderscore}tac\ {\isachardoublequoteopen}ftake\ {\isacharparenleft}Suc\ nata{\isacharparenright}{\isasymcdot}{\isacharparenleft}fnub{\isasymcdot}{\isacharparenleft}fproj{\isadigit{2}}{\isasymcdot}ds{\isacharparenright}{\isacharparenright}\ {\isacharequal}\ fnub{\isasymcdot}as{\isachardoublequoteclose}{\isacharparenright}\isanewline
\isacommand{apply}\isamarkupfalse%
\ {\isacharparenleft}simp\ add{\isacharcolon}\ alt{\isacharunderscore}Snd{\isacharunderscore}lemma{\isacharparenright}\isanewline
\isacommand{apply}\isamarkupfalse%
\ {\isacharparenleft}subgoal{\isacharunderscore}tac\ {\isachardoublequoteopen}{\isacharhash}{\isacharparenleft}fnub{\isasymcdot}{\isacharparenleft}fproj{\isadigit{2}}{\isasymcdot}ds{\isacharparenright}{\isacharparenright}\ {\isasymle}\ Fin\ {\isacharparenleft}Suc\ {\isacharparenleft}Suc\ nata{\isacharparenright}{\isacharparenright}{\isachardoublequoteclose}{\isacharparenright}\isanewline
\isacommand{apply}\isamarkupfalse%
\ {\isacharparenleft}subgoal{\isacharunderscore}tac\ {\isachardoublequoteopen}{\isacharhash}fnub{\isasymcdot}{\isacharparenleft}fproj{\isadigit{2}}{\isasymcdot}ds{\isacharparenright}\ {\isacharequal}\ {\isacharhash}{\isacharparenleft}fnub{\isasymcdot}as{\isacharparenright}{\isachardoublequoteclose}{\isacharcomma}\ simp{\isacharparenright}\isanewline
\isacommand{apply}\isamarkupfalse%
\ {\isacharparenleft}rule\ Med{\isacharunderscore}trans{\isacharunderscore}lemma\ \isanewline
\ \ \ \ \ \ \ \ \ {\isacharbrackleft}rule{\isacharunderscore}format{\isacharcomma}\ of\ {\isachardoublequoteopen}fproj{\isadigit{2}}{\isasymcdot}ds{\isachardoublequoteclose}\ {\isachardoublequoteopen}as{\isachardoublequoteclose}{\isacharbrackright}{\isacharcomma}\ auto{\isacharparenright}\ \isacommand{defer}\isamarkupfalse%
\ {\isadigit{1}}\isanewline
\isacommand{apply}\isamarkupfalse%
\ {\isacharparenleft}simp\ add{\isacharcolon}\ Snd{\isacharunderscore}def\ Let{\isacharunderscore}def{\isacharparenright}\isanewline
\isacommand{apply}\isamarkupfalse%
\ {\isacharparenleft}simp\ add{\isacharcolon}\ Snd{\isacharunderscore}def\ Let{\isacharunderscore}def{\isacharparenright}\ \isanewline
\isacommand{apply}\isamarkupfalse%
\ {\isacharparenleft}frule\ ack{\isacharunderscore}Snd{\isacharunderscore}lemma{\isacharcomma}\ auto{\isacharparenright}\isanewline
\isacommand{apply}\isamarkupfalse%
\ {\isacharparenleft}drule\ Snd{\isacharunderscore}fslen{\isacharunderscore}lemma{\isacharcomma}\ auto{\isacharparenright}\ \isanewline
\isacommand{apply}\isamarkupfalse%
\ {\isacharparenleft}simp\ add{\isacharcolon}\ inat{\isacharunderscore}defs\ split{\isacharcolon}\ inat{\isacharunderscore}splits{\isacharparenright}\ \isacommand{defer}\isamarkupfalse%
\ {\isadigit{1}}\isanewline
\isacommand{apply}\isamarkupfalse%
\ {\isacharparenleft}simp\ add{\isacharcolon}\ Snd{\isacharunderscore}def\ Let{\isacharunderscore}def{\isacharparenright}\isanewline
\isacommand{apply}\isamarkupfalse%
\ {\isacharparenleft}simp\ add{\isacharcolon}\ fproj{\isadigit{1}}{\isacharunderscore}fslen\ fproj{\isadigit{2}}{\isacharunderscore}fslen{\isacharparenright}\isanewline
\isacommand{apply}\isamarkupfalse%
\ {\isacharparenleft}simp\ add{\isacharcolon}\ inat{\isacharunderscore}defs\ split{\isacharcolon}\ inat{\isacharunderscore}splits{\isacharcomma}\ arith{\isacharquery}{\isacharparenright}\isanewline
\isacommand{apply}\isamarkupfalse%
\ {\isacharparenleft}frule\ as{\isacharunderscore}less{\isacharunderscore}i{\isacharcomma}\ auto{\isacharparenright}\isanewline
\isacommand{apply}\isamarkupfalse%
\ {\isacharparenleft}simp\ add{\isacharcolon}\ inat{\isacharunderscore}defs\ split{\isacharcolon}\ inat{\isacharunderscore}splits{\isacharparenright}\isanewline
\isacommand{apply}\isamarkupfalse%
\ {\isacharparenleft}simp\ add{\isacharcolon}\ Snd{\isacharunderscore}def\ Let{\isacharunderscore}def{\isacharcomma}\ auto{\isacharparenright}\isanewline
\isacommand{apply}\isamarkupfalse%
\ {\isacharparenleft}simp\ add{\isacharcolon}\ fproj{\isadigit{1}}{\isacharunderscore}fslen{\isacharcomma}\ arith{\isacharparenright}\isanewline
\isacommand{apply}\isamarkupfalse%
\ {\isacharparenleft}drule\ Snd{\isacharunderscore}fslen{\isacharunderscore}lemma{\isacharcomma}\ auto{\isacharparenright}\isanewline
\isacommand{by}\isamarkupfalse%
\ {\isacharparenleft}simp\ add{\isacharcolon}\ inat{\isacharunderscore}defs\ split{\isacharcolon}\ inat{\isacharunderscore}splits{\isacharparenright}%
\endisatagproof
{\isafoldproof}%
\isadelimproof
\isanewline
\endisadelimproof
\isanewline
\isacommand{lemma}\isamarkupfalse%
\ Snd{\isacharunderscore}inat{\isacharunderscore}lemma{\isadigit{1}}{\isacharcolon}\ \isanewline
\ \ {\isachardoublequoteopen}{\isacharhash}fnub{\isasymcdot}as\ {\isacharequal}\ imin\ {\isacharparenleft}Fin\ k{\isacharparenright}\ {\isacharparenleft}iSuc\ {\isacharhash}fnub{\isasymcdot}as{\isacharparenright}\ {\isasymLongrightarrow}\ {\isacharhash}{\isacharparenleft}fnub{\isasymcdot}as{\isacharparenright}\ {\isacharequal}\ Fin\ k{\isachardoublequoteclose}\isanewline
\isadelimproof
\endisadelimproof
\isatagproof
\isacommand{by}\isamarkupfalse%
\ {\isacharparenleft}auto\ simp\ add{\isacharcolon}\ imin{\isacharunderscore}def\ inat{\isacharunderscore}defs\ split{\isacharcolon}\ inat{\isacharunderscore}splits{\isacharcomma}\ arith{\isacharquery}{\isacharparenright}%
\endisatagproof
{\isafoldproof}%
\isadelimproof
\isanewline
\endisadelimproof
\isanewline
\isacommand{lemma}\isamarkupfalse%
\ Snd{\isacharunderscore}inat{\isacharunderscore}lemma{\isadigit{2}}{\isacharcolon}\isanewline
\ \ {\isachardoublequoteopen}Snd\ i\ as\ ds\ {\isasymLongrightarrow}\ {\isacharhash}{\isacharparenleft}fnub{\isasymcdot}ds{\isacharparenright}\ {\isacharequal}\ imin\ {\isacharhash}i\ {\isacharparenleft}iSuc\ {\isacharhash}{\isacharparenleft}fnub{\isasymcdot}as{\isacharparenright}{\isacharparenright}{\isachardoublequoteclose}\isanewline
\isadelimproof
\endisadelimproof
\isatagproof
\isacommand{by}\isamarkupfalse%
\ {\isacharparenleft}auto\ simp\ add{\isacharcolon}\ Snd{\isacharunderscore}def\ Let{\isacharunderscore}def\ fproj{\isadigit{1}}{\isacharunderscore}fslen{\isacharparenright}%
\endisatagproof
{\isafoldproof}%
\isadelimproof
\isanewline
\endisadelimproof
\isanewline
\isacommand{lemma}\isamarkupfalse%
\ ABP{\isacharunderscore}fslen{\isacharunderscore}lemma{\isadigit{3}}{\isacharcolon}\ \isanewline
\ \ {\isachardoublequoteopen}{\isasymlbrakk}Snd\ i\ as\ ds{\isacharsemicolon}\ Med\ ds\ dr{\isacharsemicolon}\ Med\ {\isacharparenleft}fproj{\isadigit{2}}{\isasymcdot}dr{\isacharparenright}\ as{\isasymrbrakk}\ {\isasymLongrightarrow}\ {\isacharhash}{\isacharparenleft}fnub{\isasymcdot}ds{\isacharparenright}\ {\isacharequal}\ {\isacharhash}i{\isachardoublequoteclose}\isanewline
\isadelimproof
\endisadelimproof
\isatagproof
\isacommand{apply}\isamarkupfalse%
\ {\isacharparenleft}frule\ ABP{\isacharunderscore}fslen{\isacharunderscore}lemma{\isadigit{1}}{\isacharcomma}\ assumption{\isacharplus}{\isacharparenright}\isanewline
\isacommand{apply}\isamarkupfalse%
\ {\isacharparenleft}drule\ Snd{\isacharunderscore}inat{\isacharunderscore}lemma{\isadigit{2}}{\isacharcomma}\ auto{\isacharparenright}\isanewline
\isacommand{by}\isamarkupfalse%
\ {\isacharparenleft}simp\ add{\isacharcolon}\ imin{\isacharunderscore}def\ inat{\isacharunderscore}defs\ split{\isacharcolon}\ inat{\isacharunderscore}splits{\isacharcomma}\ arith{\isacharquery}{\isacharparenright}%
\endisatagproof
{\isafoldproof}%
\isadelimproof
\isanewline
\endisadelimproof
\isanewline
\isacommand{lemma}\isamarkupfalse%
\ ABP{\isacharunderscore}fslen{\isacharunderscore}lemma{\isadigit{2}}{\isacharcolon}\ \isanewline
\ \ {\isachardoublequoteopen}{\isasymlbrakk}Snd\ i\ as\ ds{\isacharsemicolon}\ Med\ ds\ dr{\isacharsemicolon}\ Med\ {\isacharparenleft}fproj{\isadigit{2}}{\isasymcdot}dr{\isacharparenright}\ as{\isasymrbrakk}\ {\isasymLongrightarrow}\ {\isacharhash}{\isacharparenleft}fnub{\isasymcdot}ds{\isacharparenright}\ {\isacharequal}\ {\isacharhash}{\isacharparenleft}fnub{\isasymcdot}dr{\isacharparenright}{\isachardoublequoteclose}\isanewline
\isadelimproof
\endisadelimproof
\isatagproof
\isacommand{apply}\isamarkupfalse%
\ {\isacharparenleft}frule\ ABP{\isacharunderscore}fslen{\isacharunderscore}lemma{\isadigit{1}}{\isacharcomma}\ assumption{\isacharplus}{\isacharparenright}\isanewline
\isacommand{apply}\isamarkupfalse%
\ {\isacharparenleft}drule\ fnub{\isacharunderscore}less{\isacharunderscore}Med{\isacharparenright}{\isacharplus}\isanewline
\isacommand{apply}\isamarkupfalse%
\ {\isacharparenleft}insert\ fslen{\isacharunderscore}fnub{\isacharunderscore}fproj{\isadigit{2}}{\isacharunderscore}mono\ {\isacharbrackleft}of\ dr{\isacharbrackright}{\isacharparenright}\isanewline
\isacommand{by}\isamarkupfalse%
\ {\isacharparenleft}auto\ simp\ add{\isacharcolon}\ inat{\isacharunderscore}defs\ split{\isacharcolon}\ inat{\isacharunderscore}splits{\isacharparenright}%
\endisatagproof
{\isafoldproof}%
\isadelimproof
\isanewline
\endisadelimproof
\isanewline
\isacommand{lemma}\isamarkupfalse%
\ ABP{\isacharunderscore}fin{\isacharunderscore}correct{\isacharunderscore}lemma{\isacharcolon}\ \isanewline
\ \ {\isachardoublequoteopen}{\isasymlbrakk}Snd\ i\ as\ ds{\isacharsemicolon}\ Med\ ds\ dr{\isacharsemicolon}\ Rcv\ dr\ ar\ out{\isacharsemicolon}\ Med\ ar\ as{\isacharsemicolon}\ {\isacharhash}i\ {\isacharequal}\ Fin\ k{\isasymrbrakk}\ {\isasymLongrightarrow}\ out\ {\isacharequal}\ fproj{\isadigit{1}}{\isasymcdot}{\isacharparenleft}fnub{\isasymcdot}ds{\isacharparenright}{\isachardoublequoteclose}\isanewline
\isadelimproof
\endisadelimproof
\isatagproof
\isacommand{apply}\isamarkupfalse%
\ {\isacharparenleft}auto\ simp\ add{\isacharcolon}\ Rcv{\isacharunderscore}def{\isacharparenright}\isanewline
\isacommand{apply}\isamarkupfalse%
\ {\isacharparenleft}frule\ ABP{\isacharunderscore}fslen{\isacharunderscore}lemma{\isadigit{2}}{\isacharcomma}\ assumption{\isacharplus}{\isacharparenright}\isanewline
\isacommand{apply}\isamarkupfalse%
\ {\isacharparenleft}frule\ ABP{\isacharunderscore}fslen{\isacharunderscore}lemma{\isadigit{3}}{\isacharcomma}\ assumption{\isacharplus}{\isacharparenright}\isanewline
\isacommand{apply}\isamarkupfalse%
\ {\isacharparenleft}rule\ cfun{\isacharunderscore}arg{\isacharunderscore}cong{\isacharparenright}\isanewline
\isacommand{by}\isamarkupfalse%
\ {\isacharparenleft}insert\ fnub{\isacharunderscore}eq{\isacharunderscore}Med\ {\isacharbrackleft}rule{\isacharunderscore}format{\isacharcomma}\ of\ ds\ dr\ k{\isacharbrackright}{\isacharcomma}\ auto{\isacharparenright}%
\endisatagproof
{\isafoldproof}%
\isadelimproof
\isanewline
\endisadelimproof
\isanewline
\isacommand{lemma}\isamarkupfalse%
\ ABP{\isacharunderscore}fin{\isacharunderscore}correct{\isacharcolon}\ \isanewline
\ \ {\isachardoublequoteopen}{\isasymlbrakk}{\isacharhash}i\ {\isacharequal}\ Fin\ k{\isacharsemicolon}\ Snd\ i\ as\ ds{\isacharsemicolon}\ Med\ ds\ dr{\isacharsemicolon}\ Rcv\ dr\ ar\ out{\isacharsemicolon}\ Med\ ar\ as{\isasymrbrakk}\ {\isasymLongrightarrow}\ out\ {\isacharequal}\ i{\isachardoublequoteclose}\isanewline
\isadelimproof
\endisadelimproof
\isatagproof
\isacommand{apply}\isamarkupfalse%
\ {\isacharparenleft}frule\ ABP{\isacharunderscore}fin{\isacharunderscore}correct{\isacharunderscore}lemma{\isacharcomma}\ assumption{\isacharplus}{\isacharparenright}\isanewline
\isacommand{apply}\isamarkupfalse%
\ {\isacharparenleft}simp\ add{\isacharcolon}\ Rcv{\isacharunderscore}def{\isacharparenright}\isanewline
\isacommand{apply}\isamarkupfalse%
\ {\isacharparenleft}frule\ ABP{\isacharunderscore}fslen{\isacharunderscore}lemma{\isadigit{3}}{\isacharcomma}\ assumption{\isacharplus}{\isacharparenright}\isanewline
\isacommand{apply}\isamarkupfalse%
\ {\isacharparenleft}drule\ SndD{\isadigit{1}}{\isacharcomma}\ auto{\isacharparenright}\isanewline
\isacommand{apply}\isamarkupfalse%
\ {\isacharparenleft}rule\ size{\isacharunderscore}eq{\isacharcomma}\ auto{\isacharparenright}\isanewline
\isacommand{by}\isamarkupfalse%
\ {\isacharparenleft}simp\ add{\isacharcolon}\ fproj{\isadigit{1}}{\isacharunderscore}fslen\ {\isacharbrackleft}THEN\ sym{\isacharbrackright}{\isacharparenright}%
\endisatagproof
{\isafoldproof}%
\isadelimproof
\isanewline
\endisadelimproof
\isadelimtheory
\isanewline
\endisadelimtheory
\isatagtheory
\isacommand{end}\isamarkupfalse%
\endisatagtheory
{\isafoldtheory}%
\isadelimtheory
\isanewline
\endisadelimtheory
\isanewline
\isanewline
\isanewline
\end{isabellebody}%
%%% Local Variables:
%%% mode: latex
%%% TeX-master: "root"
%%% End:
