# Supplementary material for: ALICE: An Advanced Logic for Interactive Component Engineering
Source: arXiv:1410.4381 source file (2014-10-16)
Supplement: Supplementary file 2 [file ABPTypes.tex]

\begin{isabellebody}%
\isadelimtheory
\endisadelimtheory
\isatagtheory
\isacommand{theory}\isamarkupfalse%
\ ABPTypes\isanewline
\isakeyword{imports}\ ALICE\isanewline
\isakeyword{begin}%
\endisatagtheory
{\isafoldtheory}%
\isadelimtheory
\isanewline
\endisadelimtheory
\isanewline
\isacommand{typedecl}\isamarkupfalse%
\ Data\ %
\isamarkupcmt{a generic type for data%
}
\isanewline
\isacommand{types}\isamarkupfalse%
\ Bit\ {\isacharequal}\ bool%
\begin{isamarkuptext}%
By the latter type declaration in HOL, we take {\pisastyle{Bit}} as a type alias 
for the HOL type {\pisastyle{bool}}.%
\end{isamarkuptext}%
\isamarkuptrue%
\isadelimtheory
\endisadelimtheory
\isatagtheory
\isacommand{end}\isamarkupfalse%
\endisatagtheory
{\isafoldtheory}%
\isadelimtheory
\endisadelimtheory
\isanewline
\end{isabellebody}%
%%% Local Variables:
%%% mode: latex
%%% TeX-master: "root"
%%% End:
