# Supplementary material for: ALICE: An Advanced Logic for Interactive Component Engineering
Source: arXiv:1410.4381 source file (2014-10-16)
Supplement: Supplementary file 3 [file ABP.tex]

%
\begin{isabellebody}%
\def\isabellecontext{ABP}%
%
\isadelimtheory
%
\endisadelimtheory
%
\isatagtheory
\isacommand{theory}\isamarkupfalse%
\ ABP\isanewline
\isakeyword{imports}\ Sender\ Medium\ Receiver\isanewline
\isakeyword{begin}%
\endisatagtheory
{\isafoldtheory}%
%
\isadelimtheory
\isanewline
%
\endisadelimtheory
\isanewline
\isacommand{lemma}\isamarkupfalse%
\ proj{\isadigit{2}}{\isacharunderscore}abp{\isacharcolon}\ \isanewline
\ \ {\isachardoublequoteopen}{\isasymlbrakk}Snd\ i\ as\ ds{\isacharsemicolon}\ Med\ ds\ dr{\isacharsemicolon}\ Med\ {\isacharparenleft}fproj{\isadigit{2}}{\isasymcdot}dr{\isacharparenright}\ as{\isasymrbrakk}\ {\isasymLongrightarrow}\ Med\ {\isacharparenleft}fproj{\isadigit{2}}{\isasymcdot}ds{\isacharparenright}\ {\isacharparenleft}fproj{\isadigit{2}}{\isasymcdot}dr{\isacharparenright}{\isachardoublequoteclose}\isanewline
%
\isadelimproof
%
\endisadelimproof
%
\isatagproof
\isacommand{by}\isamarkupfalse%
\ {\isacharparenleft}rule\ proj{\isadigit{2}}{\isacharunderscore}Med{\isacharparenright}%
\endisatagproof
{\isafoldproof}%
%
\isadelimproof
\isanewline
%
\endisadelimproof
\isanewline
\isacommand{lemma}\isamarkupfalse%
\ abp{\isacharunderscore}one{\isacharunderscore}Med{\isacharcolon}\ \isanewline
\ \ {\isachardoublequoteopen}{\isasymlbrakk}Snd\ i\ as\ ds{\isacharsemicolon}\ Med\ ds\ dr{\isacharsemicolon}\ Med\ {\isacharparenleft}fproj{\isadigit{2}}{\isasymcdot}dr{\isacharparenright}\ as{\isasymrbrakk}\ {\isasymLongrightarrow}\ Med\ {\isacharparenleft}fproj{\isadigit{2}}{\isasymcdot}ds{\isacharparenright}\ as{\isachardoublequoteclose}\isanewline
%
\isadelimproof
%
\endisadelimproof
%
\isatagproof
\isacommand{apply}\isamarkupfalse%
\ {\isacharparenleft}drule\ proj{\isadigit{2}}{\isacharunderscore}abp{\isacharcomma}\ auto{\isacharparenright}\isanewline
\isacommand{by}\isamarkupfalse%
\ {\isacharparenleft}rule\ trans{\isacharunderscore}Med{\isacharcomma}\ auto{\isacharparenright}%
\endisatagproof
{\isafoldproof}%
%
\isadelimproof
\isanewline
%
\endisadelimproof
\isanewline
\isacommand{lemma}\isamarkupfalse%
\ fslen{\isacharunderscore}fnub{\isacharunderscore}fproj{\isadigit{2}}{\isacharunderscore}less{\isacharcolon}\ \isanewline
\ \ {\isachardoublequoteopen}{\isacharhash}{\isacharparenleft}fnub{\isasymcdot}{\isacharparenleft}fproj{\isadigit{2}}{\isasymcdot}x{\isacharparenright}{\isacharparenright}\ {\isasymsqsubseteq}\ {\isacharhash}{\isacharparenleft}fnub{\isasymcdot}x{\isacharparenright}{\isachardoublequoteclose}\isanewline
%
\isadelimproof
%
\endisadelimproof
%
\isatagproof
\isacommand{apply}\isamarkupfalse%
\ {\isacharparenleft}rule\ fstream{\isacharunderscore}ind{\isadigit{1}}\ {\isacharbrackleft}of\ {\isacharunderscore}\ x{\isacharbrackright}{\isacharcomma}\ auto{\isacharparenright}\isanewline
\isacommand{apply}\isamarkupfalse%
\ {\isacharparenleft}case{\isacharunderscore}tac\ {\isachardoublequoteopen}s{\isacharequal}{\isasymepsilon}{\isachardoublequoteclose}{\isacharcomma}\ auto{\isacharparenright}\isanewline
\isacommand{apply}\isamarkupfalse%
\ {\isacharparenleft}drule\ fscase{\isadigit{2}}{\isacharcomma}\ auto{\isacharparenright}\isanewline
\isacommand{apply}\isamarkupfalse%
\ {\isacharparenleft}case{\isacharunderscore}tac\ {\isachardoublequoteopen}b{\isacharequal}ba{\isachardoublequoteclose}{\isacharcomma}\ auto{\isacharparenright}\isanewline
\isacommand{apply}\isamarkupfalse%
\ {\isacharparenleft}case{\isacharunderscore}tac\ {\isachardoublequoteopen}a{\isacharequal}aa{\isachardoublequoteclose}{\isacharcomma}\ auto{\isacharparenright}\isanewline
\isacommand{by}\isamarkupfalse%
\ {\isacharparenleft}auto\ simp\ add{\isacharcolon}\ inat{\isacharunderscore}ord\ inat{\isacharunderscore}defs\ split{\isacharcolon}\ inat{\isacharunderscore}splits{\isacharparenright}%
\endisatagproof
{\isafoldproof}%
%
\isadelimproof
\isanewline
%
\endisadelimproof
\isanewline
\isacommand{lemma}\isamarkupfalse%
\ fslen{\isacharunderscore}fnub{\isacharunderscore}fproj{\isadigit{2}}{\isacharunderscore}mono{\isacharcolon}\ \isanewline
\ \ {\isachardoublequoteopen}{\isacharhash}{\isacharparenleft}fnub{\isasymcdot}{\isacharparenleft}fproj{\isadigit{2}}{\isasymcdot}x{\isacharparenright}{\isacharparenright}\ {\isasymle}\ {\isacharhash}{\isacharparenleft}fnub{\isasymcdot}x{\isacharparenright}{\isachardoublequoteclose}\isanewline
%
\isadelimproof
%
\endisadelimproof
%
\isatagproof
\isacommand{by}\isamarkupfalse%
\ {\isacharparenleft}insert\ fslen{\isacharunderscore}fnub{\isacharunderscore}fproj{\isadigit{2}}{\isacharunderscore}less\ {\isacharbrackleft}of\ x{\isacharbrackright}{\isacharcomma}\ simp\ add{\isacharcolon}\ inat{\isacharunderscore}ord{\isacharparenright}%
\endisatagproof
{\isafoldproof}%
%
\isadelimproof
\isanewline
%
\endisadelimproof
\isanewline
\isacommand{lemma}\isamarkupfalse%
\ Snd{\isacharunderscore}fslen{\isacharunderscore}lemma{\isacharcolon}\ \isanewline
\ \ {\isachardoublequoteopen}{\isasymlbrakk}Snd\ i\ as\ ds{\isacharsemicolon}\ Med\ ds\ dr{\isacharsemicolon}\ Med\ {\isacharparenleft}fproj{\isadigit{2}}{\isasymcdot}dr{\isacharparenright}\ as{\isasymrbrakk}\ {\isasymLongrightarrow}\ {\isacharhash}{\isacharparenleft}fnub{\isasymcdot}as{\isacharparenright}\ {\isasymle}\ {\isacharhash}{\isacharparenleft}fnub{\isasymcdot}ds{\isacharparenright}{\isachardoublequoteclose}\isanewline
%
\isadelimproof
%
\endisadelimproof
%
\isatagproof
\isacommand{apply}\isamarkupfalse%
\ {\isacharparenleft}drule\ abp{\isacharunderscore}one{\isacharunderscore}Med{\isacharcomma}\ auto{\isacharparenright}\isanewline
\isacommand{apply}\isamarkupfalse%
\ {\isacharparenleft}drule\ fnub{\isacharunderscore}less{\isacharunderscore}Med{\isacharparenright}{\isacharplus}\isanewline
\isacommand{apply}\isamarkupfalse%
\ {\isacharparenleft}insert\ fslen{\isacharunderscore}fnub{\isacharunderscore}fproj{\isadigit{2}}{\isacharunderscore}mono\ {\isacharbrackleft}of\ ds{\isacharbrackright}{\isacharparenright}\isanewline
\isacommand{by}\isamarkupfalse%
\ {\isacharparenleft}simp\ add{\isacharcolon}\ inat{\isacharunderscore}defs\ split{\isacharcolon}\ inat{\isacharunderscore}splits{\isacharparenright}%
\endisatagproof
{\isafoldproof}%
%
\isadelimproof
\isanewline
%
\endisadelimproof
\isanewline
\isacommand{lemma}\isamarkupfalse%
\ as{\isacharunderscore}less{\isacharunderscore}i{\isacharcolon}\isanewline
\ \ {\isachardoublequoteopen}{\isasymlbrakk}Snd\ i\ as\ ds{\isacharsemicolon}\ Med\ ds\ dr{\isacharsemicolon}\ Med\ {\isacharparenleft}fproj{\isadigit{2}}{\isasymcdot}dr{\isacharparenright}\ as{\isasymrbrakk}\ {\isasymLongrightarrow}\ {\isacharhash}{\isacharparenleft}fnub{\isasymcdot}as{\isacharparenright}\ {\isasymle}\ {\isacharhash}i{\isachardoublequoteclose}\isanewline
%
\isadelimproof
%
\endisadelimproof
%
\isatagproof
\isacommand{apply}\isamarkupfalse%
\ {\isacharparenleft}subgoal{\isacharunderscore}tac\ {\isachardoublequoteopen}{\isacharhash}{\isacharparenleft}fnub{\isasymcdot}ds{\isacharparenright}\ {\isasymle}\ {\isacharhash}i{\isachardoublequoteclose}{\isacharparenright}\ \isanewline
\isacommand{apply}\isamarkupfalse%
\ {\isacharparenleft}drule\ Snd{\isacharunderscore}fslen{\isacharunderscore}lemma{\isacharcomma}\ auto{\isacharparenright}\isanewline
\isacommand{apply}\isamarkupfalse%
\ {\isacharparenleft}simp\ add{\isacharcolon}\ inat{\isacharunderscore}defs\ split{\isacharcolon}\ inat{\isacharunderscore}splits{\isacharparenright}\isanewline
\isacommand{apply}\isamarkupfalse%
\ {\isacharparenleft}subgoal{\isacharunderscore}tac\ {\isachardoublequoteopen}fproj{\isadigit{1}}{\isasymcdot}{\isacharparenleft}fnub{\isasymcdot}ds{\isacharparenright}\ {\isasymsqsubseteq}\ i{\isachardoublequoteclose}{\isacharparenright}\isanewline
\isacommand{apply}\isamarkupfalse%
\ {\isacharparenleft}drule\ fslen{\isacharunderscore}mono{\isacharparenright}\isanewline
\isacommand{by}\isamarkupfalse%
\ {\isacharparenleft}auto\ simp\ add{\isacharcolon}\ fproj{\isadigit{1}}{\isacharunderscore}fslen\ Snd{\isacharunderscore}def\ Let{\isacharunderscore}def{\isacharparenright}%
\endisatagproof
{\isafoldproof}%
%
\isadelimproof
\isanewline
%
\endisadelimproof
\isanewline
\isacommand{lemma}\isamarkupfalse%
\ ABP{\isacharunderscore}fslen{\isacharunderscore}lemma{\isadigit{1}}{\isacharcolon}\ \isanewline
\ \ {\isachardoublequoteopen}{\isasymlbrakk}Snd\ i\ as\ ds{\isacharsemicolon}\ Med\ ds\ dr{\isacharsemicolon}\ Med\ {\isacharparenleft}fproj{\isadigit{2}}{\isasymcdot}dr{\isacharparenright}\ as{\isasymrbrakk}\ {\isasymLongrightarrow}\ {\isacharhash}{\isacharparenleft}fnub{\isasymcdot}ds{\isacharparenright}\ {\isacharequal}\ {\isacharhash}{\isacharparenleft}fnub{\isasymcdot}as{\isacharparenright}{\isachardoublequoteclose}\isanewline
%
\isadelimproof
%
\endisadelimproof
%
\isatagproof
\isacommand{apply}\isamarkupfalse%
\ {\isacharparenleft}case{\isacharunderscore}tac\ {\isachardoublequoteopen}{\isacharhash}{\isacharparenleft}fnub{\isasymcdot}as{\isacharparenright}\ {\isacharless}\ {\isacharhash}i{\isachardoublequoteclose}{\isacharparenright}\isanewline
\isacommand{apply}\isamarkupfalse%
\ {\isacharparenleft}case{\isacharunderscore}tac\ {\isachardoublequoteopen}fnub{\isasymcdot}as\ {\isacharequal}\ {\isasymepsilon}{\isachardoublequoteclose}{\isacharcomma}\ auto{\isacharparenright}\isanewline
\isacommand{apply}\isamarkupfalse%
\ {\isacharparenleft}drule\ strict{\isacharunderscore}rev{\isacharunderscore}fnub\ {\isacharbrackleft}rule{\isacharunderscore}format{\isacharbrackright}{\isacharparenright}\isanewline
\isacommand{apply}\isamarkupfalse%
\ {\isacharparenleft}simp\ add{\isacharcolon}\ Snd{\isacharunderscore}def\ Let{\isacharunderscore}def{\isacharcomma}\ auto{\isacharparenright}\isanewline
\isacommand{apply}\isamarkupfalse%
\ {\isacharparenleft}simp\ add{\isacharcolon}\ inat{\isacharunderscore}defs\ split{\isacharcolon}\ inat{\isacharunderscore}splits{\isacharparenright}\isanewline
\isacommand{apply}\isamarkupfalse%
\ {\isacharparenleft}drule\ fair{\isacharunderscore}Med{\isacharcomma}\ auto{\isacharparenright}\isanewline
\isacommand{apply}\isamarkupfalse%
\ {\isacharparenleft}simp\ add{\isacharcolon}\ fproj{\isadigit{2}}{\isacharunderscore}fslen\ {\isacharbrackleft}THEN\ sym{\isacharbrackright}{\isacharparenright}\isanewline
\isacommand{apply}\isamarkupfalse%
\ {\isacharparenleft}drule\ fair{\isacharunderscore}Med{\isacharcomma}\ auto{\isacharparenright}\isanewline
\isacommand{apply}\isamarkupfalse%
\ {\isacharparenleft}case{\isacharunderscore}tac\ {\isachardoublequoteopen}{\isacharhash}{\isacharparenleft}fnub{\isasymcdot}as{\isacharparenright}{\isachardoublequoteclose}{\isacharcomma}\ auto{\isacharparenright}\isanewline
\isacommand{apply}\isamarkupfalse%
\ {\isacharparenleft}case{\isacharunderscore}tac\ {\isachardoublequoteopen}nat{\isachardoublequoteclose}{\isacharcomma}\ auto{\isacharparenright}\isanewline
\isacommand{apply}\isamarkupfalse%
\ {\isacharparenleft}simp\ add{\isacharcolon}\ Fin{\isacharunderscore}{\isadigit{0}}{\isacharparenright}\isanewline
\isacommand{apply}\isamarkupfalse%
\ {\isacharparenleft}subgoal{\isacharunderscore}tac\ {\isachardoublequoteopen}{\isacharhash}ds\ {\isacharequal}\ {\isasyminfinity}{\isachardoublequoteclose}{\isacharparenright}\isanewline
\isacommand{apply}\isamarkupfalse%
\ {\isacharparenleft}frule\ abp{\isacharunderscore}one{\isacharunderscore}Med{\isacharcomma}\ auto{\isacharparenright}\isanewline
\isacommand{apply}\isamarkupfalse%
\ {\isacharparenleft}simp\ add{\isacharcolon}\ fproj{\isadigit{2}}{\isacharunderscore}fslen\ {\isacharbrackleft}THEN\ sym{\isacharbrackright}{\isacharparenright}\isanewline
\isacommand{apply}\isamarkupfalse%
\ {\isacharparenleft}subgoal{\isacharunderscore}tac\ {\isachardoublequoteopen}ftake\ {\isacharparenleft}Suc\ nata{\isacharparenright}{\isasymcdot}{\isacharparenleft}fnub{\isasymcdot}{\isacharparenleft}fproj{\isadigit{2}}{\isasymcdot}ds{\isacharparenright}{\isacharparenright}\ {\isacharequal}\ fnub{\isasymcdot}as{\isachardoublequoteclose}{\isacharparenright}\isanewline
\isacommand{apply}\isamarkupfalse%
\ {\isacharparenleft}simp\ add{\isacharcolon}\ alt{\isacharunderscore}Snd{\isacharunderscore}lemma{\isacharparenright}\isanewline
\isacommand{apply}\isamarkupfalse%
\ {\isacharparenleft}subgoal{\isacharunderscore}tac\ {\isachardoublequoteopen}{\isacharhash}{\isacharparenleft}fnub{\isasymcdot}{\isacharparenleft}fproj{\isadigit{2}}{\isasymcdot}ds{\isacharparenright}{\isacharparenright}\ {\isasymle}\ Fin\ {\isacharparenleft}Suc\ {\isacharparenleft}Suc\ nata{\isacharparenright}{\isacharparenright}{\isachardoublequoteclose}{\isacharparenright}\isanewline
\isacommand{apply}\isamarkupfalse%
\ {\isacharparenleft}subgoal{\isacharunderscore}tac\ {\isachardoublequoteopen}{\isacharhash}fnub{\isasymcdot}{\isacharparenleft}fproj{\isadigit{2}}{\isasymcdot}ds{\isacharparenright}\ {\isacharequal}\ {\isacharhash}{\isacharparenleft}fnub{\isasymcdot}as{\isacharparenright}{\isachardoublequoteclose}{\isacharcomma}\ simp{\isacharparenright}\isanewline
\isacommand{apply}\isamarkupfalse%
\ {\isacharparenleft}rule\ Med{\isacharunderscore}trans{\isacharunderscore}lemma\ \isanewline
\ \ \ \ \ \ \ \ \ {\isacharbrackleft}rule{\isacharunderscore}format{\isacharcomma}\ of\ {\isachardoublequoteopen}fproj{\isadigit{2}}{\isasymcdot}ds{\isachardoublequoteclose}\ {\isachardoublequoteopen}as{\isachardoublequoteclose}{\isacharbrackright}{\isacharcomma}\ auto{\isacharparenright}\ \isacommand{defer}\isamarkupfalse%
\ {\isadigit{1}}\isanewline
\isacommand{apply}\isamarkupfalse%
\ {\isacharparenleft}simp\ add{\isacharcolon}\ Snd{\isacharunderscore}def\ Let{\isacharunderscore}def{\isacharparenright}\isanewline
\isacommand{apply}\isamarkupfalse%
\ {\isacharparenleft}simp\ add{\isacharcolon}\ Snd{\isacharunderscore}def\ Let{\isacharunderscore}def{\isacharparenright}\ \isanewline
\isacommand{apply}\isamarkupfalse%
\ {\isacharparenleft}frule\ ack{\isacharunderscore}Snd{\isacharunderscore}lemma{\isacharcomma}\ auto{\isacharparenright}\isanewline
\isacommand{apply}\isamarkupfalse%
\ {\isacharparenleft}drule\ Snd{\isacharunderscore}fslen{\isacharunderscore}lemma{\isacharcomma}\ auto{\isacharparenright}\ \isanewline
\isacommand{apply}\isamarkupfalse%
\ {\isacharparenleft}simp\ add{\isacharcolon}\ inat{\isacharunderscore}defs\ split{\isacharcolon}\ inat{\isacharunderscore}splits{\isacharparenright}\ \isacommand{defer}\isamarkupfalse%
\ {\isadigit{1}}\isanewline
\isacommand{apply}\isamarkupfalse%
\ {\isacharparenleft}simp\ add{\isacharcolon}\ Snd{\isacharunderscore}def\ Let{\isacharunderscore}def{\isacharparenright}\isanewline
\isacommand{apply}\isamarkupfalse%
\ {\isacharparenleft}simp\ add{\isacharcolon}\ fproj{\isadigit{1}}{\isacharunderscore}fslen\ fproj{\isadigit{2}}{\isacharunderscore}fslen{\isacharparenright}\isanewline
\isacommand{apply}\isamarkupfalse%
\ {\isacharparenleft}simp\ add{\isacharcolon}\ inat{\isacharunderscore}defs\ split{\isacharcolon}\ inat{\isacharunderscore}splits{\isacharcomma}\ arith{\isacharquery}{\isacharparenright}\isanewline
\isacommand{apply}\isamarkupfalse%
\ {\isacharparenleft}frule\ as{\isacharunderscore}less{\isacharunderscore}i{\isacharcomma}\ auto{\isacharparenright}\isanewline
\isacommand{apply}\isamarkupfalse%
\ {\isacharparenleft}simp\ add{\isacharcolon}\ inat{\isacharunderscore}defs\ split{\isacharcolon}\ inat{\isacharunderscore}splits{\isacharparenright}\isanewline
\isacommand{apply}\isamarkupfalse%
\ {\isacharparenleft}simp\ add{\isacharcolon}\ Snd{\isacharunderscore}def\ Let{\isacharunderscore}def{\isacharcomma}\ auto{\isacharparenright}\isanewline
\isacommand{apply}\isamarkupfalse%
\ {\isacharparenleft}simp\ add{\isacharcolon}\ fproj{\isadigit{1}}{\isacharunderscore}fslen{\isacharcomma}\ arith{\isacharparenright}\isanewline
\isacommand{apply}\isamarkupfalse%
\ {\isacharparenleft}drule\ Snd{\isacharunderscore}fslen{\isacharunderscore}lemma{\isacharcomma}\ auto{\isacharparenright}\isanewline
\isacommand{by}\isamarkupfalse%
\ {\isacharparenleft}simp\ add{\isacharcolon}\ inat{\isacharunderscore}defs\ split{\isacharcolon}\ inat{\isacharunderscore}splits{\isacharparenright}%
\endisatagproof
{\isafoldproof}%
%
\isadelimproof
\isanewline
%
\endisadelimproof
\isanewline
\isacommand{lemma}\isamarkupfalse%
\ Snd{\isacharunderscore}inat{\isacharunderscore}lemma{\isadigit{1}}{\isacharcolon}\ \isanewline
\ \ {\isachardoublequoteopen}{\isacharhash}fnub{\isasymcdot}as\ {\isacharequal}\ imin\ {\isacharparenleft}Fin\ k{\isacharparenright}\ {\isacharparenleft}iSuc\ {\isacharhash}fnub{\isasymcdot}as{\isacharparenright}\ {\isasymLongrightarrow}\ {\isacharhash}{\isacharparenleft}fnub{\isasymcdot}as{\isacharparenright}\ {\isacharequal}\ Fin\ k{\isachardoublequoteclose}\isanewline
%
\isadelimproof
%
\endisadelimproof
%
\isatagproof
\isacommand{by}\isamarkupfalse%
\ {\isacharparenleft}auto\ simp\ add{\isacharcolon}\ imin{\isacharunderscore}def\ inat{\isacharunderscore}defs\ split{\isacharcolon}\ inat{\isacharunderscore}splits{\isacharcomma}\ arith{\isacharquery}{\isacharparenright}%
\endisatagproof
{\isafoldproof}%
%
\isadelimproof
\isanewline
%
\endisadelimproof
\isanewline
\isacommand{lemma}\isamarkupfalse%
\ Snd{\isacharunderscore}inat{\isacharunderscore}lemma{\isadigit{2}}{\isacharcolon}\isanewline
\ \ {\isachardoublequoteopen}Snd\ i\ as\ ds\ {\isasymLongrightarrow}\ {\isacharhash}{\isacharparenleft}fnub{\isasymcdot}ds{\isacharparenright}\ {\isacharequal}\ imin\ {\isacharhash}i\ {\isacharparenleft}iSuc\ {\isacharhash}{\isacharparenleft}fnub{\isasymcdot}as{\isacharparenright}{\isacharparenright}{\isachardoublequoteclose}\isanewline
%
\isadelimproof
%
\endisadelimproof
%
\isatagproof
\isacommand{by}\isamarkupfalse%
\ {\isacharparenleft}auto\ simp\ add{\isacharcolon}\ Snd{\isacharunderscore}def\ Let{\isacharunderscore}def\ fproj{\isadigit{1}}{\isacharunderscore}fslen{\isacharparenright}%
\endisatagproof
{\isafoldproof}%
%
\isadelimproof
\isanewline
%
\endisadelimproof
\isanewline
\isacommand{lemma}\isamarkupfalse%
\ ABP{\isacharunderscore}fslen{\isacharunderscore}lemma{\isadigit{3}}{\isacharcolon}\ \isanewline
\ \ {\isachardoublequoteopen}{\isasymlbrakk}Snd\ i\ as\ ds{\isacharsemicolon}\ Med\ ds\ dr{\isacharsemicolon}\ Med\ {\isacharparenleft}fproj{\isadigit{2}}{\isasymcdot}dr{\isacharparenright}\ as{\isasymrbrakk}\ {\isasymLongrightarrow}\ {\isacharhash}{\isacharparenleft}fnub{\isasymcdot}ds{\isacharparenright}\ {\isacharequal}\ {\isacharhash}i{\isachardoublequoteclose}\isanewline
%
\isadelimproof
%
\endisadelimproof
%
\isatagproof
\isacommand{apply}\isamarkupfalse%
\ {\isacharparenleft}frule\ ABP{\isacharunderscore}fslen{\isacharunderscore}lemma{\isadigit{1}}{\isacharcomma}\ assumption{\isacharplus}{\isacharparenright}\isanewline
\isacommand{apply}\isamarkupfalse%
\ {\isacharparenleft}drule\ Snd{\isacharunderscore}inat{\isacharunderscore}lemma{\isadigit{2}}{\isacharcomma}\ auto{\isacharparenright}\isanewline
\isacommand{by}\isamarkupfalse%
\ {\isacharparenleft}simp\ add{\isacharcolon}\ imin{\isacharunderscore}def\ inat{\isacharunderscore}defs\ split{\isacharcolon}\ inat{\isacharunderscore}splits{\isacharcomma}\ arith{\isacharquery}{\isacharparenright}%
\endisatagproof
{\isafoldproof}%
%
\isadelimproof
\isanewline
%
\endisadelimproof
\isanewline
\isacommand{lemma}\isamarkupfalse%
\ ABP{\isacharunderscore}fslen{\isacharunderscore}lemma{\isadigit{2}}{\isacharcolon}\ \isanewline
\ \ {\isachardoublequoteopen}{\isasymlbrakk}Snd\ i\ as\ ds{\isacharsemicolon}\ Med\ ds\ dr{\isacharsemicolon}\ Med\ {\isacharparenleft}fproj{\isadigit{2}}{\isasymcdot}dr{\isacharparenright}\ as{\isasymrbrakk}\ {\isasymLongrightarrow}\ {\isacharhash}{\isacharparenleft}fnub{\isasymcdot}ds{\isacharparenright}\ {\isacharequal}\ {\isacharhash}{\isacharparenleft}fnub{\isasymcdot}dr{\isacharparenright}{\isachardoublequoteclose}\isanewline
%
\isadelimproof
%
\endisadelimproof
%
\isatagproof
\isacommand{apply}\isamarkupfalse%
\ {\isacharparenleft}frule\ ABP{\isacharunderscore}fslen{\isacharunderscore}lemma{\isadigit{1}}{\isacharcomma}\ assumption{\isacharplus}{\isacharparenright}\isanewline
\isacommand{apply}\isamarkupfalse%
\ {\isacharparenleft}drule\ fnub{\isacharunderscore}less{\isacharunderscore}Med{\isacharparenright}{\isacharplus}\isanewline
\isacommand{apply}\isamarkupfalse%
\ {\isacharparenleft}insert\ fslen{\isacharunderscore}fnub{\isacharunderscore}fproj{\isadigit{2}}{\isacharunderscore}mono\ {\isacharbrackleft}of\ dr{\isacharbrackright}{\isacharparenright}\isanewline
\isacommand{by}\isamarkupfalse%
\ {\isacharparenleft}auto\ simp\ add{\isacharcolon}\ inat{\isacharunderscore}defs\ split{\isacharcolon}\ inat{\isacharunderscore}splits{\isacharparenright}%
\endisatagproof
{\isafoldproof}%
%
\isadelimproof
\isanewline
%
\endisadelimproof
\isanewline
\isacommand{lemma}\isamarkupfalse%
\ ABP{\isacharunderscore}fin{\isacharunderscore}correct{\isacharunderscore}lemma{\isacharcolon}\ \isanewline
\ \ {\isachardoublequoteopen}{\isasymlbrakk}Snd\ i\ as\ ds{\isacharsemicolon}\ Med\ ds\ dr{\isacharsemicolon}\ Rcv\ dr\ ar\ out{\isacharsemicolon}\ Med\ ar\ as{\isacharsemicolon}\ {\isacharhash}i\ {\isacharequal}\ Fin\ k{\isasymrbrakk}\ {\isasymLongrightarrow}\ out\ {\isacharequal}\ fproj{\isadigit{1}}{\isasymcdot}{\isacharparenleft}fnub{\isasymcdot}ds{\isacharparenright}{\isachardoublequoteclose}\isanewline
%
\isadelimproof
%
\endisadelimproof
%
\isatagproof
\isacommand{apply}\isamarkupfalse%
\ {\isacharparenleft}auto\ simp\ add{\isacharcolon}\ Rcv{\isacharunderscore}def{\isacharparenright}\isanewline
\isacommand{apply}\isamarkupfalse%
\ {\isacharparenleft}frule\ ABP{\isacharunderscore}fslen{\isacharunderscore}lemma{\isadigit{2}}{\isacharcomma}\ assumption{\isacharplus}{\isacharparenright}\isanewline
\isacommand{apply}\isamarkupfalse%
\ {\isacharparenleft}frule\ ABP{\isacharunderscore}fslen{\isacharunderscore}lemma{\isadigit{3}}{\isacharcomma}\ assumption{\isacharplus}{\isacharparenright}\isanewline
\isacommand{apply}\isamarkupfalse%
\ {\isacharparenleft}rule\ cfun{\isacharunderscore}arg{\isacharunderscore}cong{\isacharparenright}\isanewline
\isacommand{by}\isamarkupfalse%
\ {\isacharparenleft}insert\ fnub{\isacharunderscore}eq{\isacharunderscore}Med\ {\isacharbrackleft}rule{\isacharunderscore}format{\isacharcomma}\ of\ ds\ dr\ k{\isacharbrackright}{\isacharcomma}\ auto{\isacharparenright}%
\endisatagproof
{\isafoldproof}%
%
\isadelimproof
\isanewline
%
\endisadelimproof
\isanewline
\isacommand{lemma}\isamarkupfalse%
\ ABP{\isacharunderscore}fin{\isacharunderscore}correct{\isacharcolon}\ \isanewline
\ \ {\isachardoublequoteopen}{\isasymlbrakk}{\isacharhash}i\ {\isacharequal}\ Fin\ k{\isacharsemicolon}\ Snd\ i\ as\ ds{\isacharsemicolon}\ Med\ ds\ dr{\isacharsemicolon}\ Rcv\ dr\ ar\ out{\isacharsemicolon}\ Med\ ar\ as{\isasymrbrakk}\ {\isasymLongrightarrow}\ out\ {\isacharequal}\ i{\isachardoublequoteclose}\isanewline
%
\isadelimproof
%
\endisadelimproof
%
\isatagproof
\isacommand{apply}\isamarkupfalse%
\ {\isacharparenleft}frule\ ABP{\isacharunderscore}fin{\isacharunderscore}correct{\isacharunderscore}lemma{\isacharcomma}\ assumption{\isacharplus}{\isacharparenright}\isanewline
\isacommand{apply}\isamarkupfalse%
\ {\isacharparenleft}simp\ add{\isacharcolon}\ Rcv{\isacharunderscore}def{\isacharparenright}\isanewline
\isacommand{apply}\isamarkupfalse%
\ {\isacharparenleft}frule\ ABP{\isacharunderscore}fslen{\isacharunderscore}lemma{\isadigit{3}}{\isacharcomma}\ assumption{\isacharplus}{\isacharparenright}\isanewline
\isacommand{apply}\isamarkupfalse%
\ {\isacharparenleft}drule\ SndD{\isadigit{1}}{\isacharcomma}\ auto{\isacharparenright}\isanewline
\isacommand{apply}\isamarkupfalse%
\ {\isacharparenleft}rule\ size{\isacharunderscore}eq{\isacharcomma}\ auto{\isacharparenright}\isanewline
\isacommand{by}\isamarkupfalse%
\ {\isacharparenleft}simp\ add{\isacharcolon}\ fproj{\isadigit{1}}{\isacharunderscore}fslen\ {\isacharbrackleft}THEN\ sym{\isacharbrackright}{\isacharparenright}%
\endisatagproof
{\isafoldproof}%
%
\isadelimproof
\isanewline
%
\endisadelimproof
%
\isadelimtheory
\isanewline
%
\endisadelimtheory
%
\isatagtheory
\isacommand{end}\isamarkupfalse%
%
\endisatagtheory
{\isafoldtheory}%
%
\isadelimtheory
\isanewline
%
\endisadelimtheory
\isanewline
\isanewline
\isanewline
\end{isabellebody}%
%%% Local Variables:
%%% mode: latex
%%% TeX-master: "root"
%%% End:
