# Supplementary material for: ALICE: An Advanced Logic for Interactive Component Engineering
Source: arXiv:1410.4381 source file (2014-10-16)
Supplement: Supplementary file 5 [file Receiver.tex]

%
\begin{isabellebody}%
\def\isabellecontext{Receiver}%
%
\isadelimtheory
%
\endisadelimtheory
%
\isatagtheory
\isacommand{theory}\isamarkupfalse%
\ Receiver\isanewline
\isakeyword{imports}\ ABPTypes\isanewline
\isakeyword{begin}%
\endisatagtheory
{\isafoldtheory}%
%
\isadelimtheory
\isanewline
%
\endisadelimtheory
\isanewline
\isacommand{constdefs}\isamarkupfalse%
\isanewline
\ \ Rcv\ {\isacharcolon}{\isacharcolon}\ {\isachardoublequoteopen}{\isacharparenleft}Data\ {\isacharasterisk}\ Bit{\isacharparenright}\ fstream\ {\isasymRightarrow}\ Bit\ fstream\ {\isasymRightarrow}\ Data\ fstream\ {\isasymRightarrow}\ bool{\isachardoublequoteclose}\isanewline
\ \ Rcv{\isacharunderscore}def{\isacharcolon}\ \isanewline
\ \ \ \ {\isachardoublequoteopen}Rcv\ dr\ ar\ out\ {\isasymequiv}\ \isanewline
\ \ \ \ \ \ \ ar\ {\isacharequal}\ fproj{\isadigit{2}}{\isasymcdot}dr\ {\isasymand}\ \isanewline
\ \ \ \ \ \ \ out\ {\isacharequal}\ fproj{\isadigit{1}}{\isasymcdot}{\isacharparenleft}fnub{\isasymcdot}dr{\isacharparenright}{\isachardoublequoteclose}\isanewline
%
\isadelimtheory
\isanewline
%
\endisadelimtheory
%
\isatagtheory
\isacommand{end}\isamarkupfalse%
%
\endisatagtheory
{\isafoldtheory}%
%
\isadelimtheory
\isanewline
%
\endisadelimtheory
\end{isabellebody}%
%%% Local Variables:
%%% mode: latex
%%% TeX-master: "root"
%%% End:
