# Supplementary material for: ALICE: An Advanced Logic for Interactive Component Engineering
Source: arXiv:1410.4381 source file (2014-10-16)
Supplement: Supplementary file 6 [file Sender.tex]

%
\begin{isabellebody}%
\def\isabellecontext{Sender}%
%
\isadelimtheory
%
\endisadelimtheory
%
\isatagtheory
\isacommand{theory}\isamarkupfalse%
\ Sender\isanewline
\isakeyword{imports}\ ABPTypes\isanewline
\isakeyword{begin}%
\endisatagtheory
{\isafoldtheory}%
%
\isadelimtheory
\isanewline
%
\endisadelimtheory
\isanewline
\isacommand{constdefs}\isamarkupfalse%
\isanewline
\ \ Snd\ {\isacharcolon}{\isacharcolon}\ {\isachardoublequoteopen}Data\ fstream\ {\isasymRightarrow}\ Bit\ fstream\ {\isasymRightarrow}\ {\isacharparenleft}Data\ {\isacharasterisk}\ Bit{\isacharparenright}\ fstream\ {\isasymRightarrow}\ bool{\isachardoublequoteclose}\isanewline
\ \ Snd{\isacharunderscore}def{\isacharcolon}\ \isanewline
\ \ \ \ {\isachardoublequoteopen}Snd\ i\ as\ ds\ {\isasymequiv}\ \isanewline
\ \ \ \ \ \ \ let\ \isanewline
\ \ \ \ \ \ \ \ \ \ fas\ {\isacharequal}\ fnub{\isasymcdot}as{\isacharsemicolon}\ \isanewline
\ \ \ \ \ \ \ \ \ \ fb\ {\isacharequal}\ fproj{\isadigit{2}}{\isasymcdot}{\isacharparenleft}fnub{\isasymcdot}ds{\isacharparenright}{\isacharsemicolon}\isanewline
\ \ \ \ \ \ \ \ \ \ fds\ {\isacharequal}\ fproj{\isadigit{1}}{\isasymcdot}{\isacharparenleft}fnub{\isasymcdot}ds{\isacharparenright}\ \isanewline
\ \ \ \ \ \ \ in\ \isanewline
\ \ \ \ \ \ \ \ \ \ fds\ {\isasymsqsubseteq}\ i\ {\isasymand}\ \ \isanewline
\ \ \ \ \ \ \ \ \ \ fnub{\isasymcdot}fb\ {\isacharequal}\ fb\ {\isasymand}\ \ \isanewline
\ \ \ \ \ \ \ \ \ \ {\isacharhash}fds\ {\isacharequal}\ imin\ {\isacharhash}i\ {\isacharparenleft}iSuc\ {\isacharparenleft}{\isacharhash}fas{\isacharparenright}{\isacharparenright}\ {\isasymand}\ \isanewline
\ \ \ \ \ \ \ \ \ \ {\isacharparenleft}{\isacharhash}fas\ {\isacharless}\ {\isacharhash}i\ {\isasymlongrightarrow}\ \isanewline
\ \ \ \ \ \ \ \ \ \ \ \ \ \ \ \ \ \ \ \ \ \ {\isacharhash}ds\ {\isacharequal}\ {\isasyminfinity}\ {\isasymand}\ \isanewline
\ \ \ \ \ \ \ \ \ \ \ \ \ \ \ \ \ \ \ \ \ \ {\isacharparenleft}ftake\ {\isacharparenleft}THE\ k{\isachardot}\ {\isacharhash}{\isacharparenleft}fnub{\isasymcdot}as{\isacharparenright}\ {\isacharequal}\ Fin\ k{\isacharparenright}{\isasymcdot}fb\ {\isacharequal}\ fas{\isacharparenright}{\isacharparenright}{\isachardoublequoteclose}\isanewline
\isanewline
\isacommand{lemma}\isamarkupfalse%
\ SndD{\isadigit{1}}{\isacharcolon}\ \isanewline
\ \ {\isachardoublequoteopen}Snd\ i\ as\ ds\ {\isasymLongrightarrow}\ fproj{\isadigit{1}}{\isasymcdot}{\isacharparenleft}fnub{\isasymcdot}ds{\isacharparenright}\ {\isasymsqsubseteq}\ i{\isachardoublequoteclose}\isanewline
%
\isadelimproof
%
\endisadelimproof
%
\isatagproof
\isacommand{by}\isamarkupfalse%
\ {\isacharparenleft}simp\ add{\isacharcolon}\ Snd{\isacharunderscore}def\ Let{\isacharunderscore}def{\isacharparenright}%
\endisatagproof
{\isafoldproof}%
%
\isadelimproof
\isanewline
%
\endisadelimproof
\isanewline
\isacommand{lemma}\isamarkupfalse%
\ SndD{\isadigit{2}}{\isacharcolon}\ \isanewline
\ \ {\isachardoublequoteopen}Snd\ i\ as\ ds\ {\isasymLongrightarrow}\ {\isacharhash}{\isacharparenleft}fproj{\isadigit{1}}{\isasymcdot}{\isacharparenleft}fnub{\isasymcdot}ds{\isacharparenright}{\isacharparenright}\ {\isacharequal}\ imin\ {\isacharhash}i\ {\isacharparenleft}iSuc\ {\isacharhash}{\isacharparenleft}fnub{\isasymcdot}as{\isacharparenright}{\isacharparenright}{\isachardoublequoteclose}\isanewline
%
\isadelimproof
%
\endisadelimproof
%
\isatagproof
\isacommand{by}\isamarkupfalse%
\ {\isacharparenleft}simp\ add{\isacharcolon}\ Snd{\isacharunderscore}def\ Let{\isacharunderscore}def{\isacharparenright}%
\endisatagproof
{\isafoldproof}%
%
\isadelimproof
\isanewline
%
\endisadelimproof
\isanewline
\isacommand{lemma}\isamarkupfalse%
\ Snd{\isacharunderscore}epsilon{\isacharunderscore}all{\isacharbrackleft}simp{\isacharbrackright}{\isacharcolon}\ \isanewline
\ \ {\isachardoublequoteopen}Snd\ {\isasymepsilon}\ {\isasymepsilon}\ {\isasymepsilon}{\isachardoublequoteclose}\isanewline
%
\isadelimproof
%
\endisadelimproof
%
\isatagproof
\isacommand{by}\isamarkupfalse%
\ {\isacharparenleft}auto\ simp\ add{\isacharcolon}\ Snd{\isacharunderscore}def\ Let{\isacharunderscore}def{\isacharparenright}%
\endisatagproof
{\isafoldproof}%
%
\isadelimproof
\isanewline
%
\endisadelimproof
\isanewline
\isacommand{lemma}\isamarkupfalse%
\ mixed{\isacharunderscore}fnub{\isacharunderscore}fproj{\isadigit{2}}{\isacharbrackleft}simp{\isacharbrackright}{\isacharcolon}\ \isanewline
\ \ {\isachardoublequoteopen}fnub{\isasymcdot}{\isacharparenleft}fproj{\isadigit{2}}{\isasymcdot}{\isacharparenleft}fnub{\isasymcdot}x{\isacharparenright}{\isacharparenright}\ {\isacharequal}\ fnub{\isasymcdot}{\isacharparenleft}fproj{\isadigit{2}}{\isasymcdot}x{\isacharparenright}{\isachardoublequoteclose}\isanewline
%
\isadelimproof
%
\endisadelimproof
%
\isatagproof
\isacommand{apply}\isamarkupfalse%
\ {\isacharparenleft}rule\ fstream{\isacharunderscore}ind{\isadigit{1}}\ {\isacharbrackleft}of\ {\isacharunderscore}\ {\isachardoublequoteopen}x{\isachardoublequoteclose}{\isacharbrackright}{\isacharcomma}\ auto{\isacharparenright}\isanewline
\isacommand{apply}\isamarkupfalse%
\ {\isacharparenleft}case{\isacharunderscore}tac\ {\isachardoublequoteopen}s\ {\isacharequal}\ {\isasymepsilon}{\isachardoublequoteclose}{\isacharcomma}\ auto{\isacharparenright}\isanewline
\isacommand{apply}\isamarkupfalse%
\ {\isacharparenleft}drule\ fscase{\isadigit{2}}{\isacharcomma}\ auto{\isacharparenright}\isanewline
\isacommand{apply}\isamarkupfalse%
\ {\isacharparenleft}case{\isacharunderscore}tac\ {\isachardoublequoteopen}{\isacharparenleft}a{\isacharcomma}b{\isacharparenright}\ {\isacharequal}\ {\isacharparenleft}aa{\isacharcomma}ba{\isacharparenright}{\isachardoublequoteclose}{\isacharcomma}\ auto{\isacharparenright}\isanewline
\isacommand{apply}\isamarkupfalse%
\ {\isacharparenleft}insert\ fnub{\isacharunderscore}exhaust{\isacharcomma}\ atomize{\isacharparenright}\isanewline
\isacommand{apply}\isamarkupfalse%
\ {\isacharparenleft}erule{\isacharunderscore}tac\ x{\isacharequal}{\isachardoublequoteopen}{\isacharparenleft}aa{\isacharcomma}ba{\isacharparenright}{\isachardoublequoteclose}\isakeyword{in}\ allE{\isacharparenright}\isanewline
\isacommand{apply}\isamarkupfalse%
\ {\isacharparenleft}erule{\isacharunderscore}tac\ x{\isacharequal}{\isachardoublequoteopen}rs{\isachardoublequoteclose}\ \isakeyword{in}\ allE{\isacharcomma}\ auto{\isacharparenright}\isanewline
\isacommand{apply}\isamarkupfalse%
\ {\isacharparenleft}case{\isacharunderscore}tac\ {\isachardoublequoteopen}b{\isacharequal}ba{\isachardoublequoteclose}{\isacharcomma}\ auto{\isacharparenright}\isanewline
\isacommand{apply}\isamarkupfalse%
\ atomize\isanewline
\isacommand{apply}\isamarkupfalse%
\ {\isacharparenleft}erule{\isacharunderscore}tac\ x{\isacharequal}{\isachardoublequoteopen}{\isacharparenleft}aa{\isacharcomma}ba{\isacharparenright}{\isachardoublequoteclose}\ \isakeyword{in}\ allE{\isacharparenright}\isanewline
\isacommand{by}\isamarkupfalse%
\ {\isacharparenleft}erule{\isacharunderscore}tac\ x{\isacharequal}{\isachardoublequoteopen}rs{\isachardoublequoteclose}\ \isakeyword{in}\ allE{\isacharcomma}\ auto{\isacharparenright}%
\endisatagproof
{\isafoldproof}%
%
\isadelimproof
\isanewline
%
\endisadelimproof
\isanewline
\isacommand{lemma}\isamarkupfalse%
\ alt{\isacharunderscore}Snd{\isacharunderscore}lemma{\isacharcolon}\ \isanewline
\ \ {\isachardoublequoteopen}Snd\ i\ as\ ds\ {\isasymLongrightarrow}\ fproj{\isadigit{2}}{\isasymcdot}{\isacharparenleft}fnub{\isasymcdot}ds{\isacharparenright}\ {\isacharequal}\ fnub{\isasymcdot}{\isacharparenleft}fproj{\isadigit{2}}{\isasymcdot}ds{\isacharparenright}{\isachardoublequoteclose}\isanewline
%
\isadelimproof
%
\endisadelimproof
%
\isatagproof
\isacommand{by}\isamarkupfalse%
\ {\isacharparenleft}simp\ add{\isacharcolon}\ Snd{\isacharunderscore}def\ Let{\isacharunderscore}def{\isacharparenright}%
\endisatagproof
{\isafoldproof}%
%
\isadelimproof
\isanewline
%
\endisadelimproof
\isanewline
\isacommand{lemma}\isamarkupfalse%
\ send{\isacharunderscore}Snd{\isacharunderscore}lemma{\isacharcolon}\ \isanewline
\ \ {\isachardoublequoteopen}Snd\ i\ as\ ds\ {\isasymLongrightarrow}\ {\isacharhash}{\isacharparenleft}fnub{\isasymcdot}ds{\isacharparenright}\ {\isasymle}\ {\isacharhash}i{\isachardoublequoteclose}\isanewline
%
\isadelimproof
%
\endisadelimproof
%
\isatagproof
\isacommand{apply}\isamarkupfalse%
\ {\isacharparenleft}drule\ SndD{\isadigit{1}}{\isacharcomma}\ drule\ fslen{\isacharunderscore}mono{\isacharparenright}\isanewline
\isacommand{by}\isamarkupfalse%
\ {\isacharparenleft}simp\ add{\isacharcolon}\ fproj{\isadigit{1}}{\isacharunderscore}fslen{\isacharparenright}%
\endisatagproof
{\isafoldproof}%
%
\isadelimproof
\isanewline
%
\endisadelimproof
\isanewline
\isacommand{lemma}\isamarkupfalse%
\ ack{\isacharunderscore}Snd{\isacharunderscore}lemma{\isacharcolon}\ \isanewline
\ \ {\isachardoublequoteopen}Snd\ i\ as\ ds\ {\isasymLongrightarrow}\ {\isacharparenleft}{\isacharhash}{\isacharparenleft}fnub{\isasymcdot}as{\isacharparenright}\ {\isacharless}\ {\isacharhash}i{\isacharparenright}\ {\isasymor}\ {\isacharparenleft}{\isacharhash}{\isacharparenleft}fnub{\isasymcdot}ds{\isacharparenright}\ {\isacharequal}\ {\isacharhash}i{\isacharparenright}{\isachardoublequoteclose}\isanewline
%
\isadelimproof
%
\endisadelimproof
%
\isatagproof
\isacommand{apply}\isamarkupfalse%
\ {\isacharparenleft}frule\ SndD{\isadigit{2}}{\isacharcomma}\ auto{\isacharparenright}\isanewline
\isacommand{apply}\isamarkupfalse%
\ {\isacharparenleft}drule\ send{\isacharunderscore}Snd{\isacharunderscore}lemma{\isacharparenright}\isanewline
\isacommand{apply}\isamarkupfalse%
\ {\isacharparenleft}simp\ add{\isacharcolon}\ fproj{\isadigit{1}}{\isacharunderscore}fslen{\isacharparenright}\isanewline
\isacommand{by}\isamarkupfalse%
\ {\isacharparenleft}simp\ add{\isacharcolon}\ imin{\isacharunderscore}def\ inat{\isacharunderscore}defs\ split{\isacharcolon}\ inat{\isacharunderscore}splits{\isacharcomma}\ arith{\isacharquery}{\isacharparenright}%
\endisatagproof
{\isafoldproof}%
%
\isadelimproof
\isanewline
%
\endisadelimproof
%
\isadelimtheory
\isanewline
%
\endisadelimtheory
%
\isatagtheory
\isacommand{end}\isamarkupfalse%
%
\endisatagtheory
{\isafoldtheory}%
%
\isadelimtheory
\isanewline
%
\endisadelimtheory
\isanewline
\end{isabellebody}%
%%% Local Variables:
%%% mode: latex
%%% TeX-master: "root"
%%% End:
